# Supplementary material for: Business Process Deviance Mining: Review and Evaluation
Source: arXiv:1608.08252 source file (2016-08-29)
Supplement: Supplementary file 1 [file appendix.tex]

\section{Appendix}\label{sec:Appendix}

\subsection{Schedule Dataset}

\begin{figure}[htb!]
	\centering
	{\includegraphics[scale=0.8] {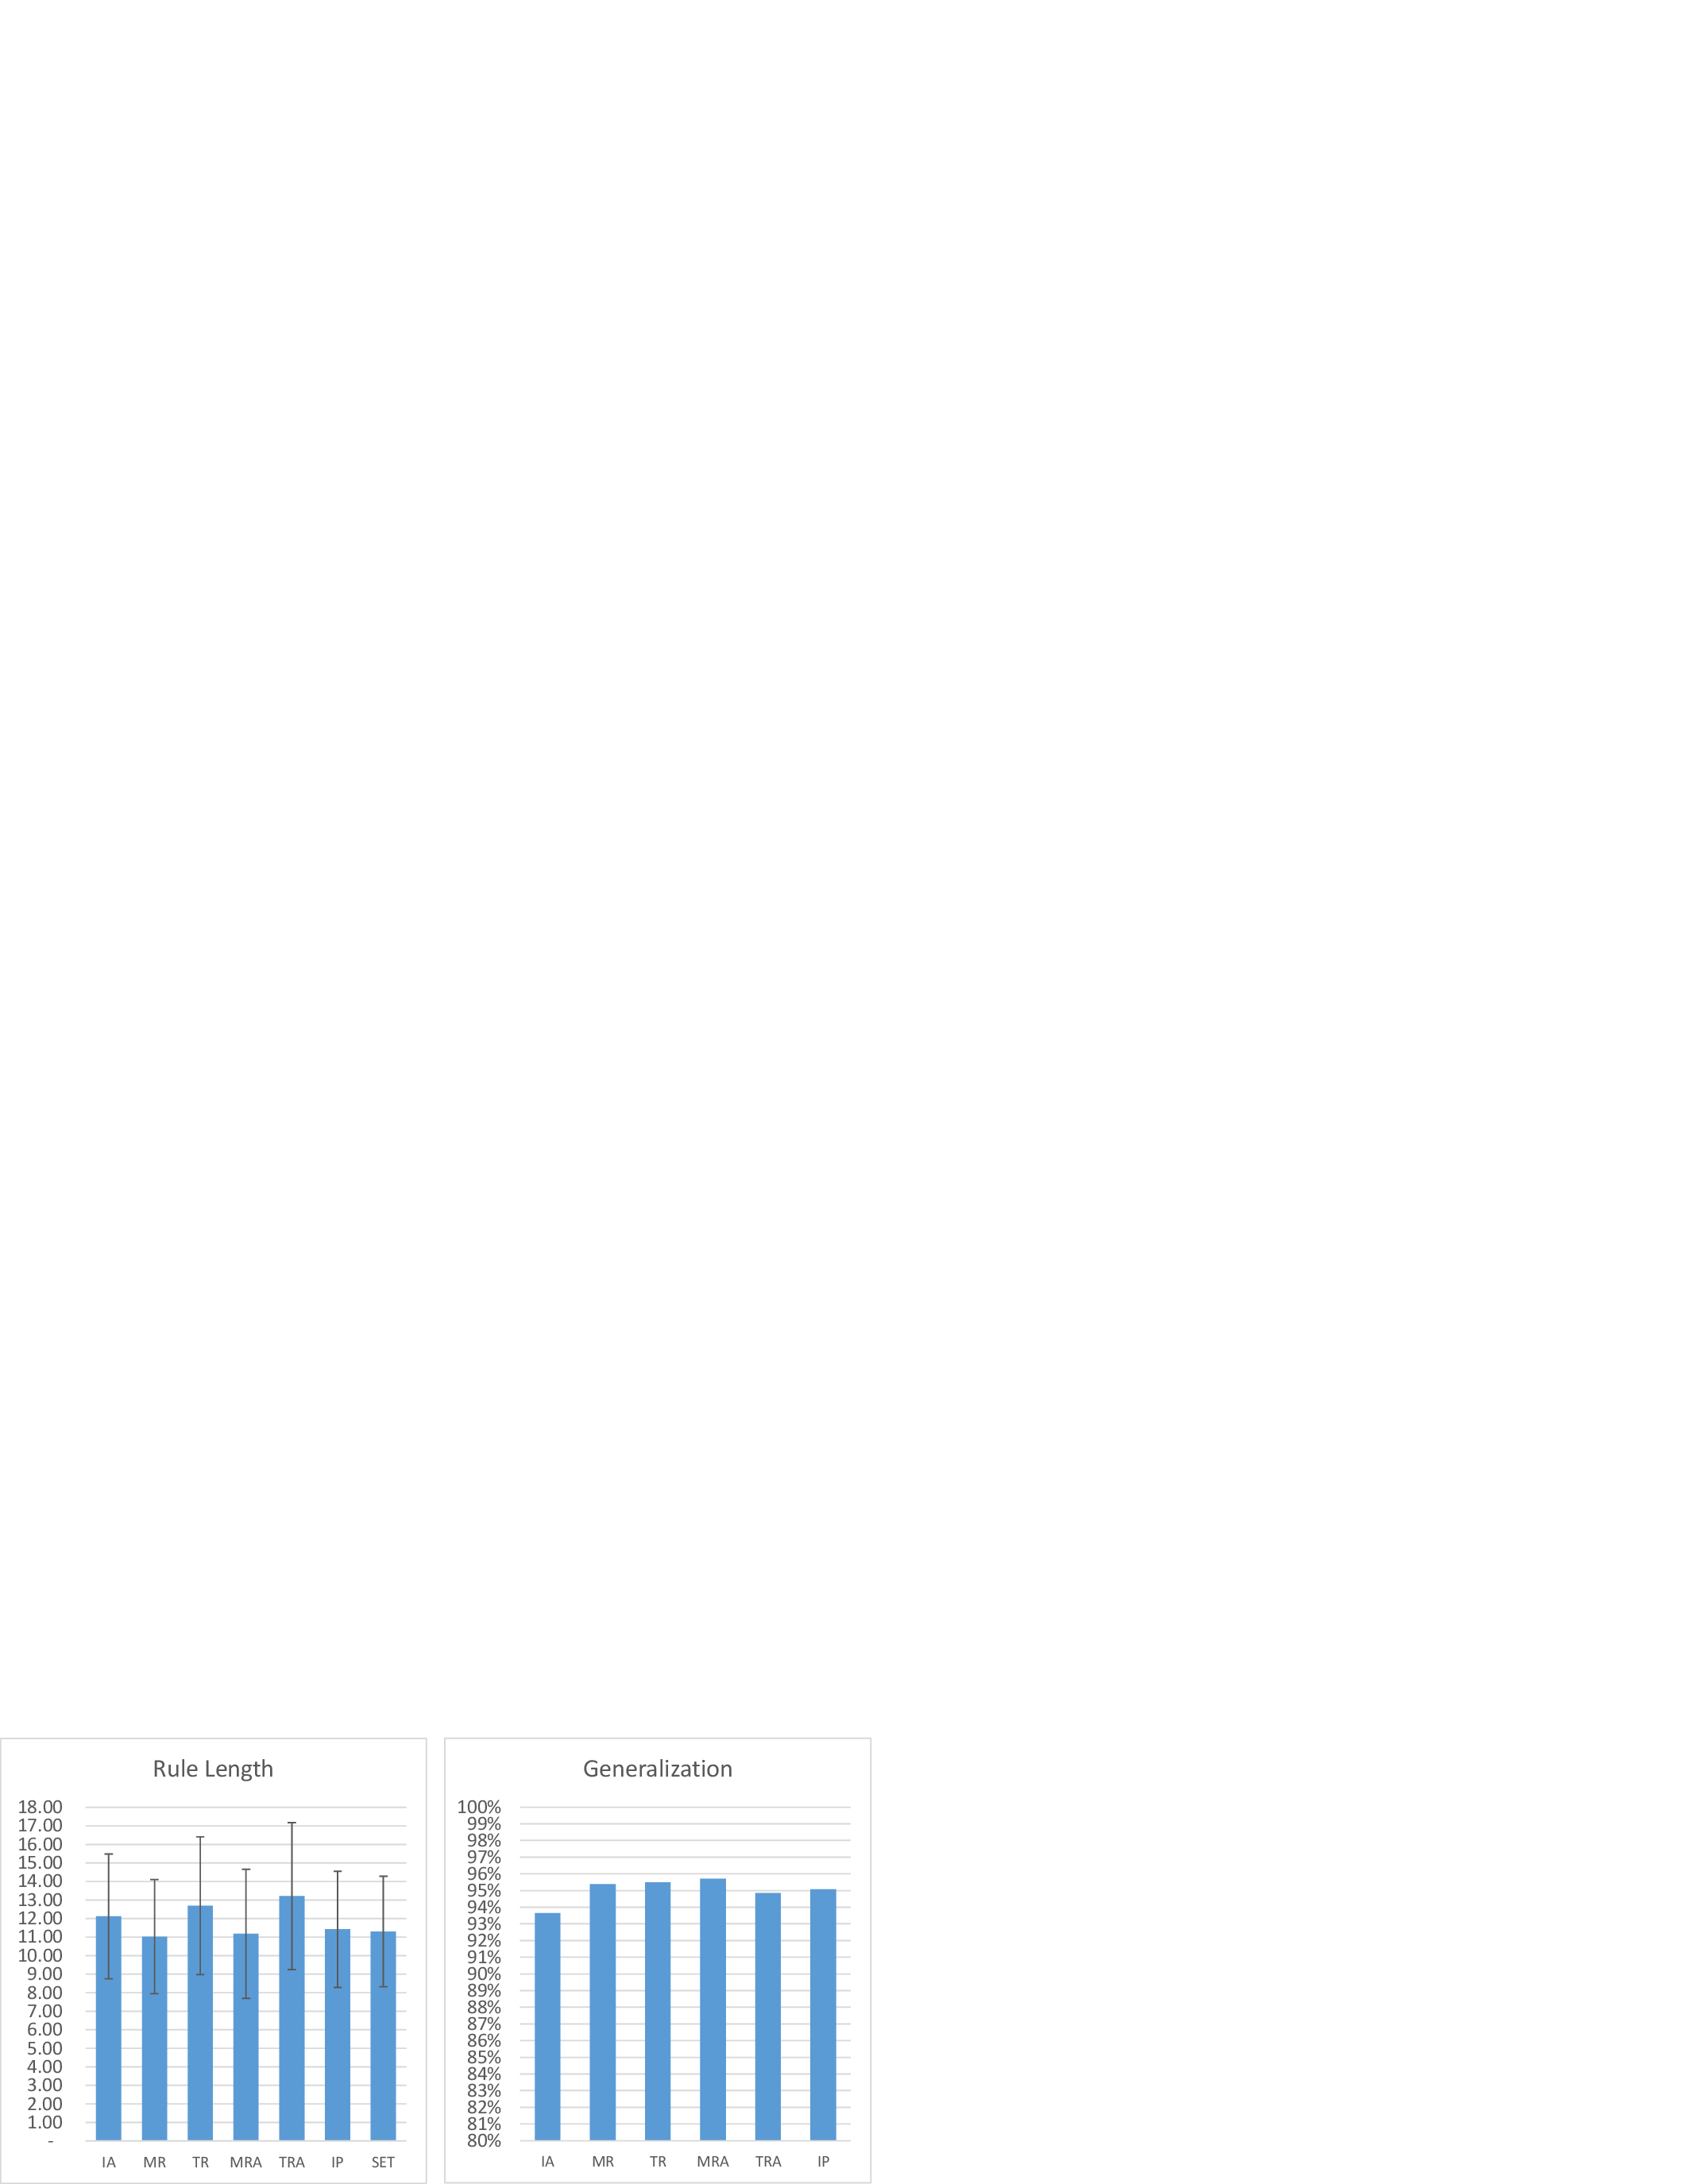}} %{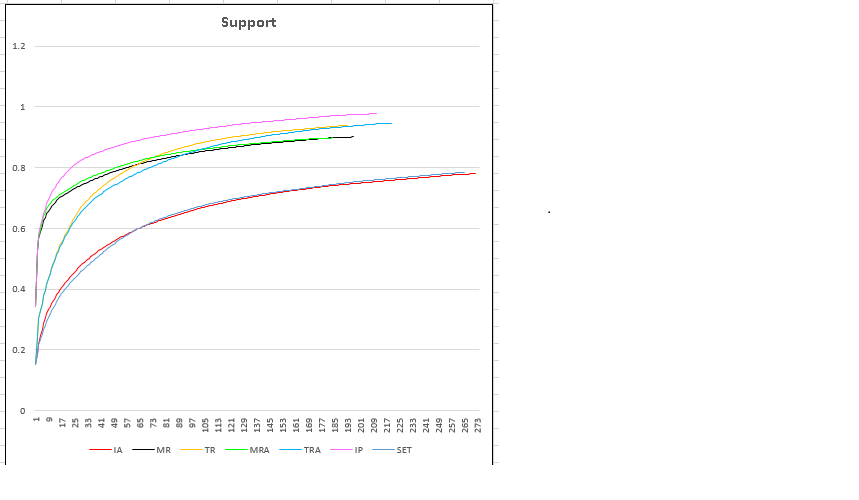}} 
	\caption{Schedule dataset - Rule Length \& \%Generalization}
	\label{fig:schedule-interest5}
\end{figure}	
	
\begin{figure}[htb!]	
	\centering
	{\includegraphics[width=\textwidth]{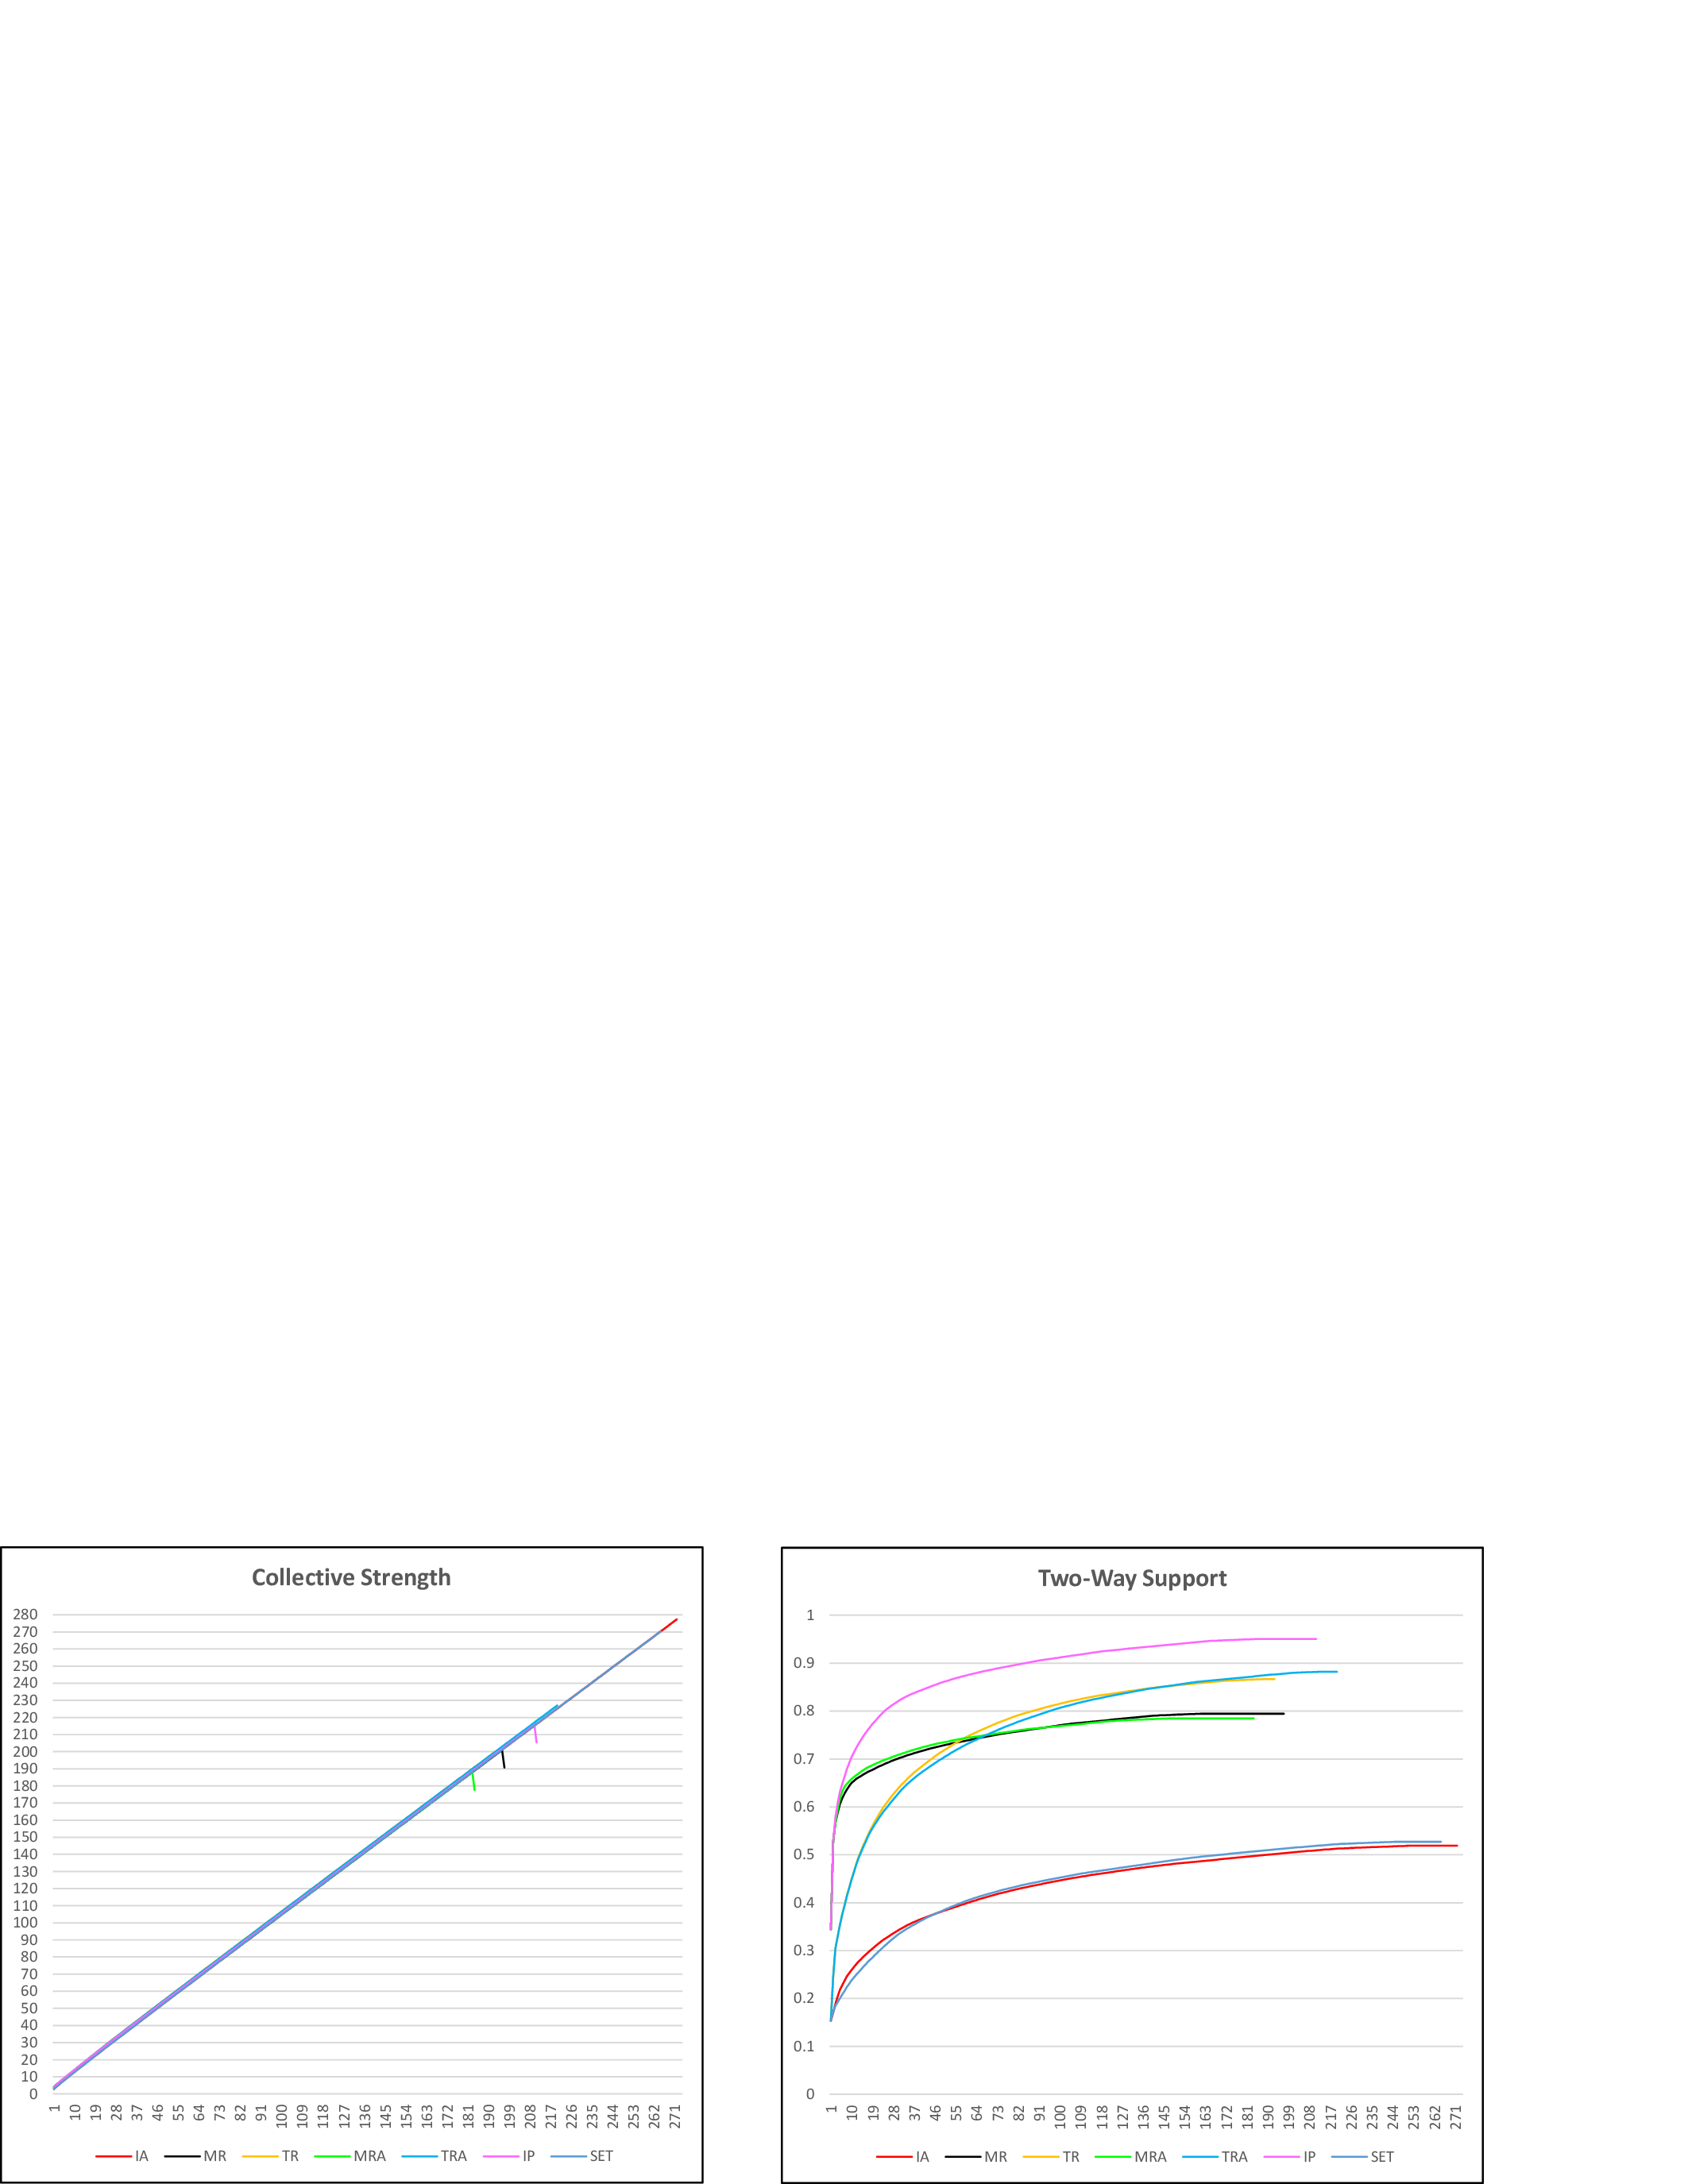}}
	\caption{Schedule dataset - Collective Strength and Two-Way Support}
	\label{fig:schedule-interest2}
\end{figure}

\begin{figure}[htb!]
	\centering
	{\includegraphics[width=\textwidth]{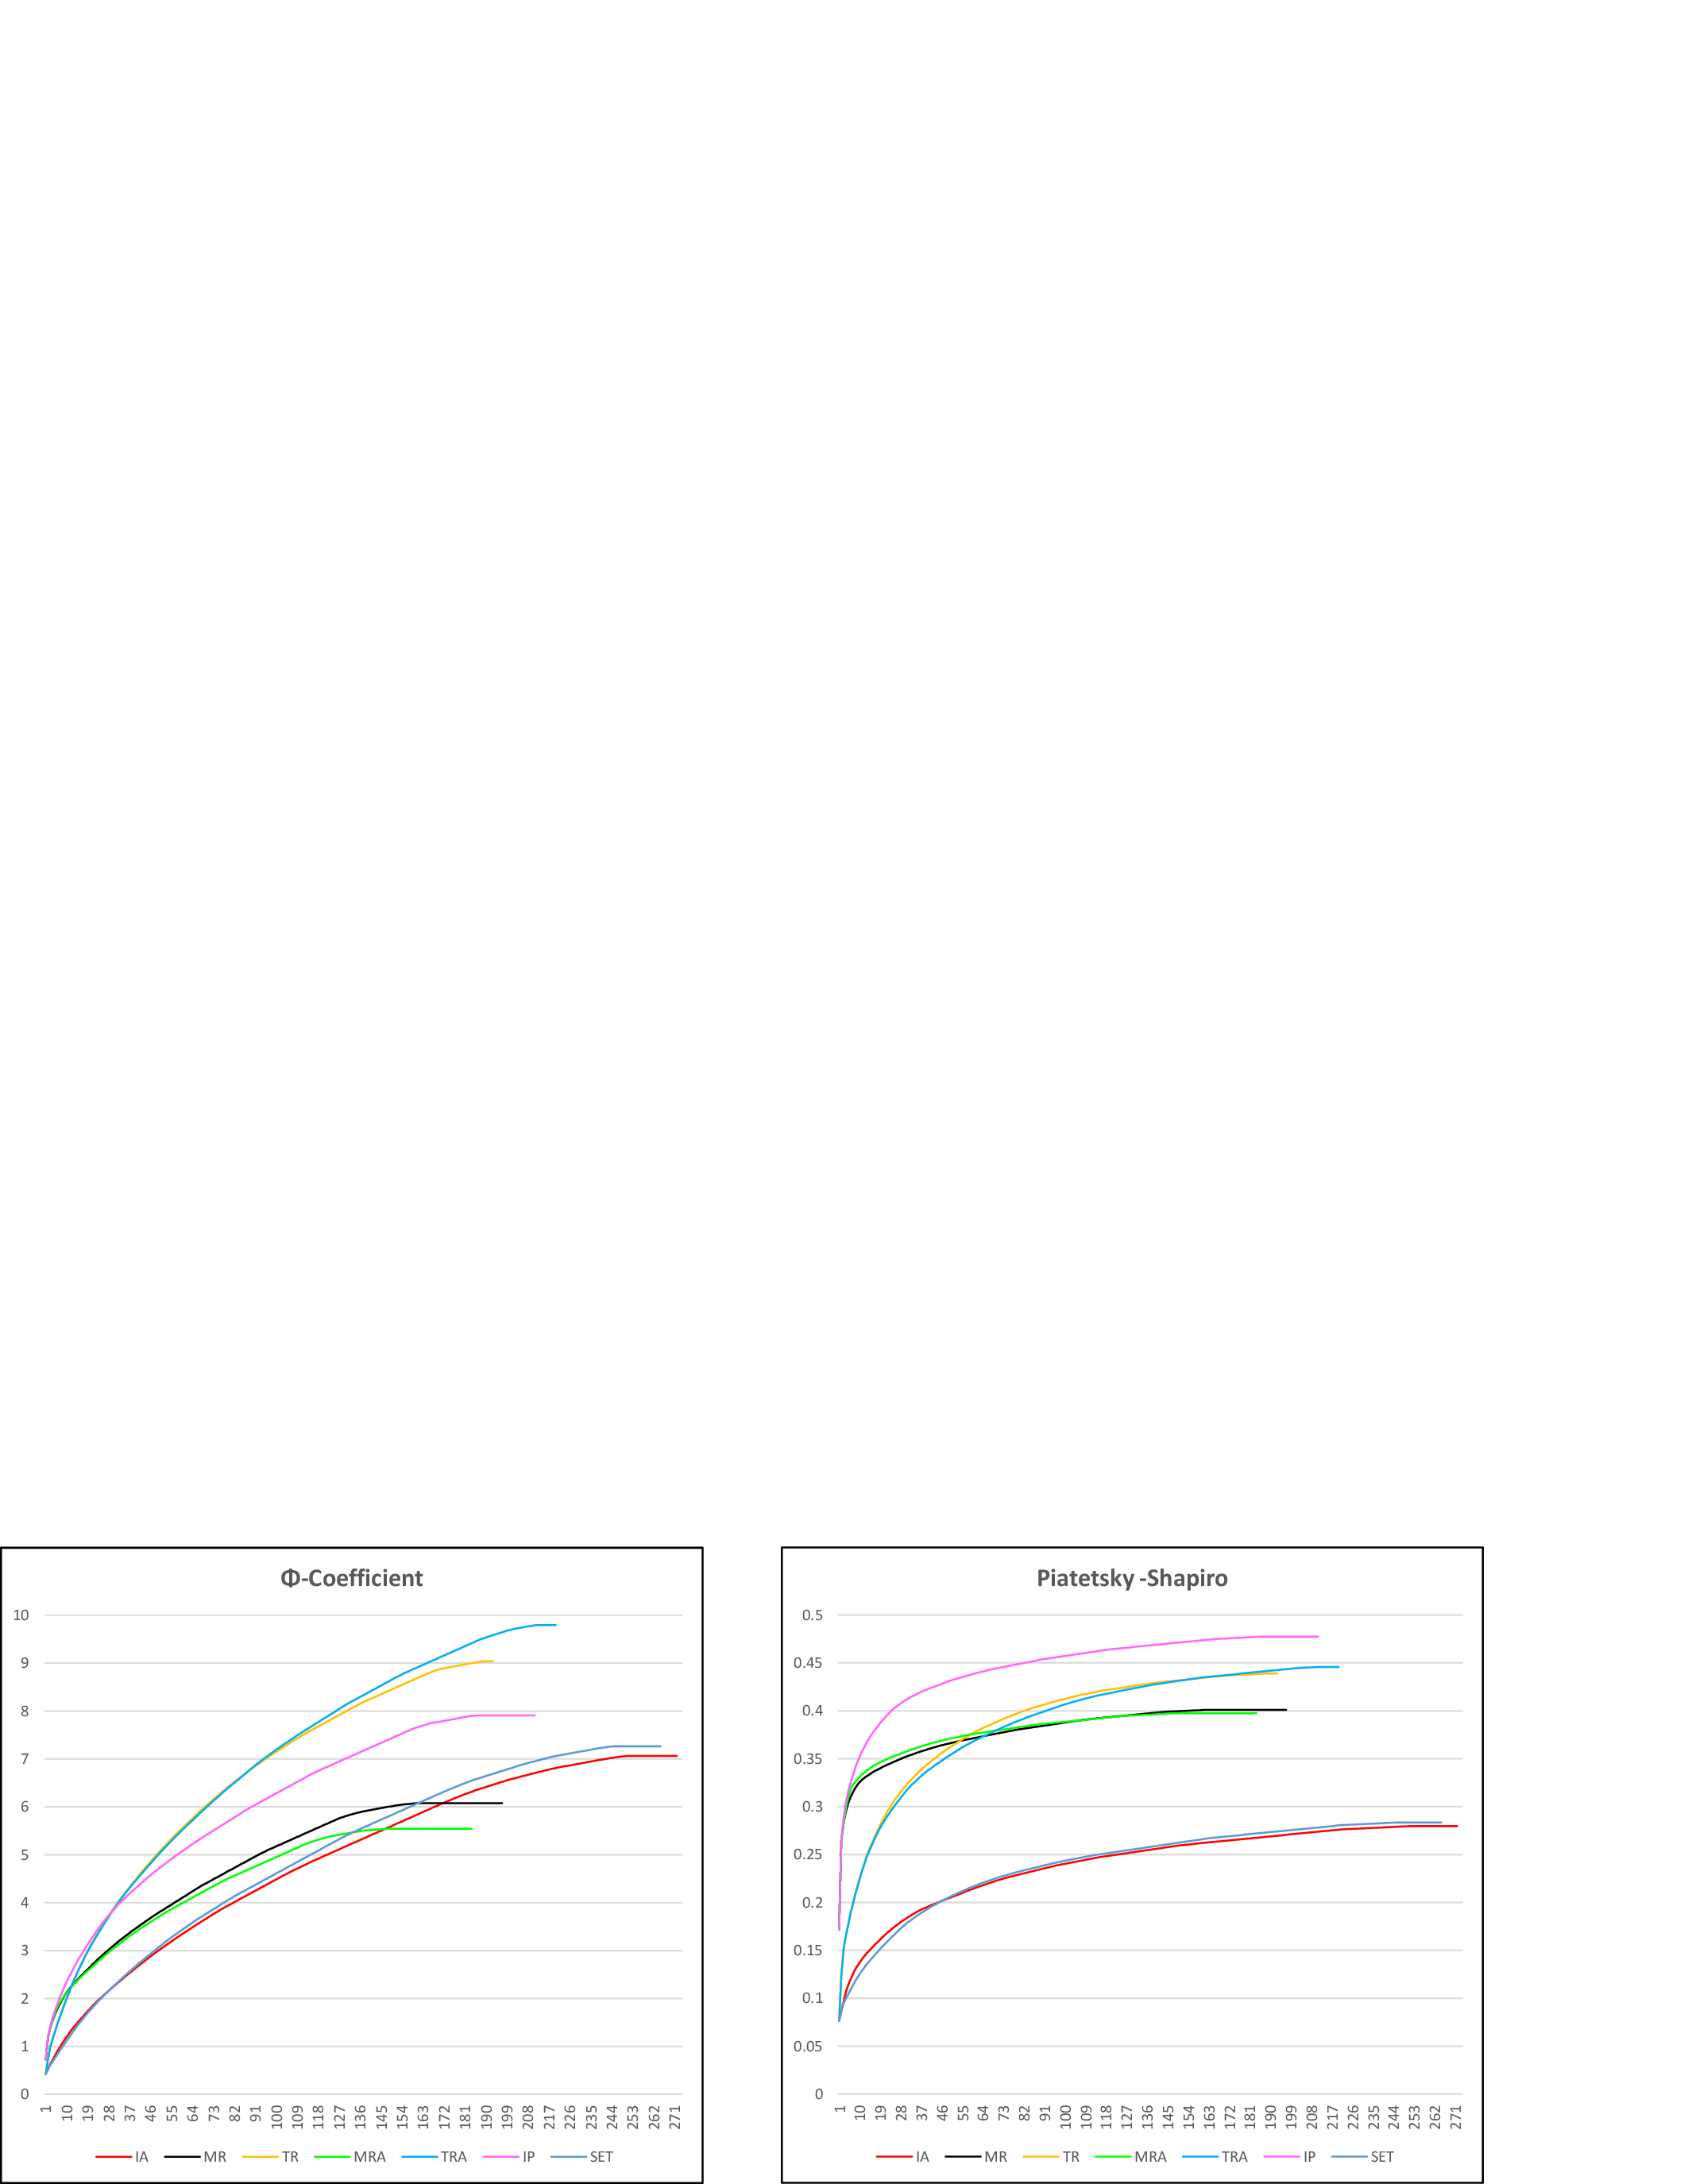}}
	\caption{Schedule dataset - \(\phi\)-Coefficient and Piatetsky-Shapiro}
	\label{fig:schedule-interest3}
\end{figure}

\begin{figure}[htb!]
	\centering
	{\includegraphics[width=\textwidth]{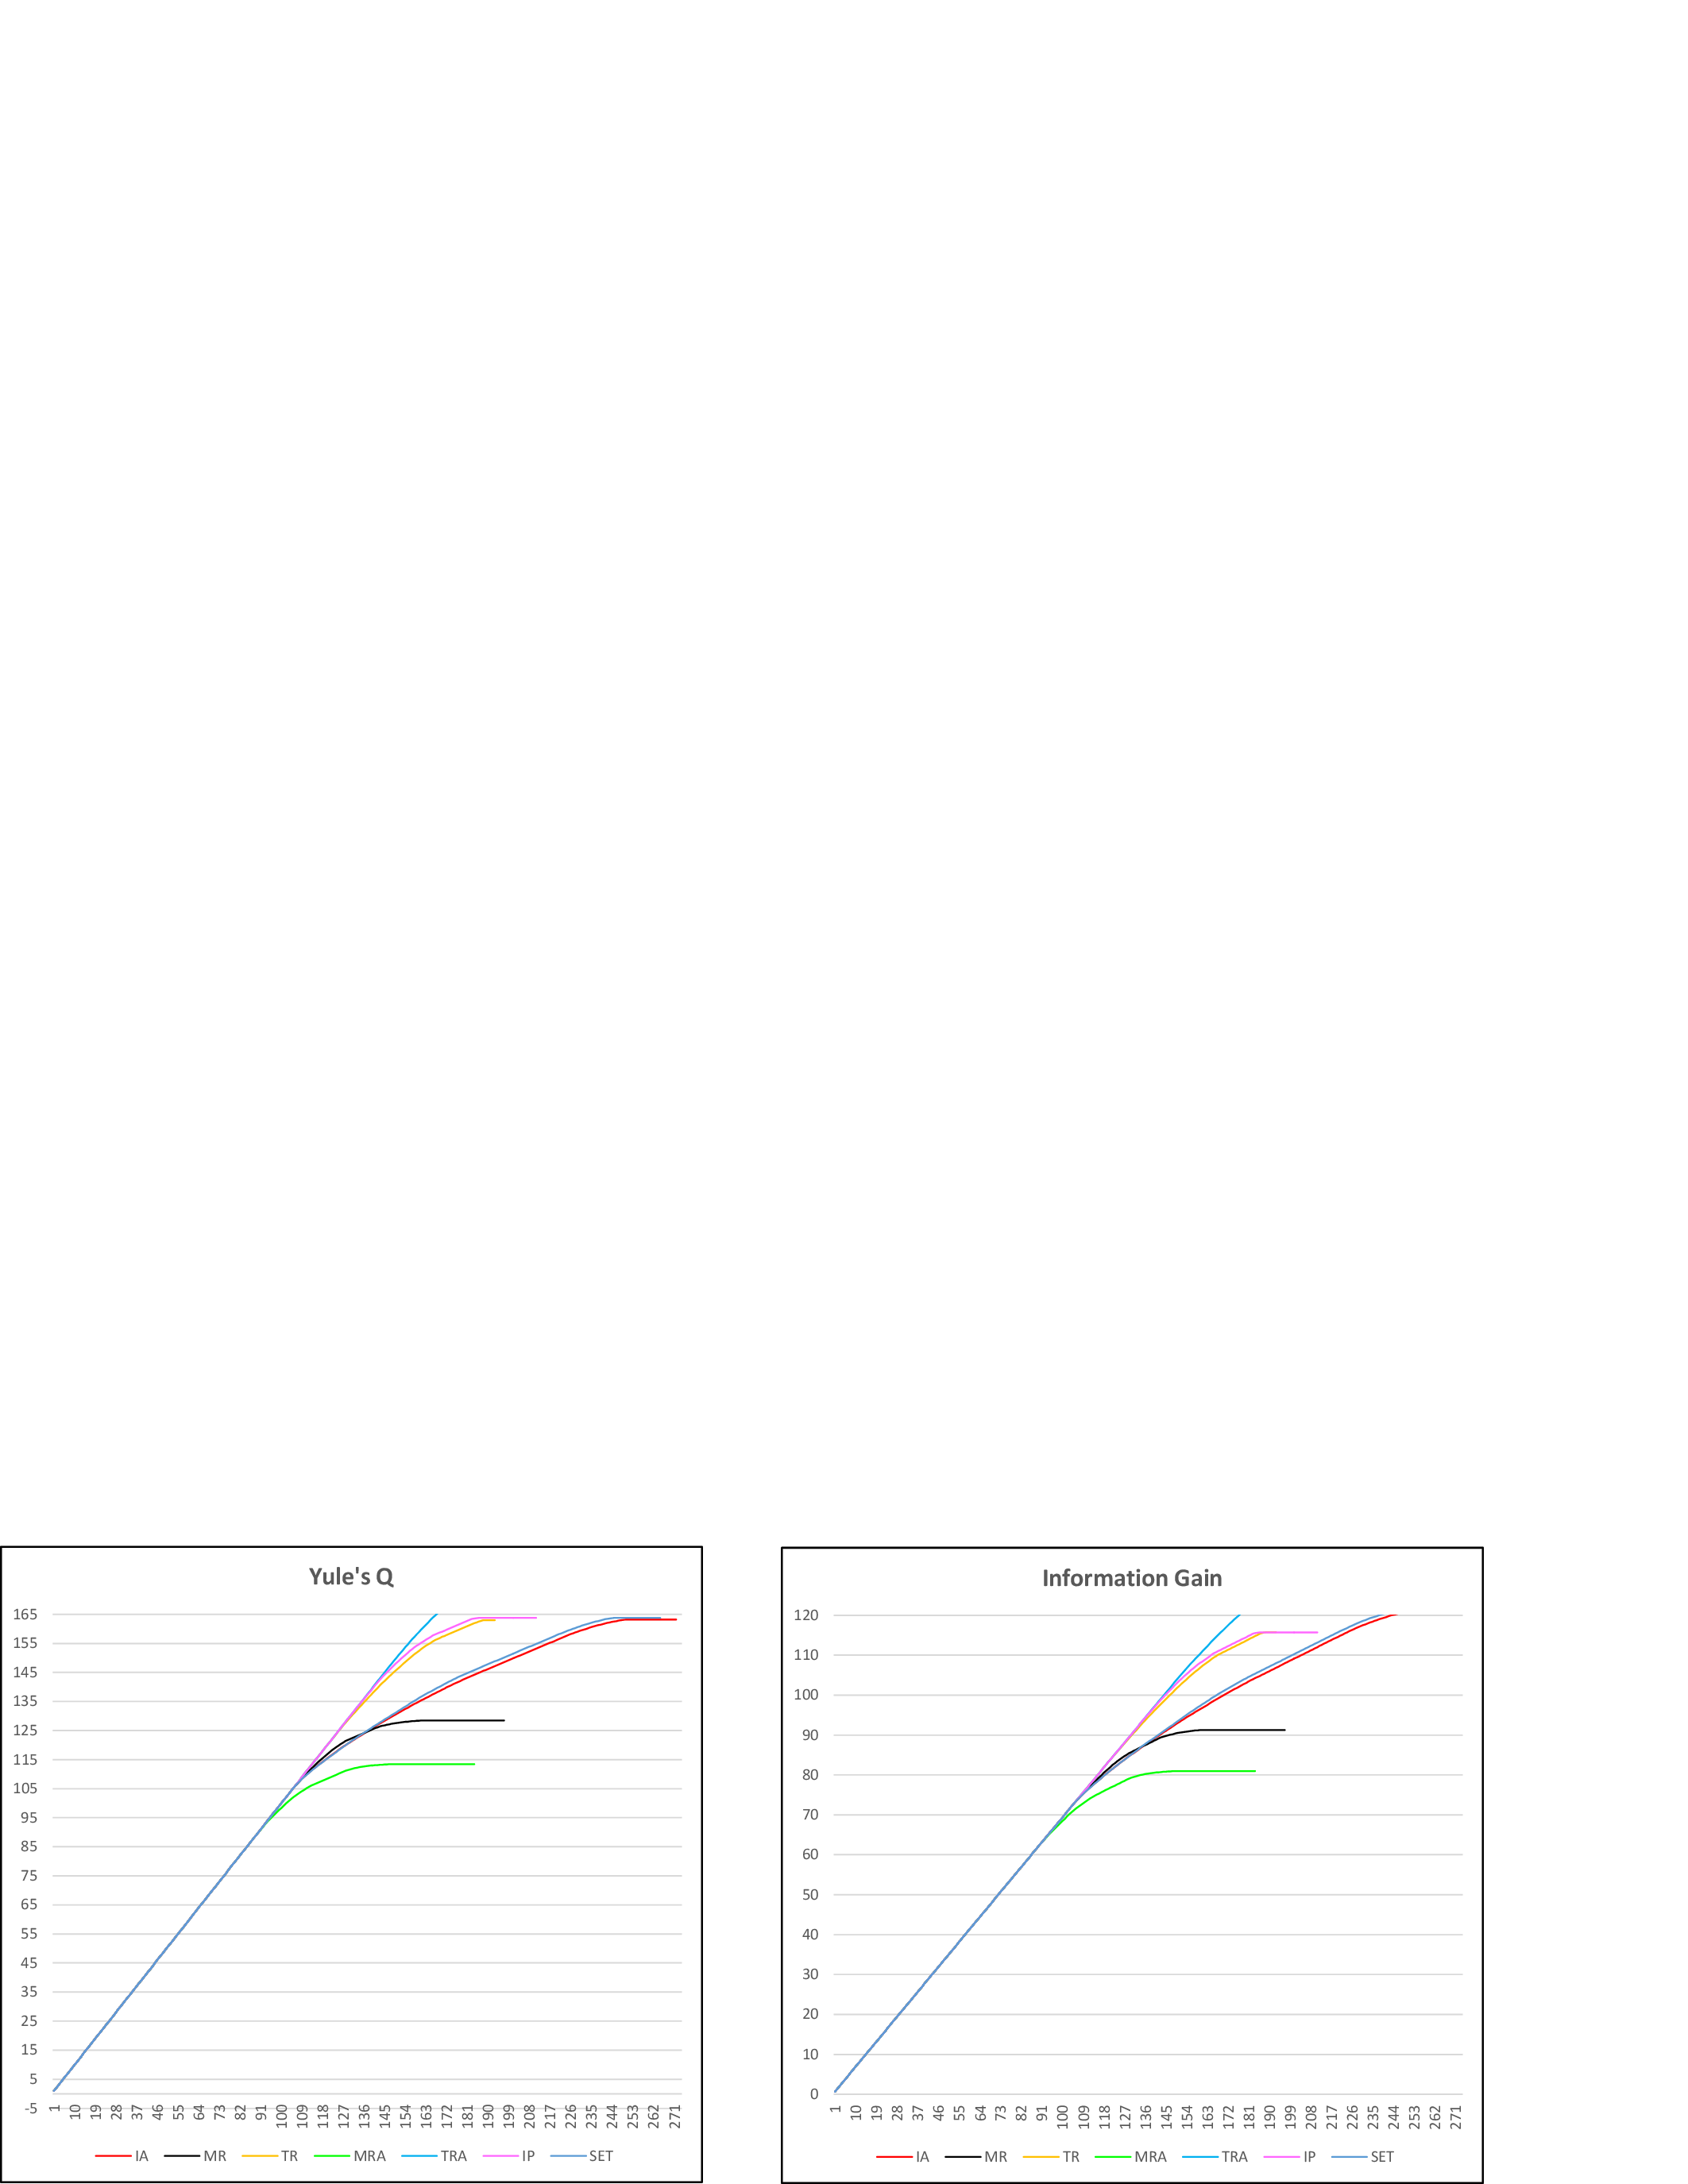}}
	\caption{Schedule dataset - Yule's Q and Information Gain}
	\label{fig:schedule-interest4}
\end{figure}
\FloatBarrier

\clearpage
\subsection{MySQL Dataset}

\FloatBarrier
\begin{figure}[!htb]
	{\includegraphics[scale=0.8]{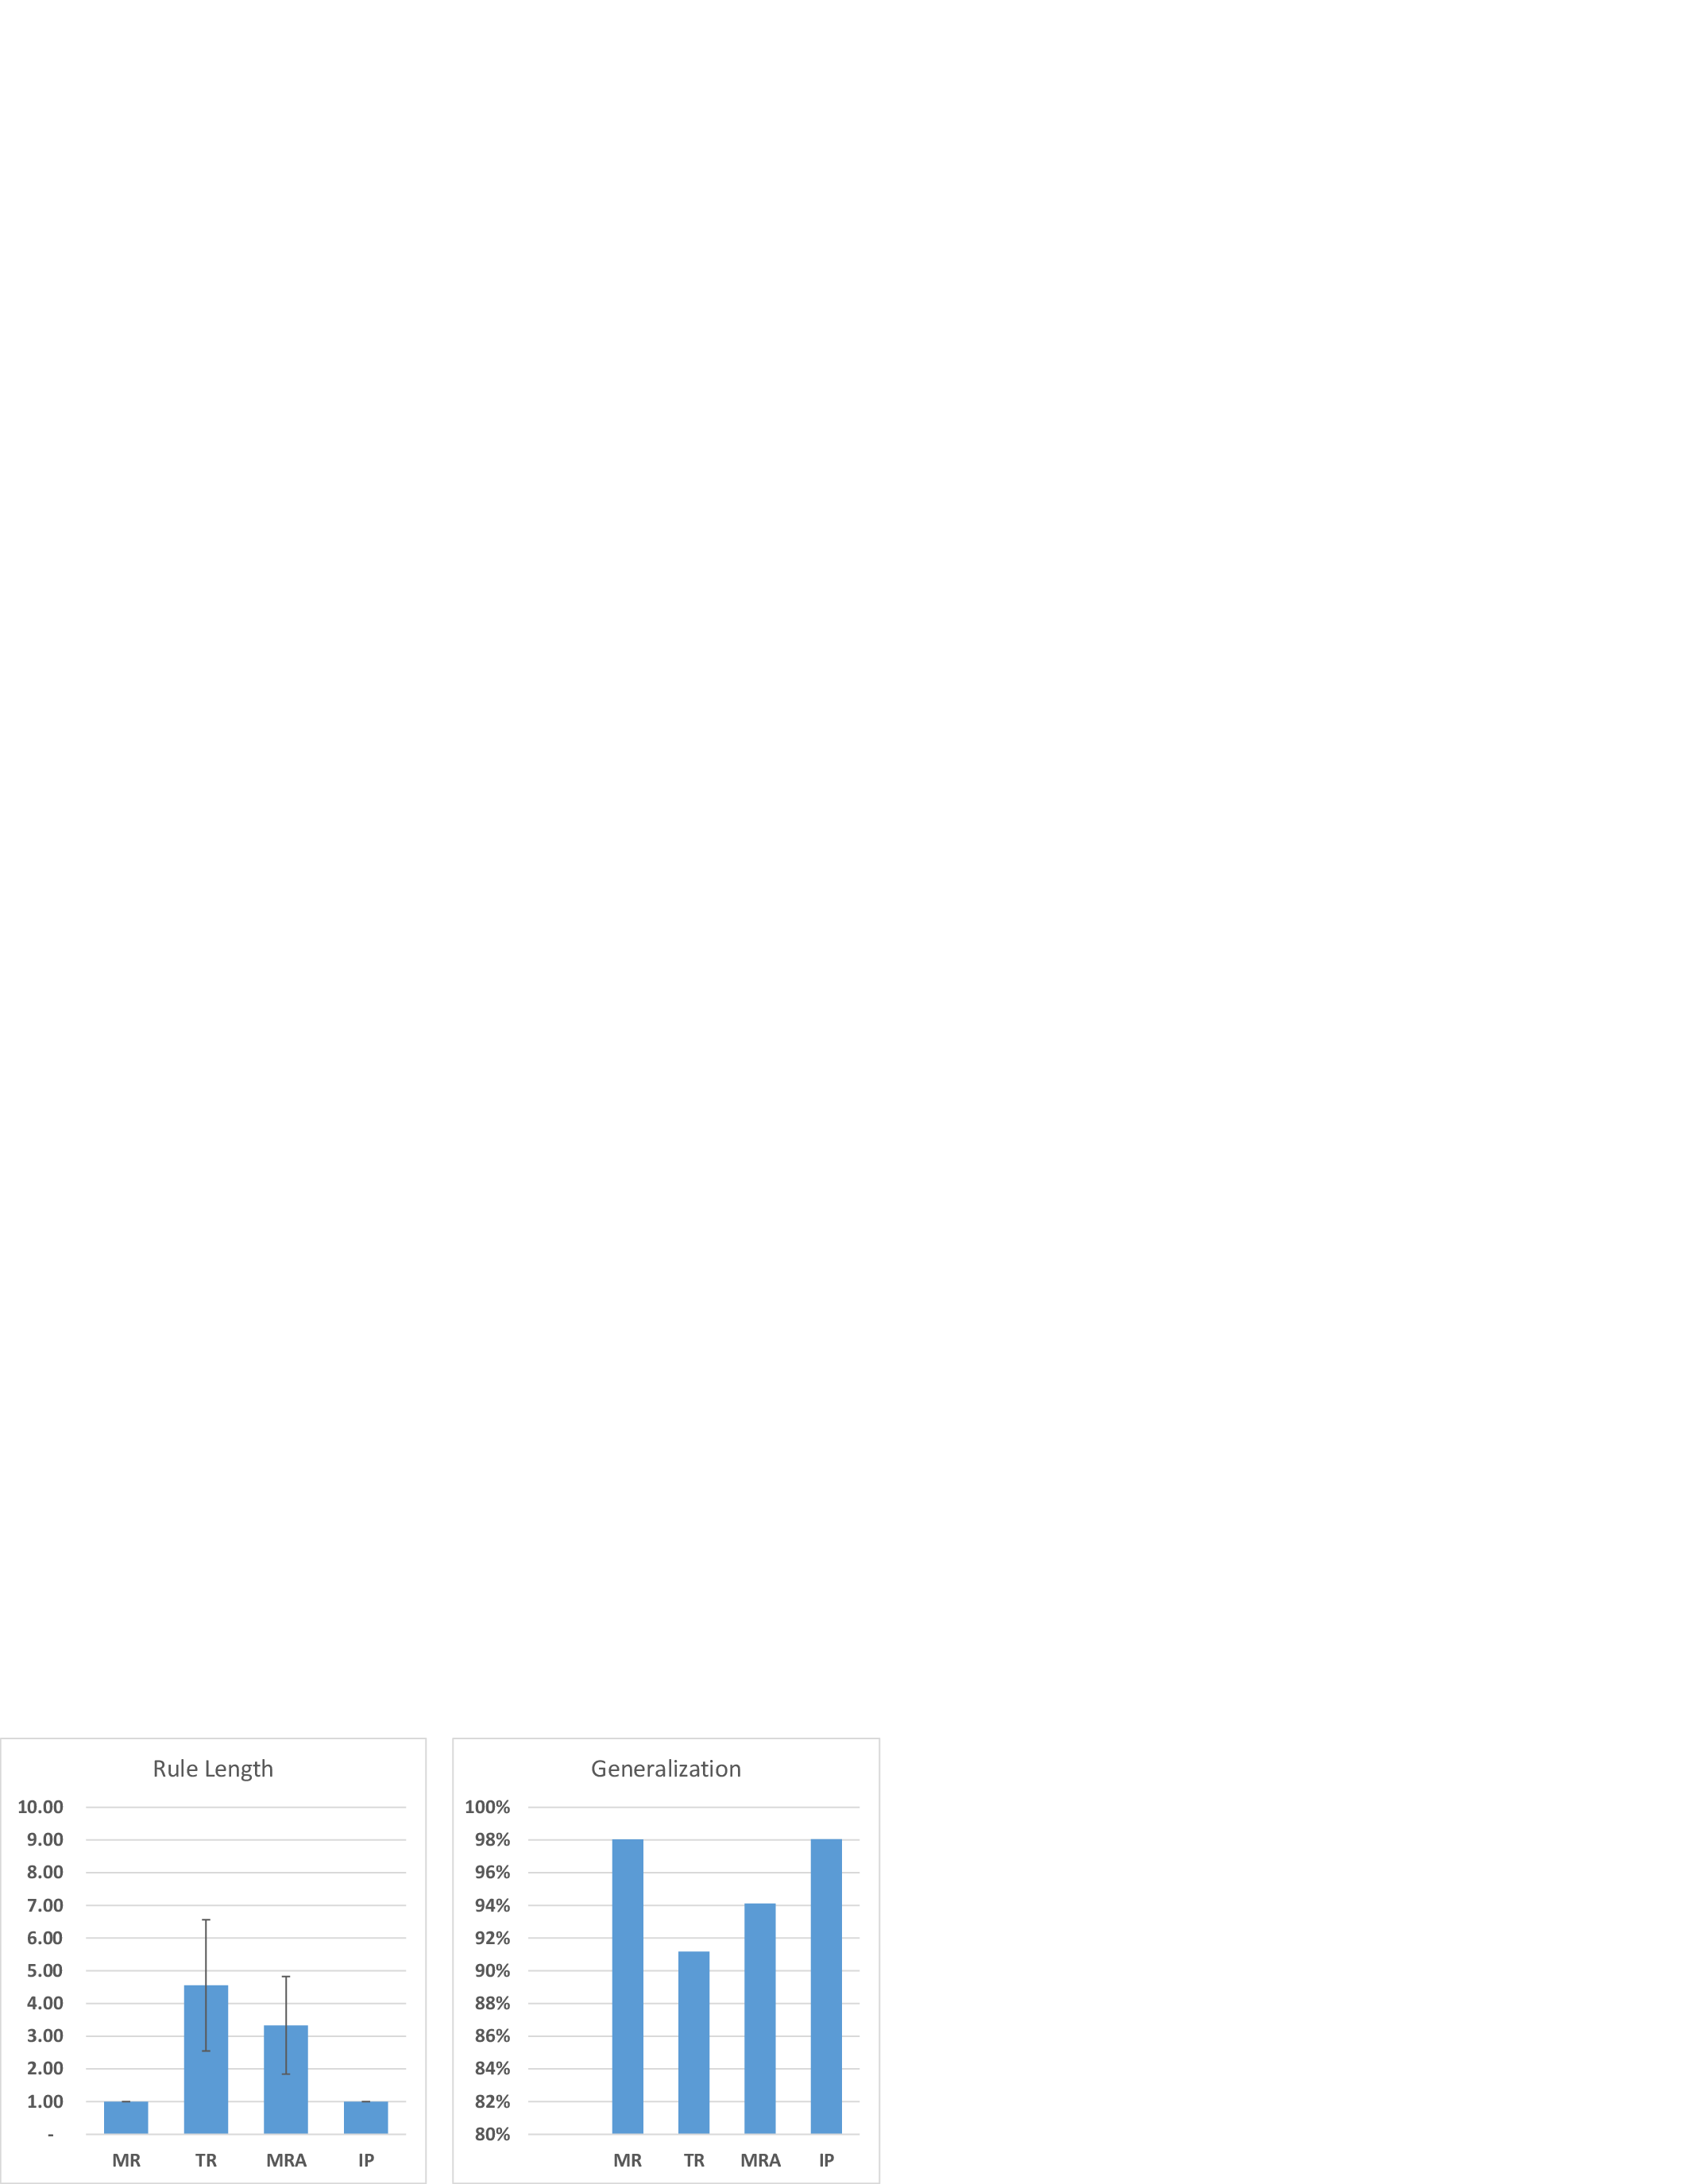}}
	\caption{MySQL dataset - Rule Length \& \%Generalization}
	\label{fig:mysql-interest5}
\end{figure}

\begin{figure}[!htb]
	\centering		
	{\includegraphics[width=\textwidth]{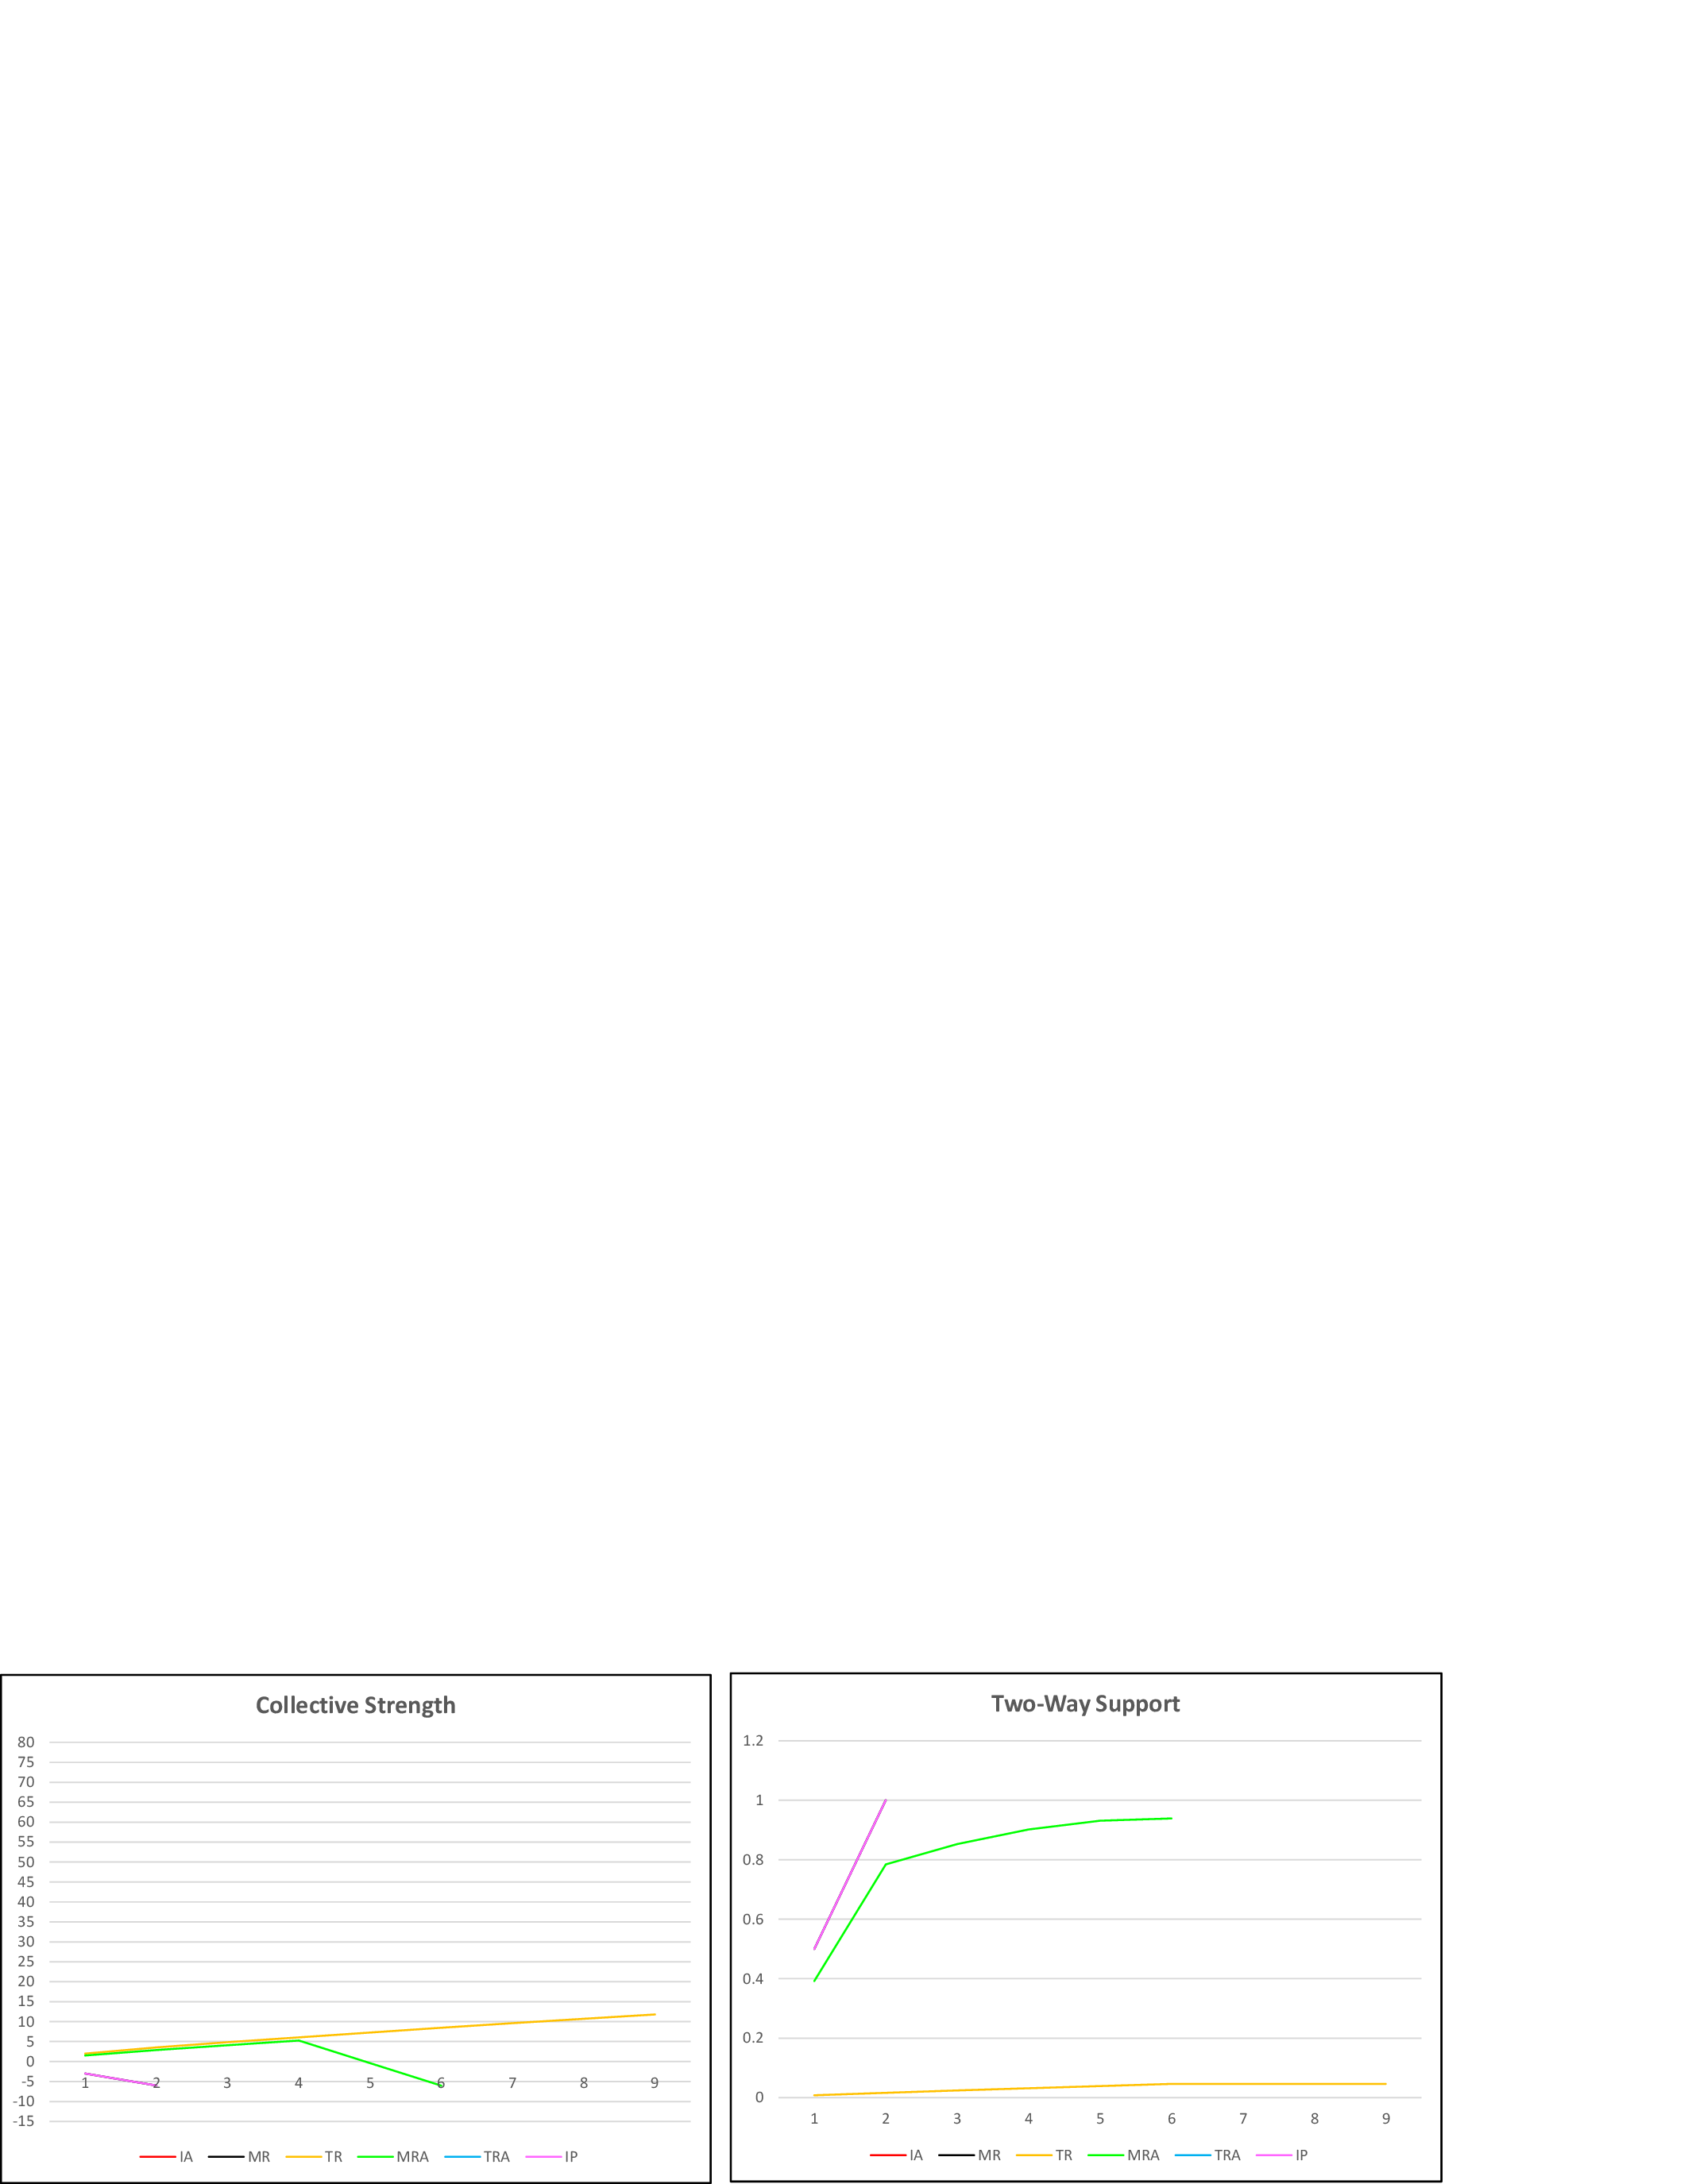}}
	\caption{MySQL dataset - Collective Strength and Two-Way Support}
	\label{fig:mysql-interest2}
\end{figure}

\begin{figure}[!htb]
	\centering
	{\includegraphics[width=\textwidth]{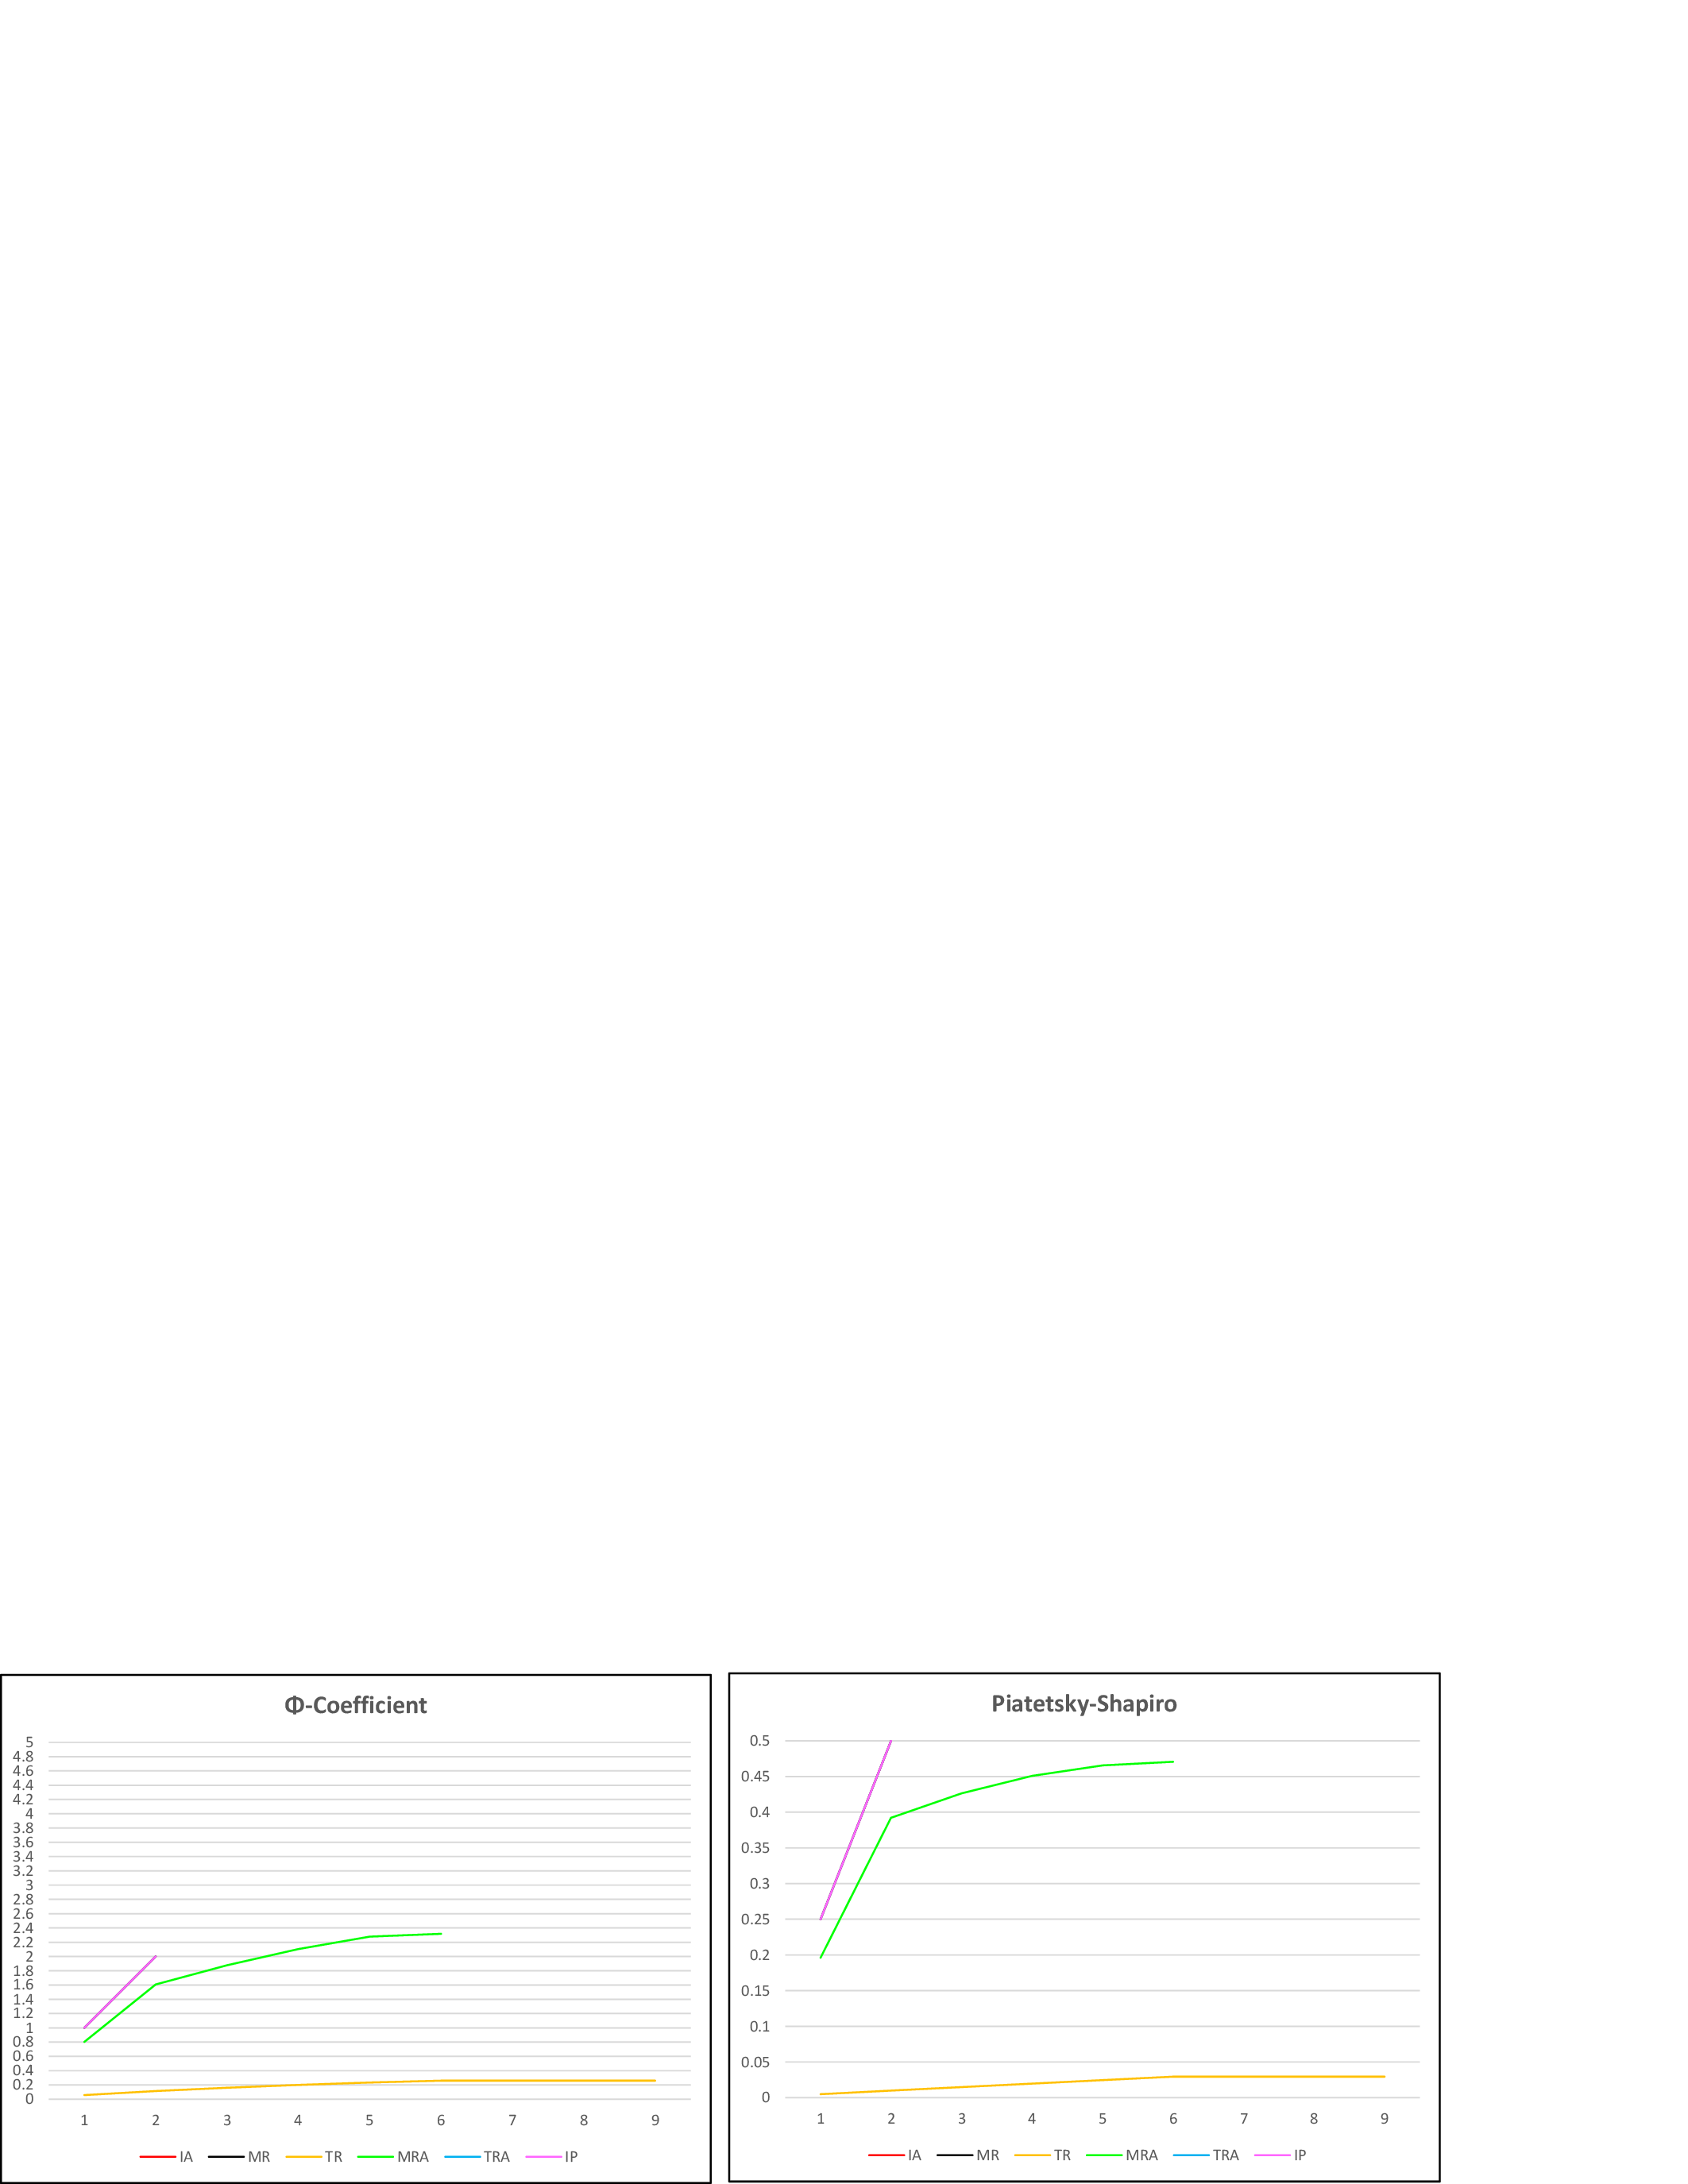}}
	\caption{MySQL dataset - \(\phi\)-Coefficient and Piatetsky-Shapiro}
	\label{fig:mysql-interest3}	
\end{figure}
	
\begin{figure}[!htb]
	\centering	
	{\includegraphics[width=\textwidth]{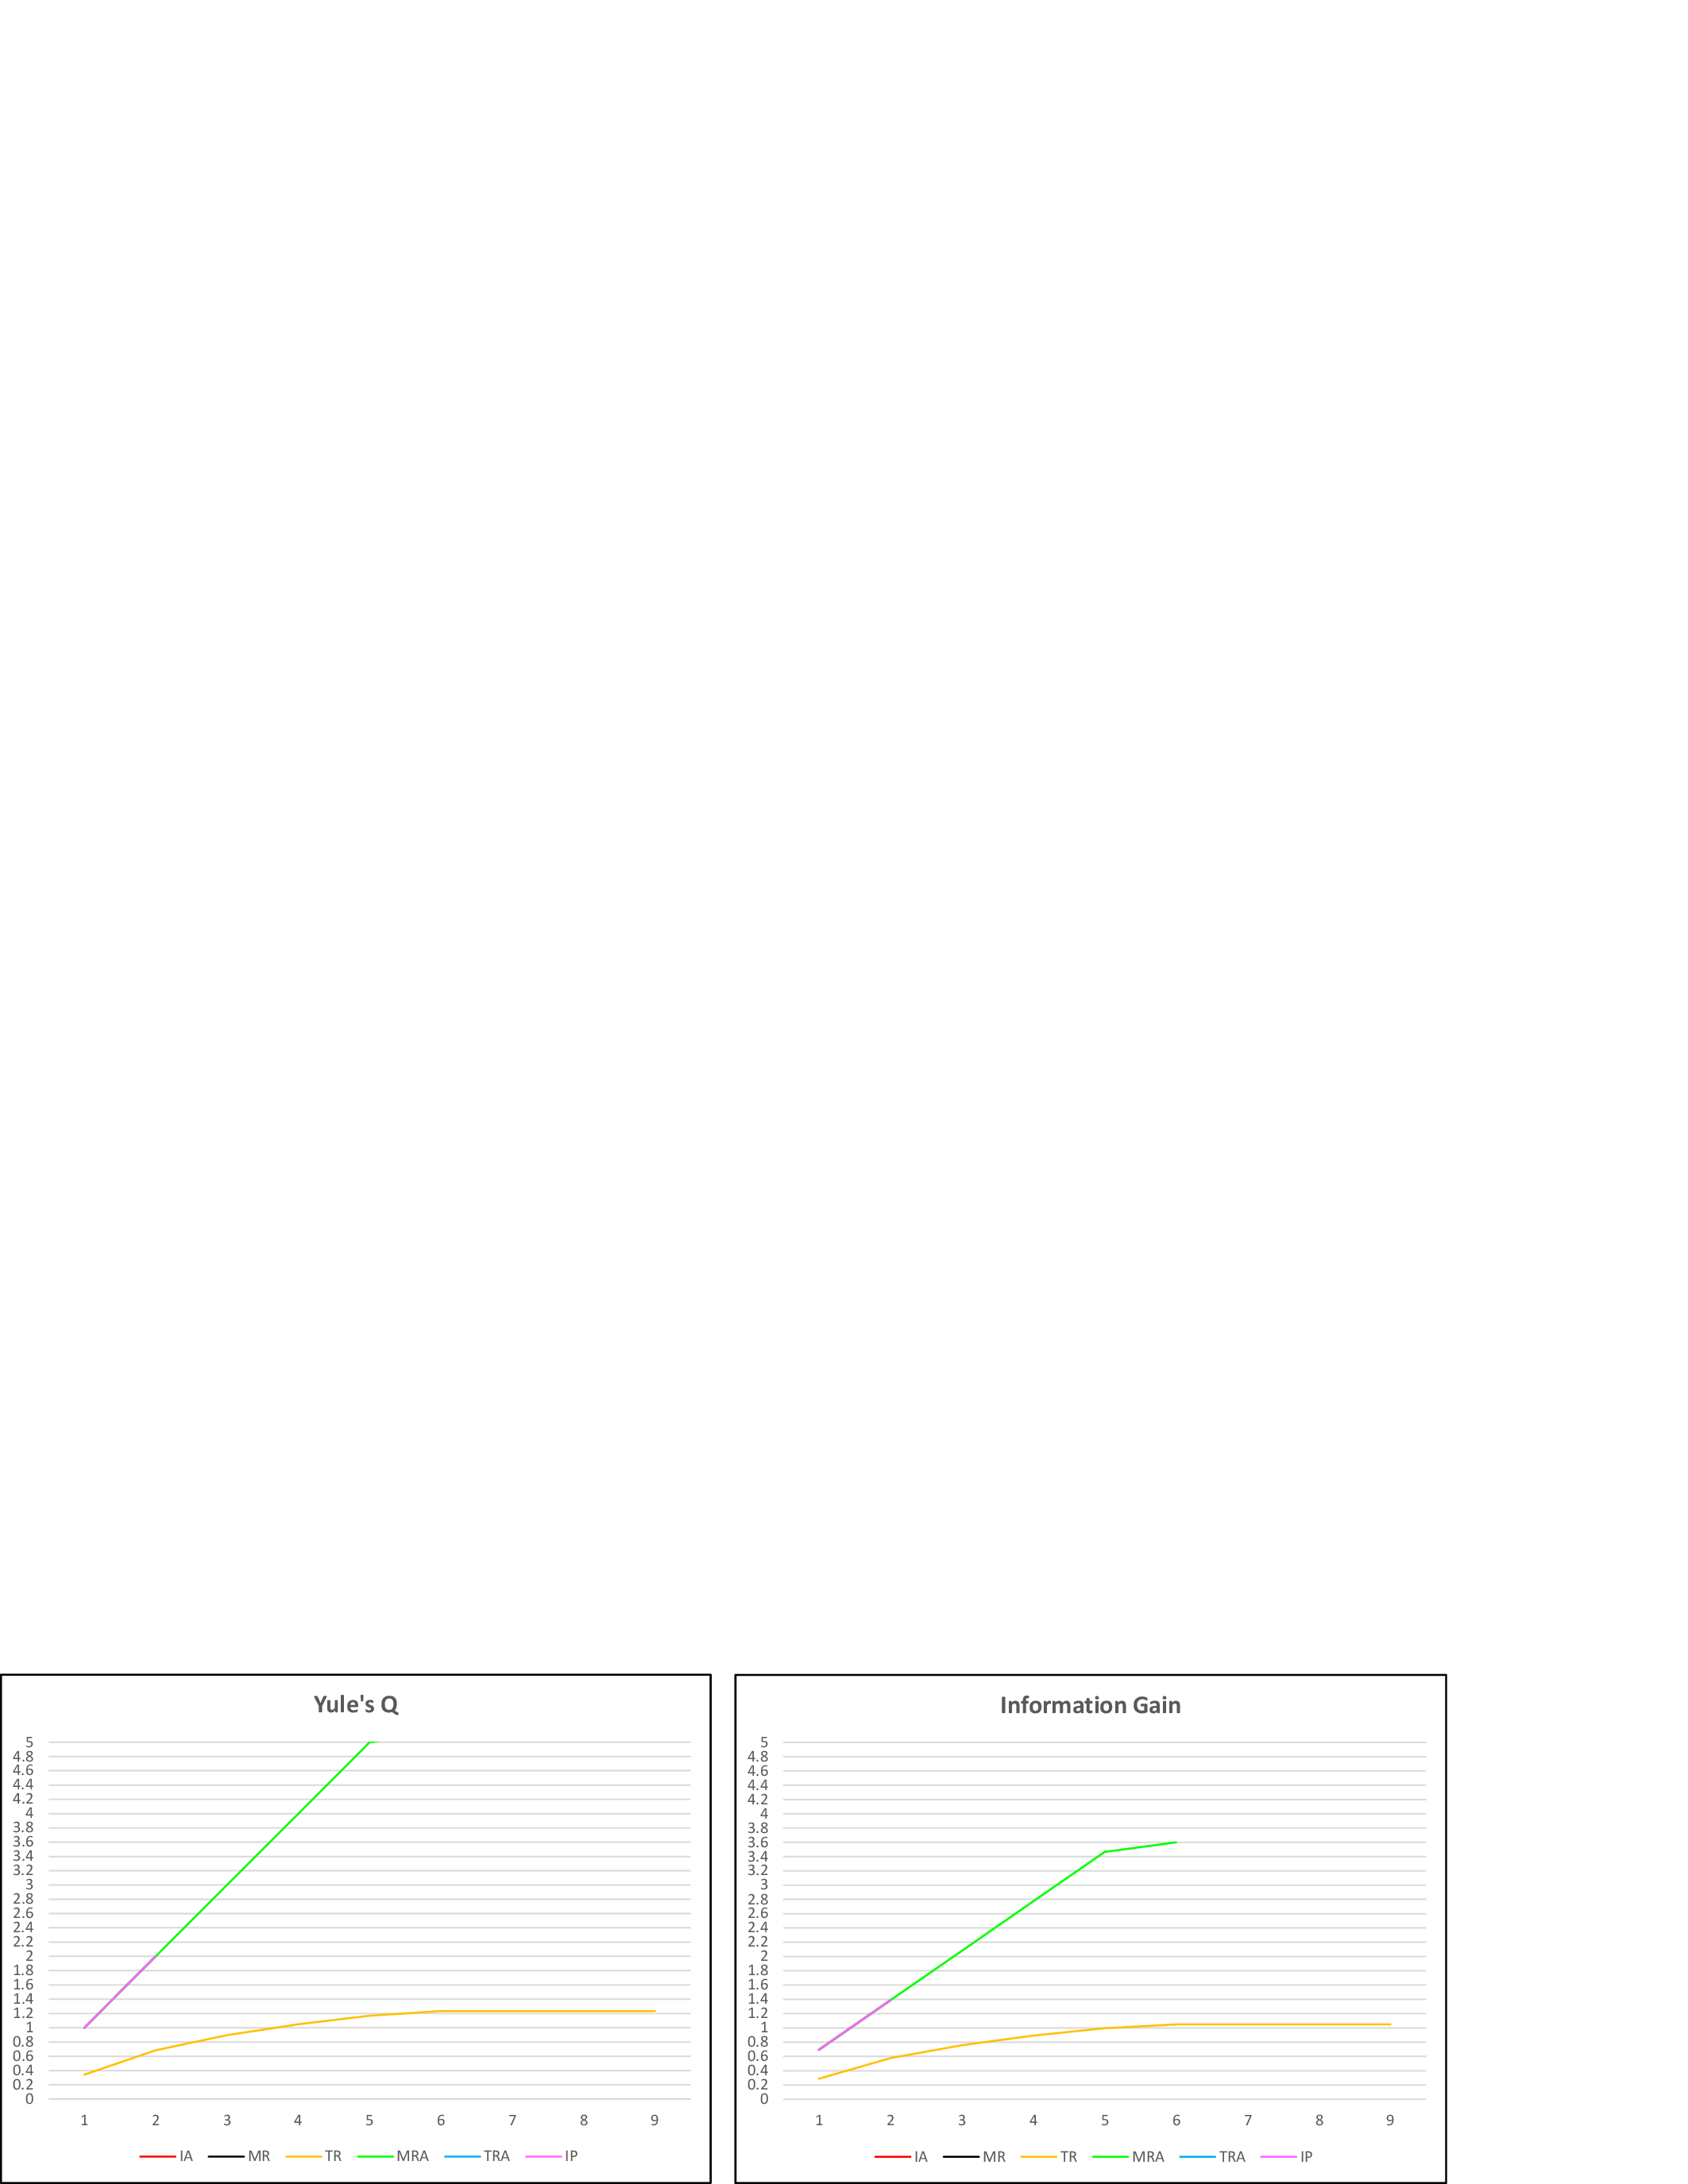}}
	\caption{MySQL dataset - Yule's Q and Information Gain}
	\label{fig:mysql-interest4}
\end{figure}
\FloatBarrier

\clearpage
\subsection{Hospital1 Dataset}

\FloatBarrier
\begin{figure}[!htb]
	\centering
	{\includegraphics[width=\textwidth]{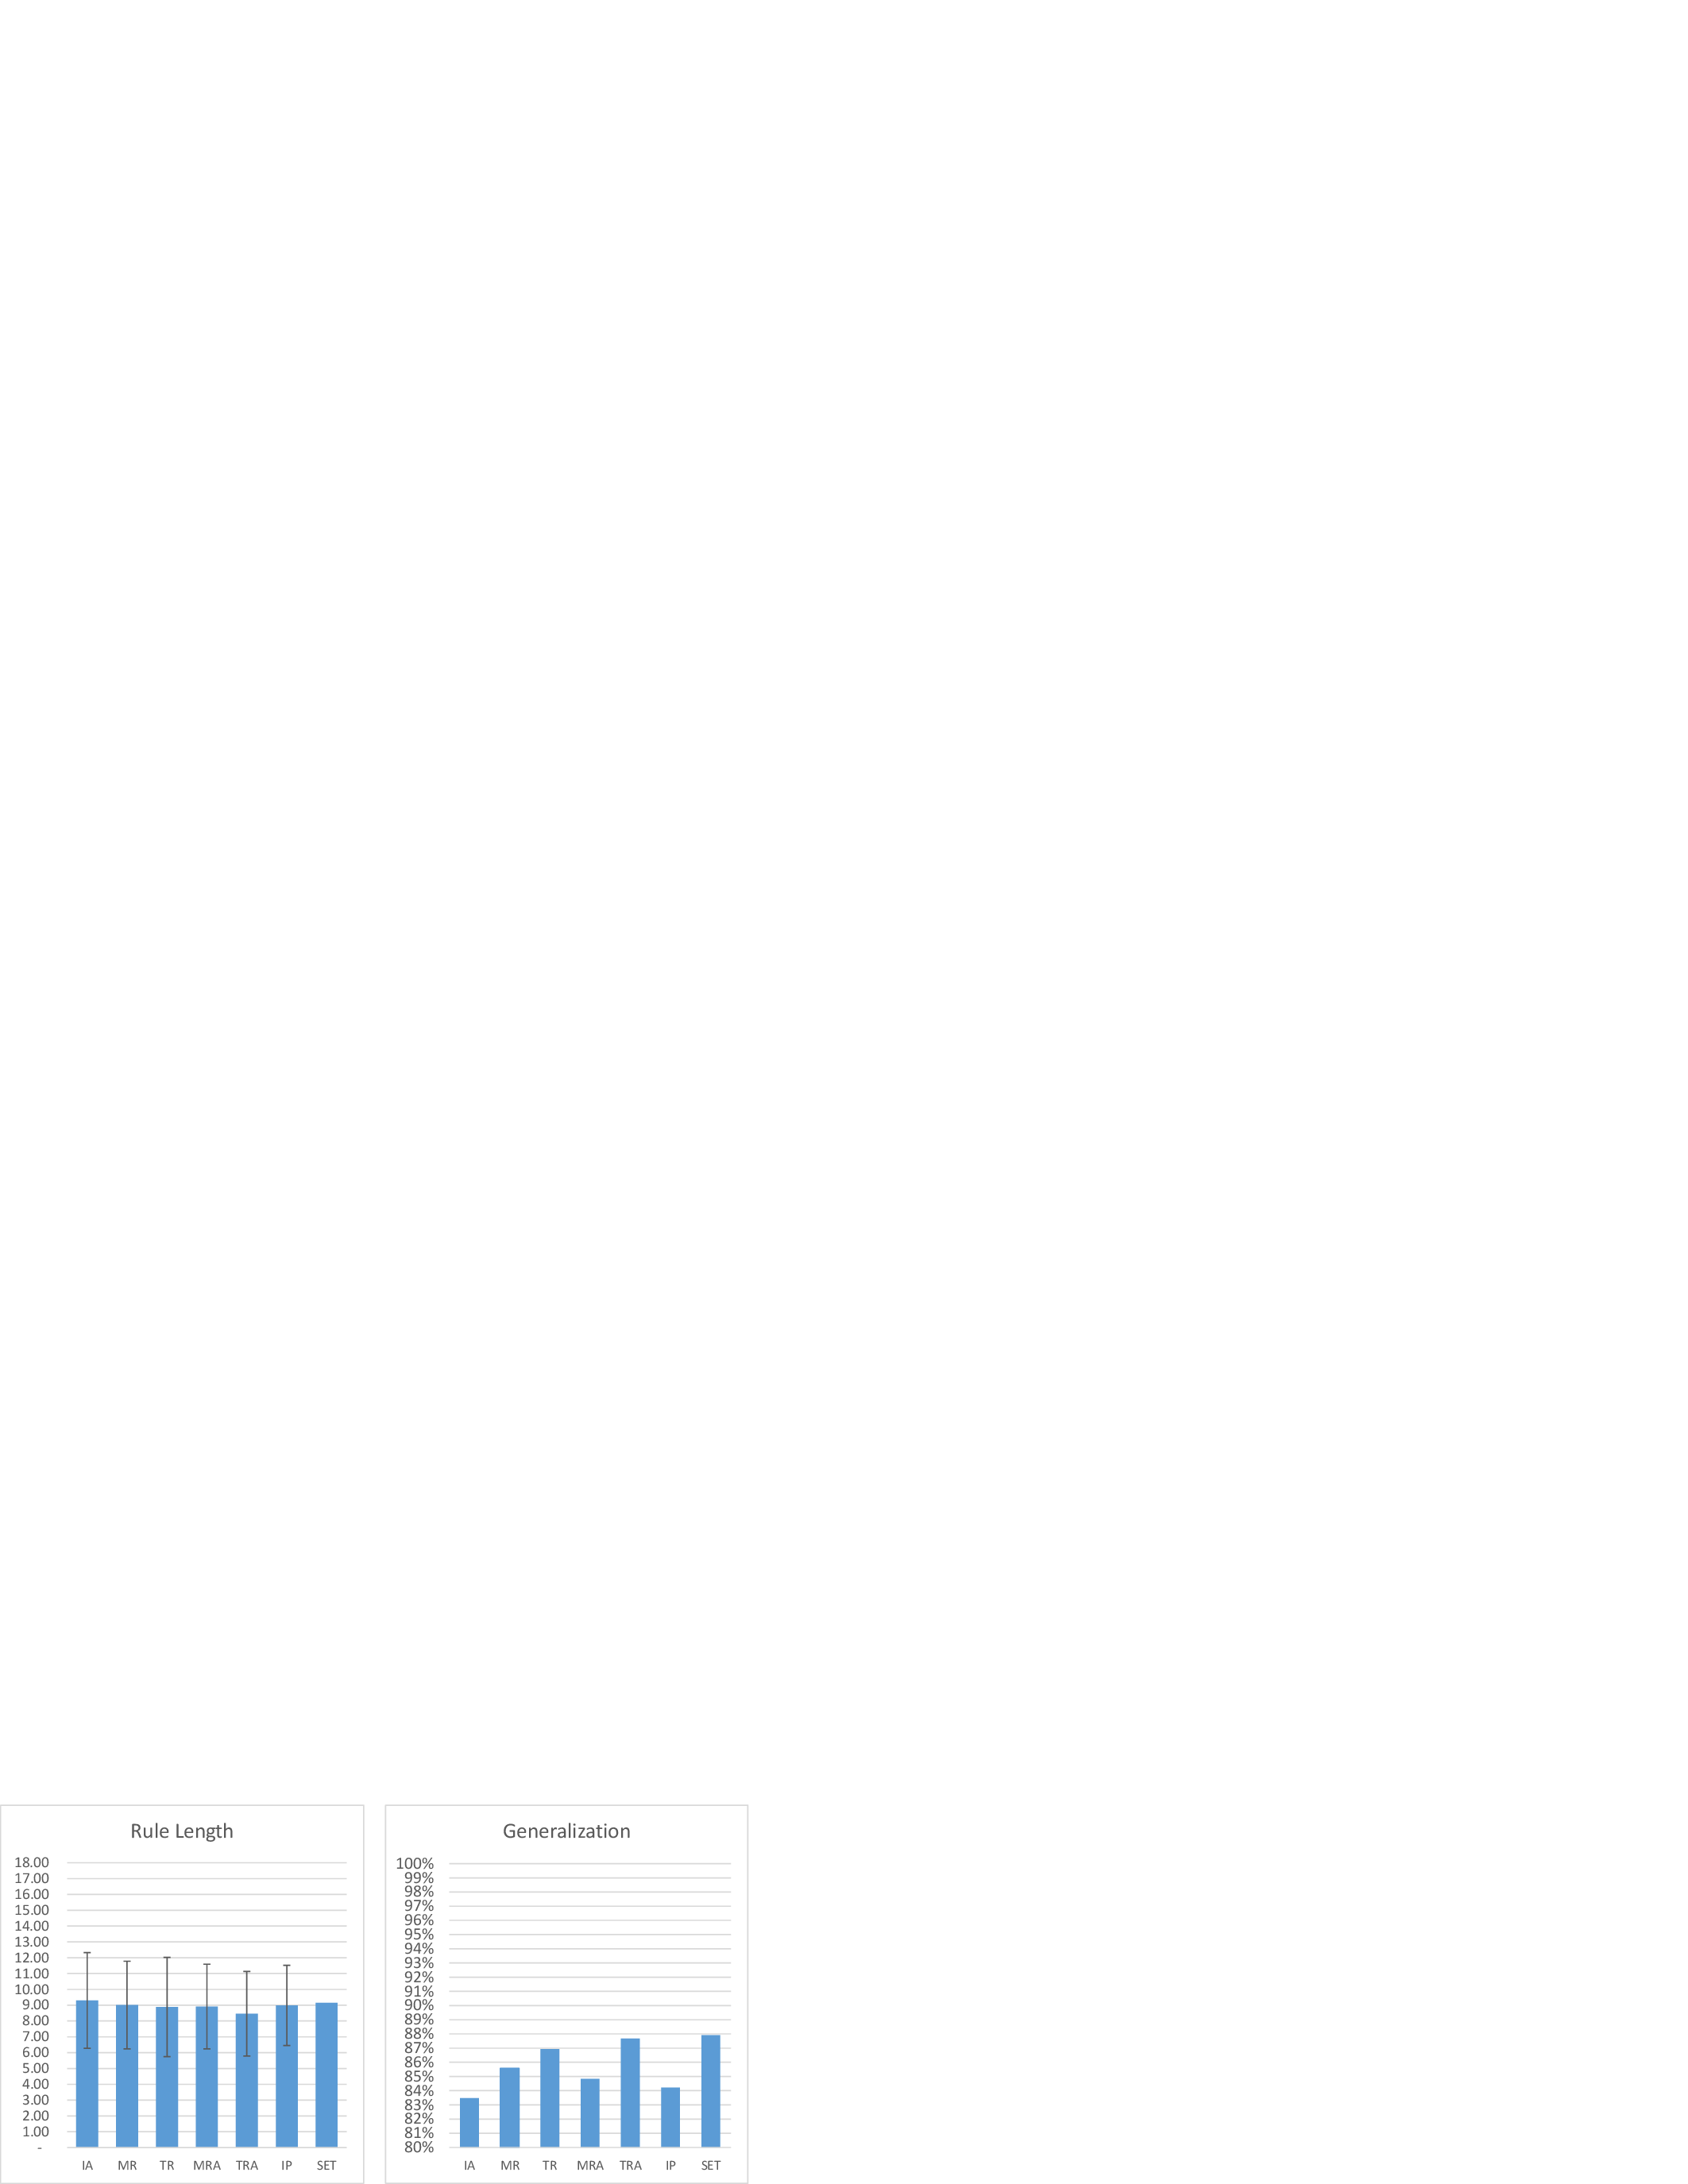}}
	\caption{Hospital1 dataset - Rule Length \& \%Generalization}
	\label{fig:hospital1-interest5}
\end{figure}
	
\begin{figure}[!htb]
	{\includegraphics[width=\textwidth]{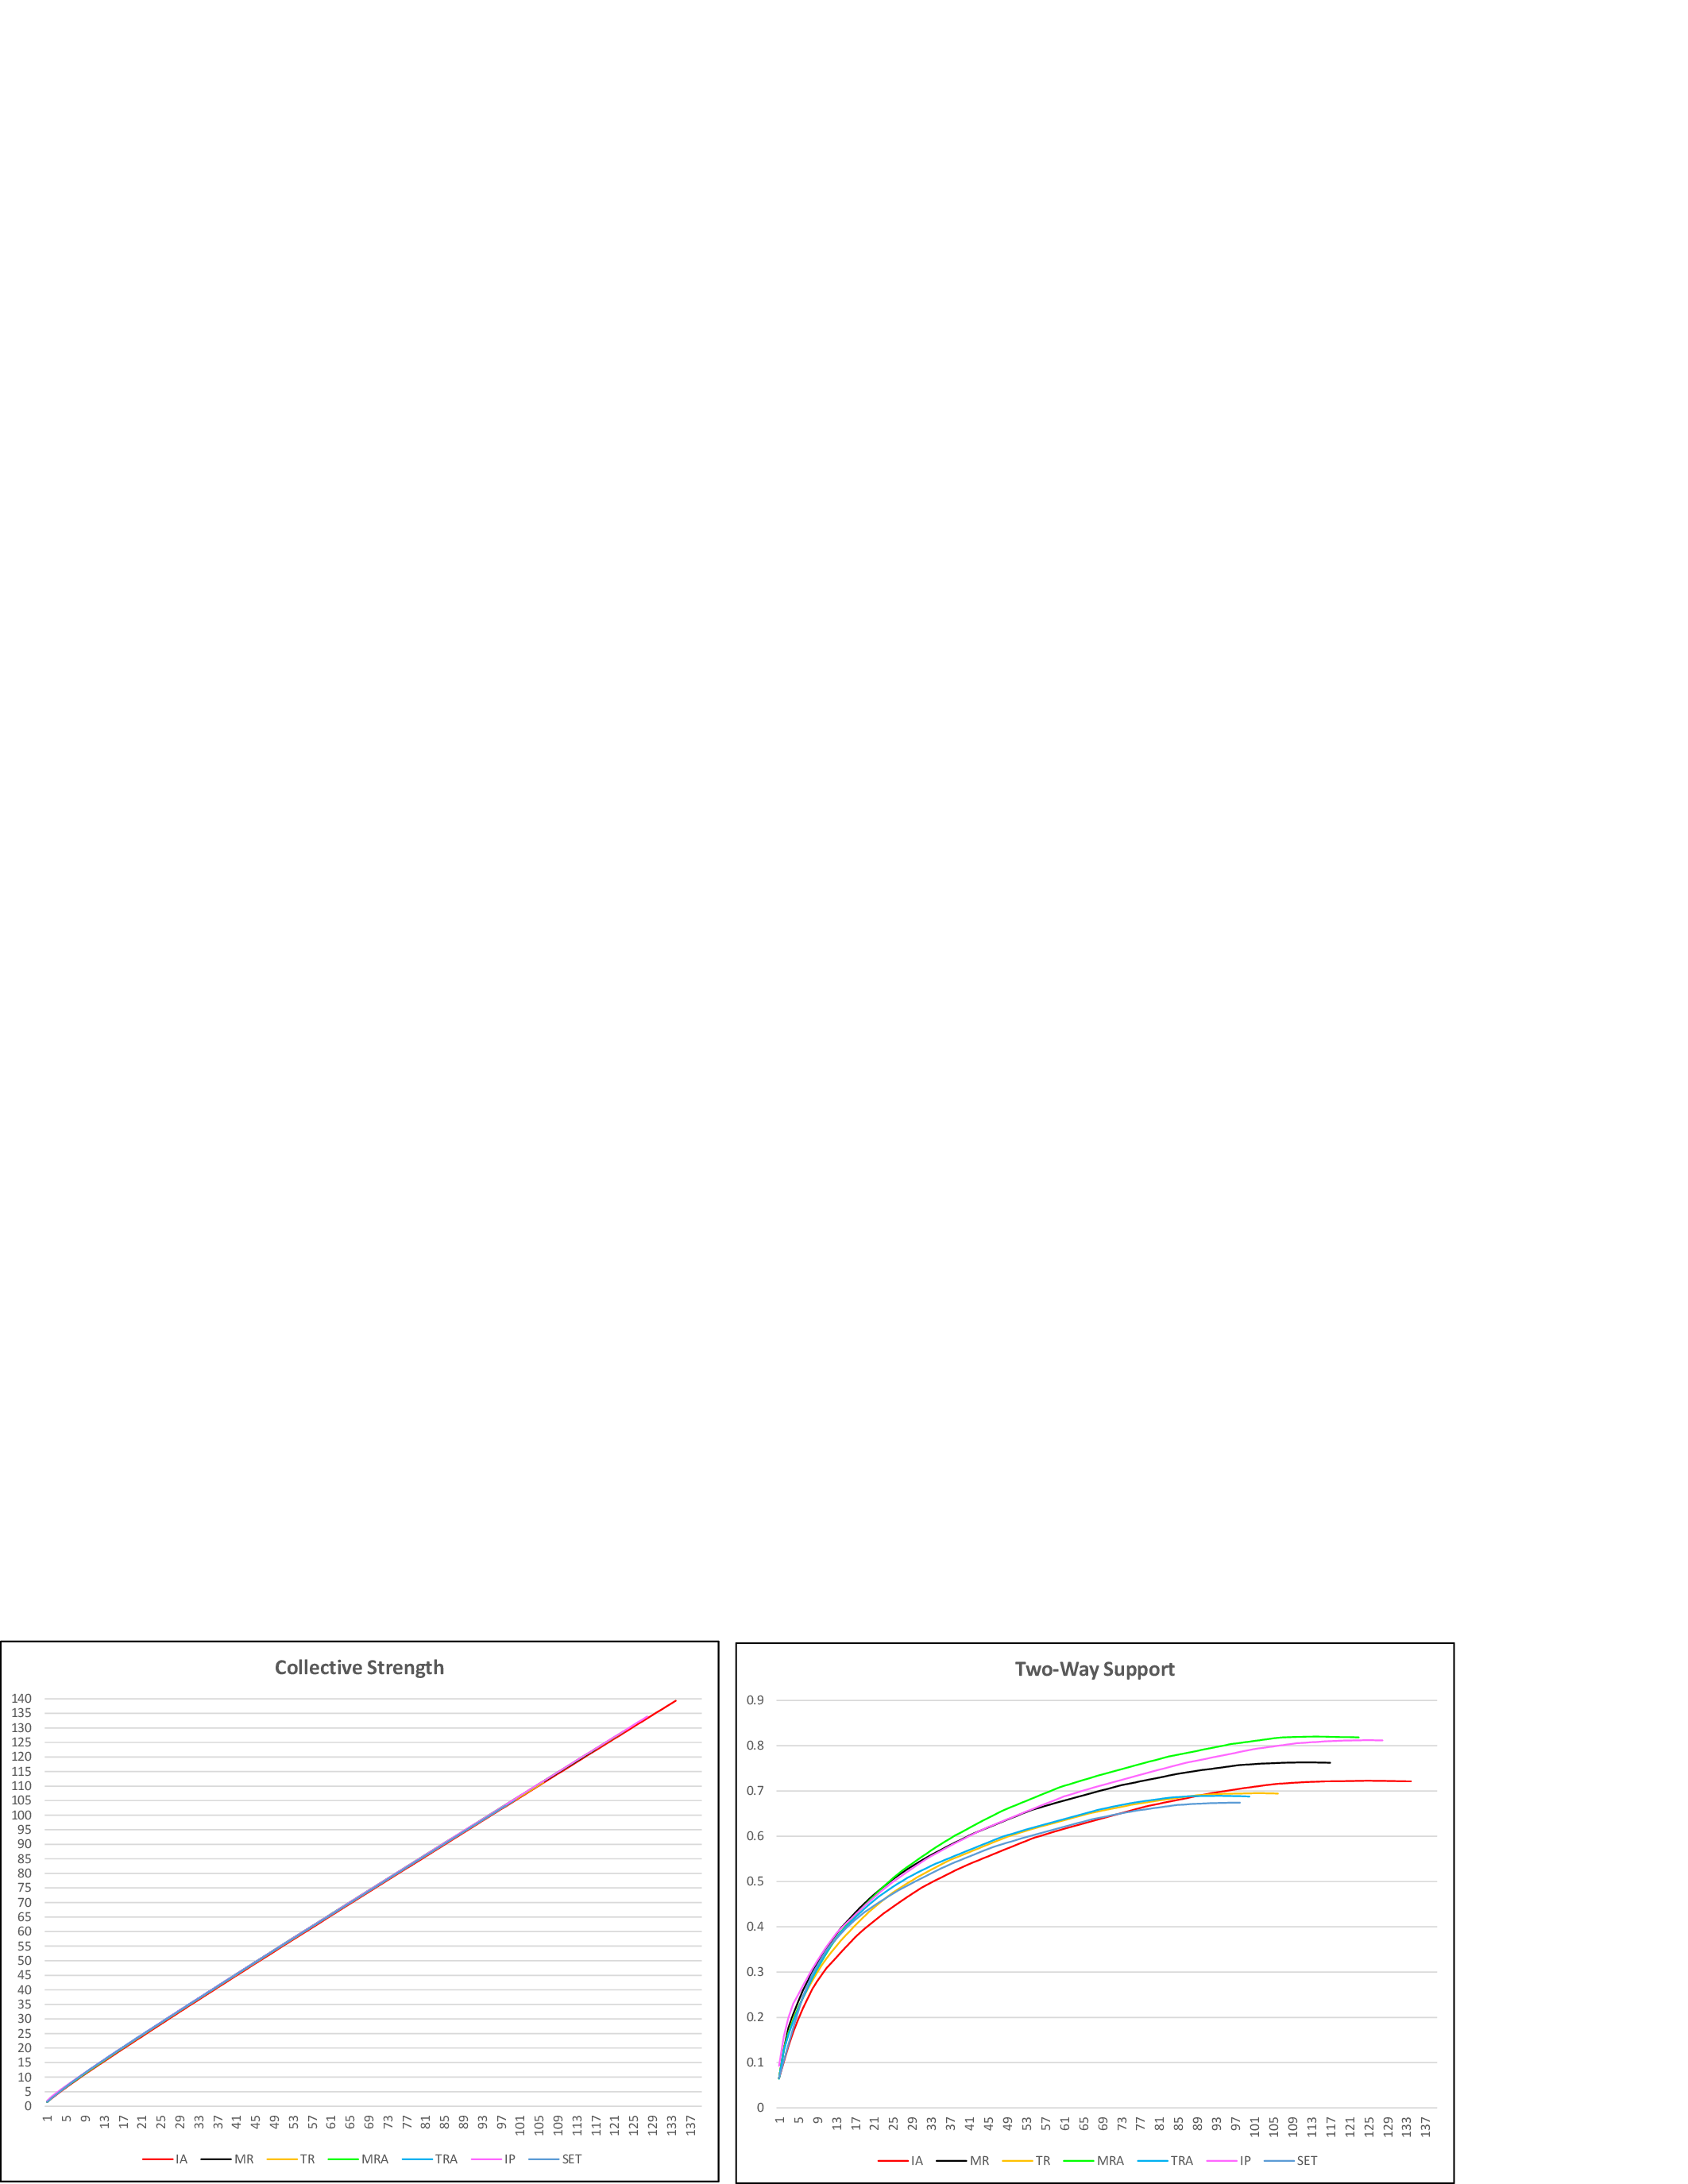}}
	\caption{Hospital1 dataset - Collective Strength and Two-Way Support}
	\label{fig:hospital1-interest2}
\end{figure}

\begin{figure}[!htb]
	\centering
	{\includegraphics[width=\textwidth]{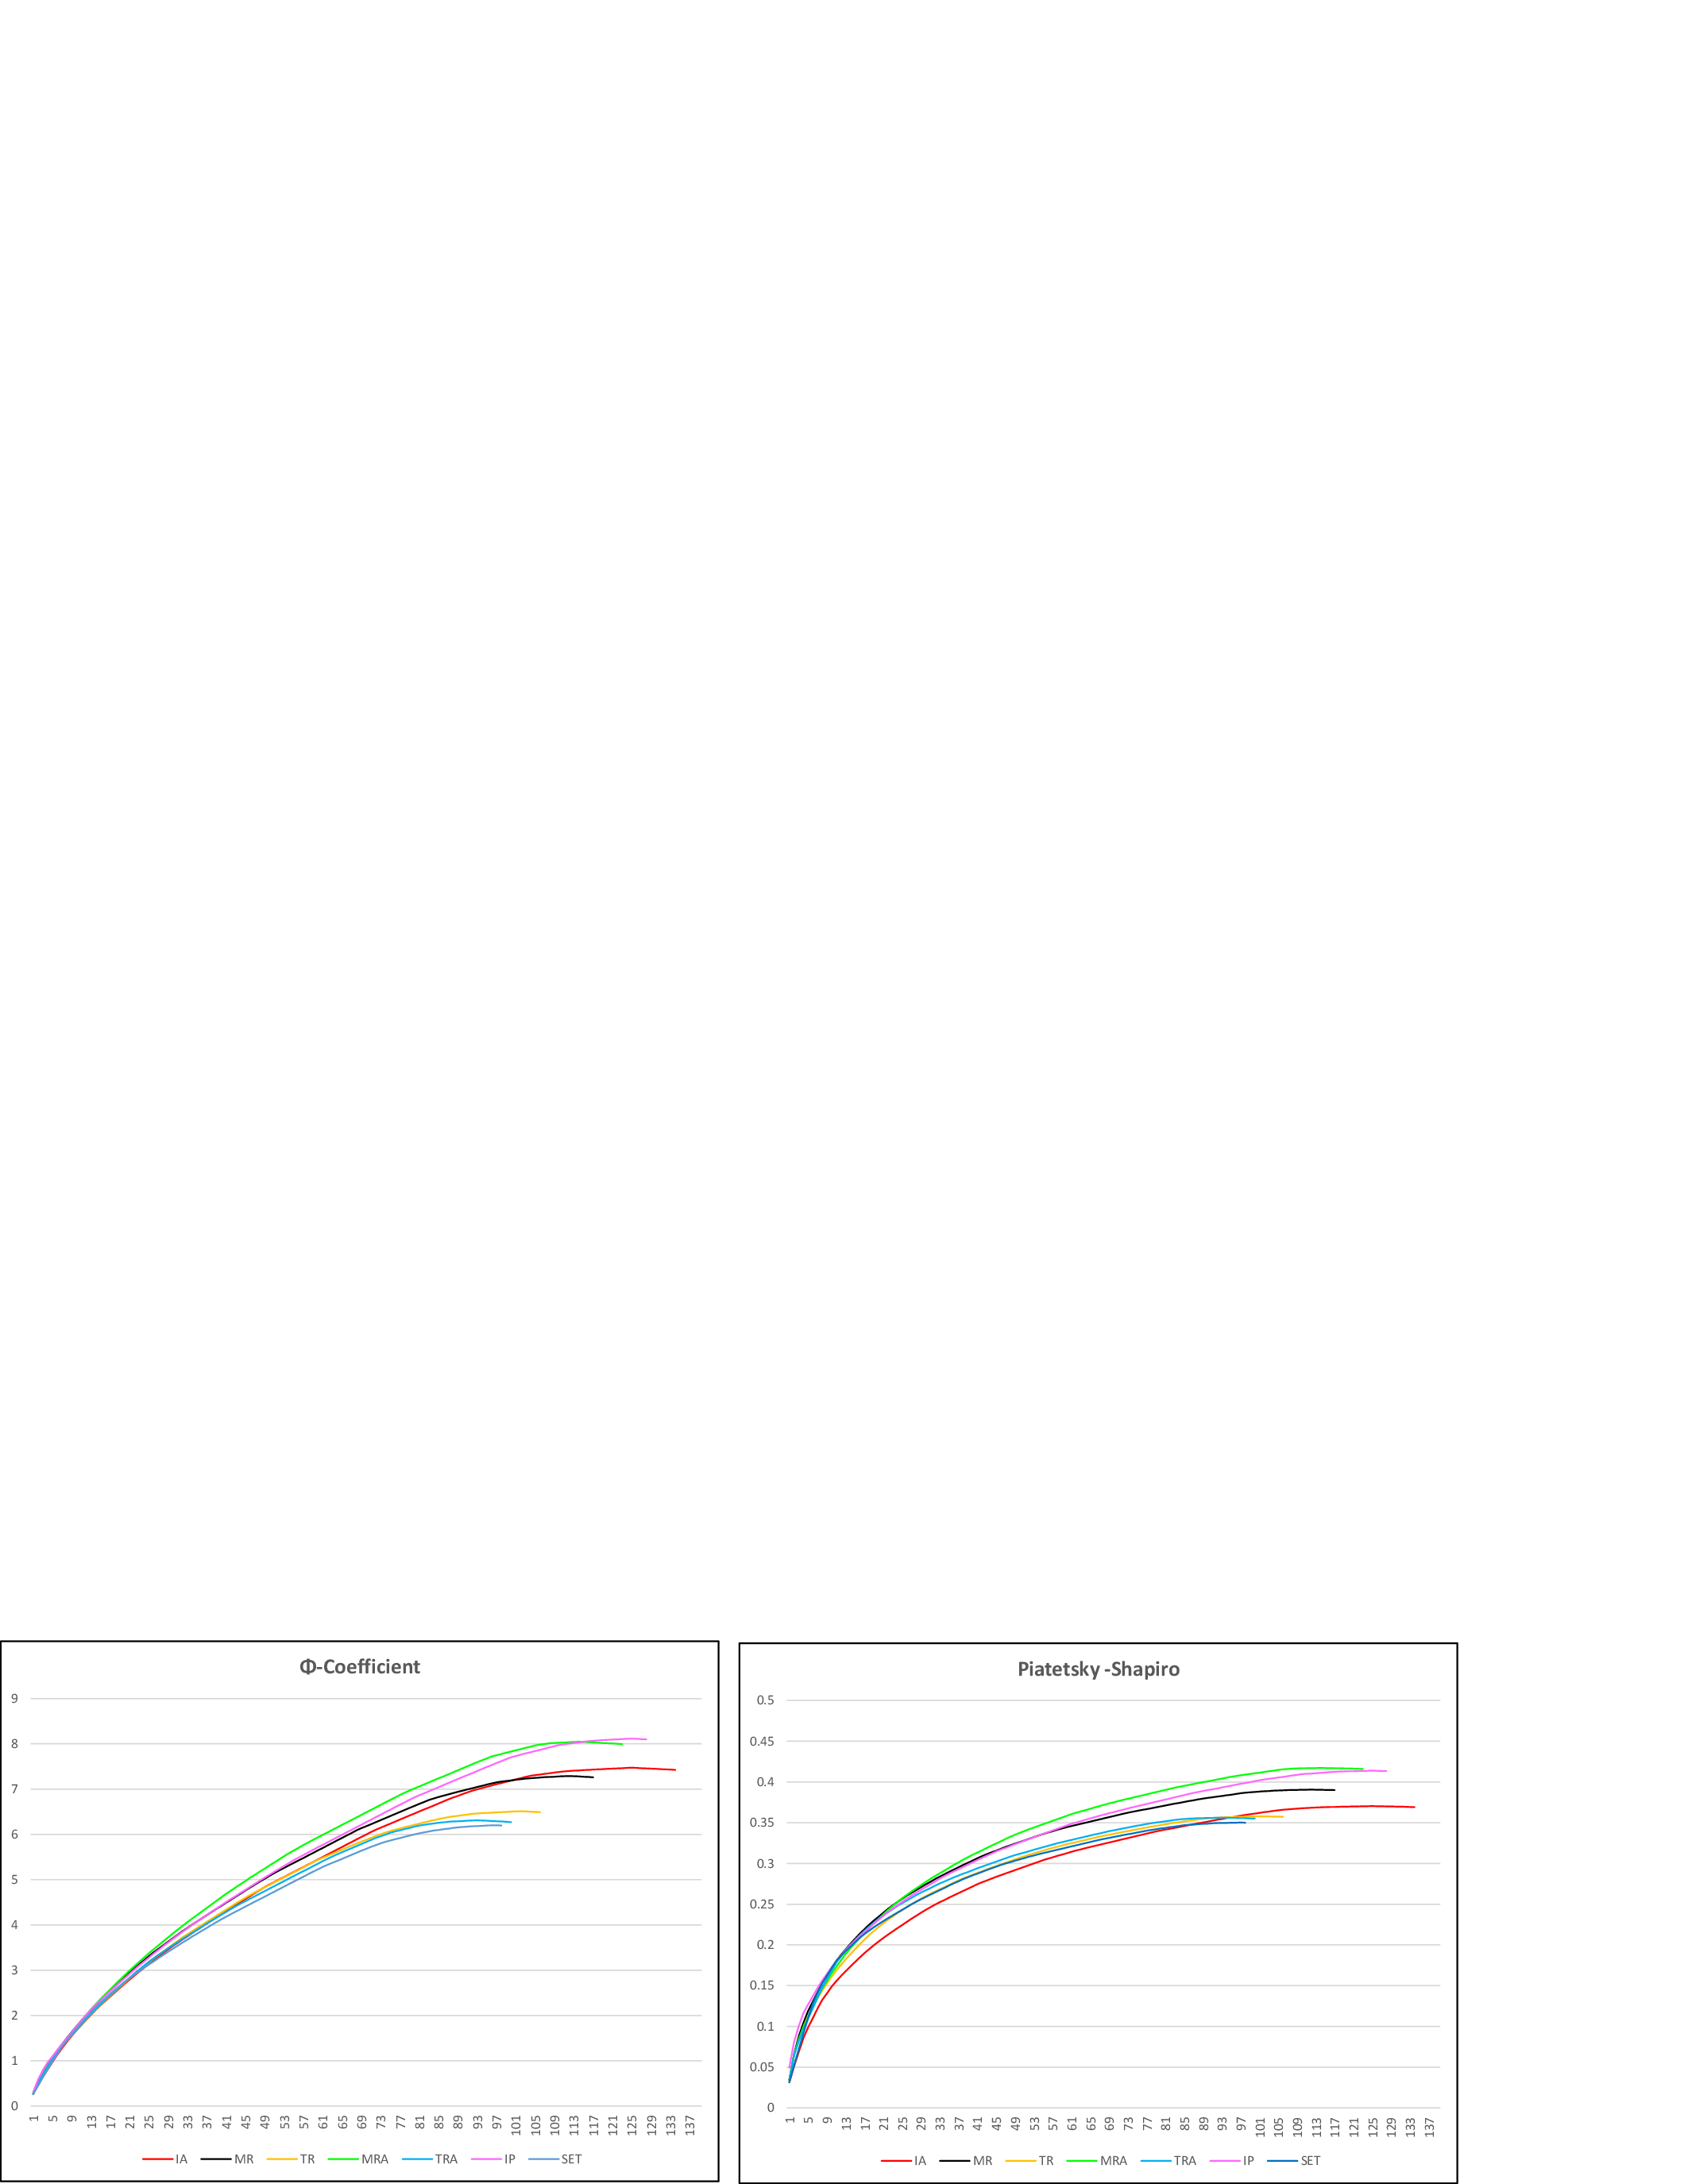}}
	\caption{Hospital1 dataset - \(\phi\)-Coefficient and Piatetsky-Shapiro}
	\label{fig:hospital1-interest3}	
\end{figure}
	
\begin{figure}[!htb]
	{\includegraphics[width=\textwidth]{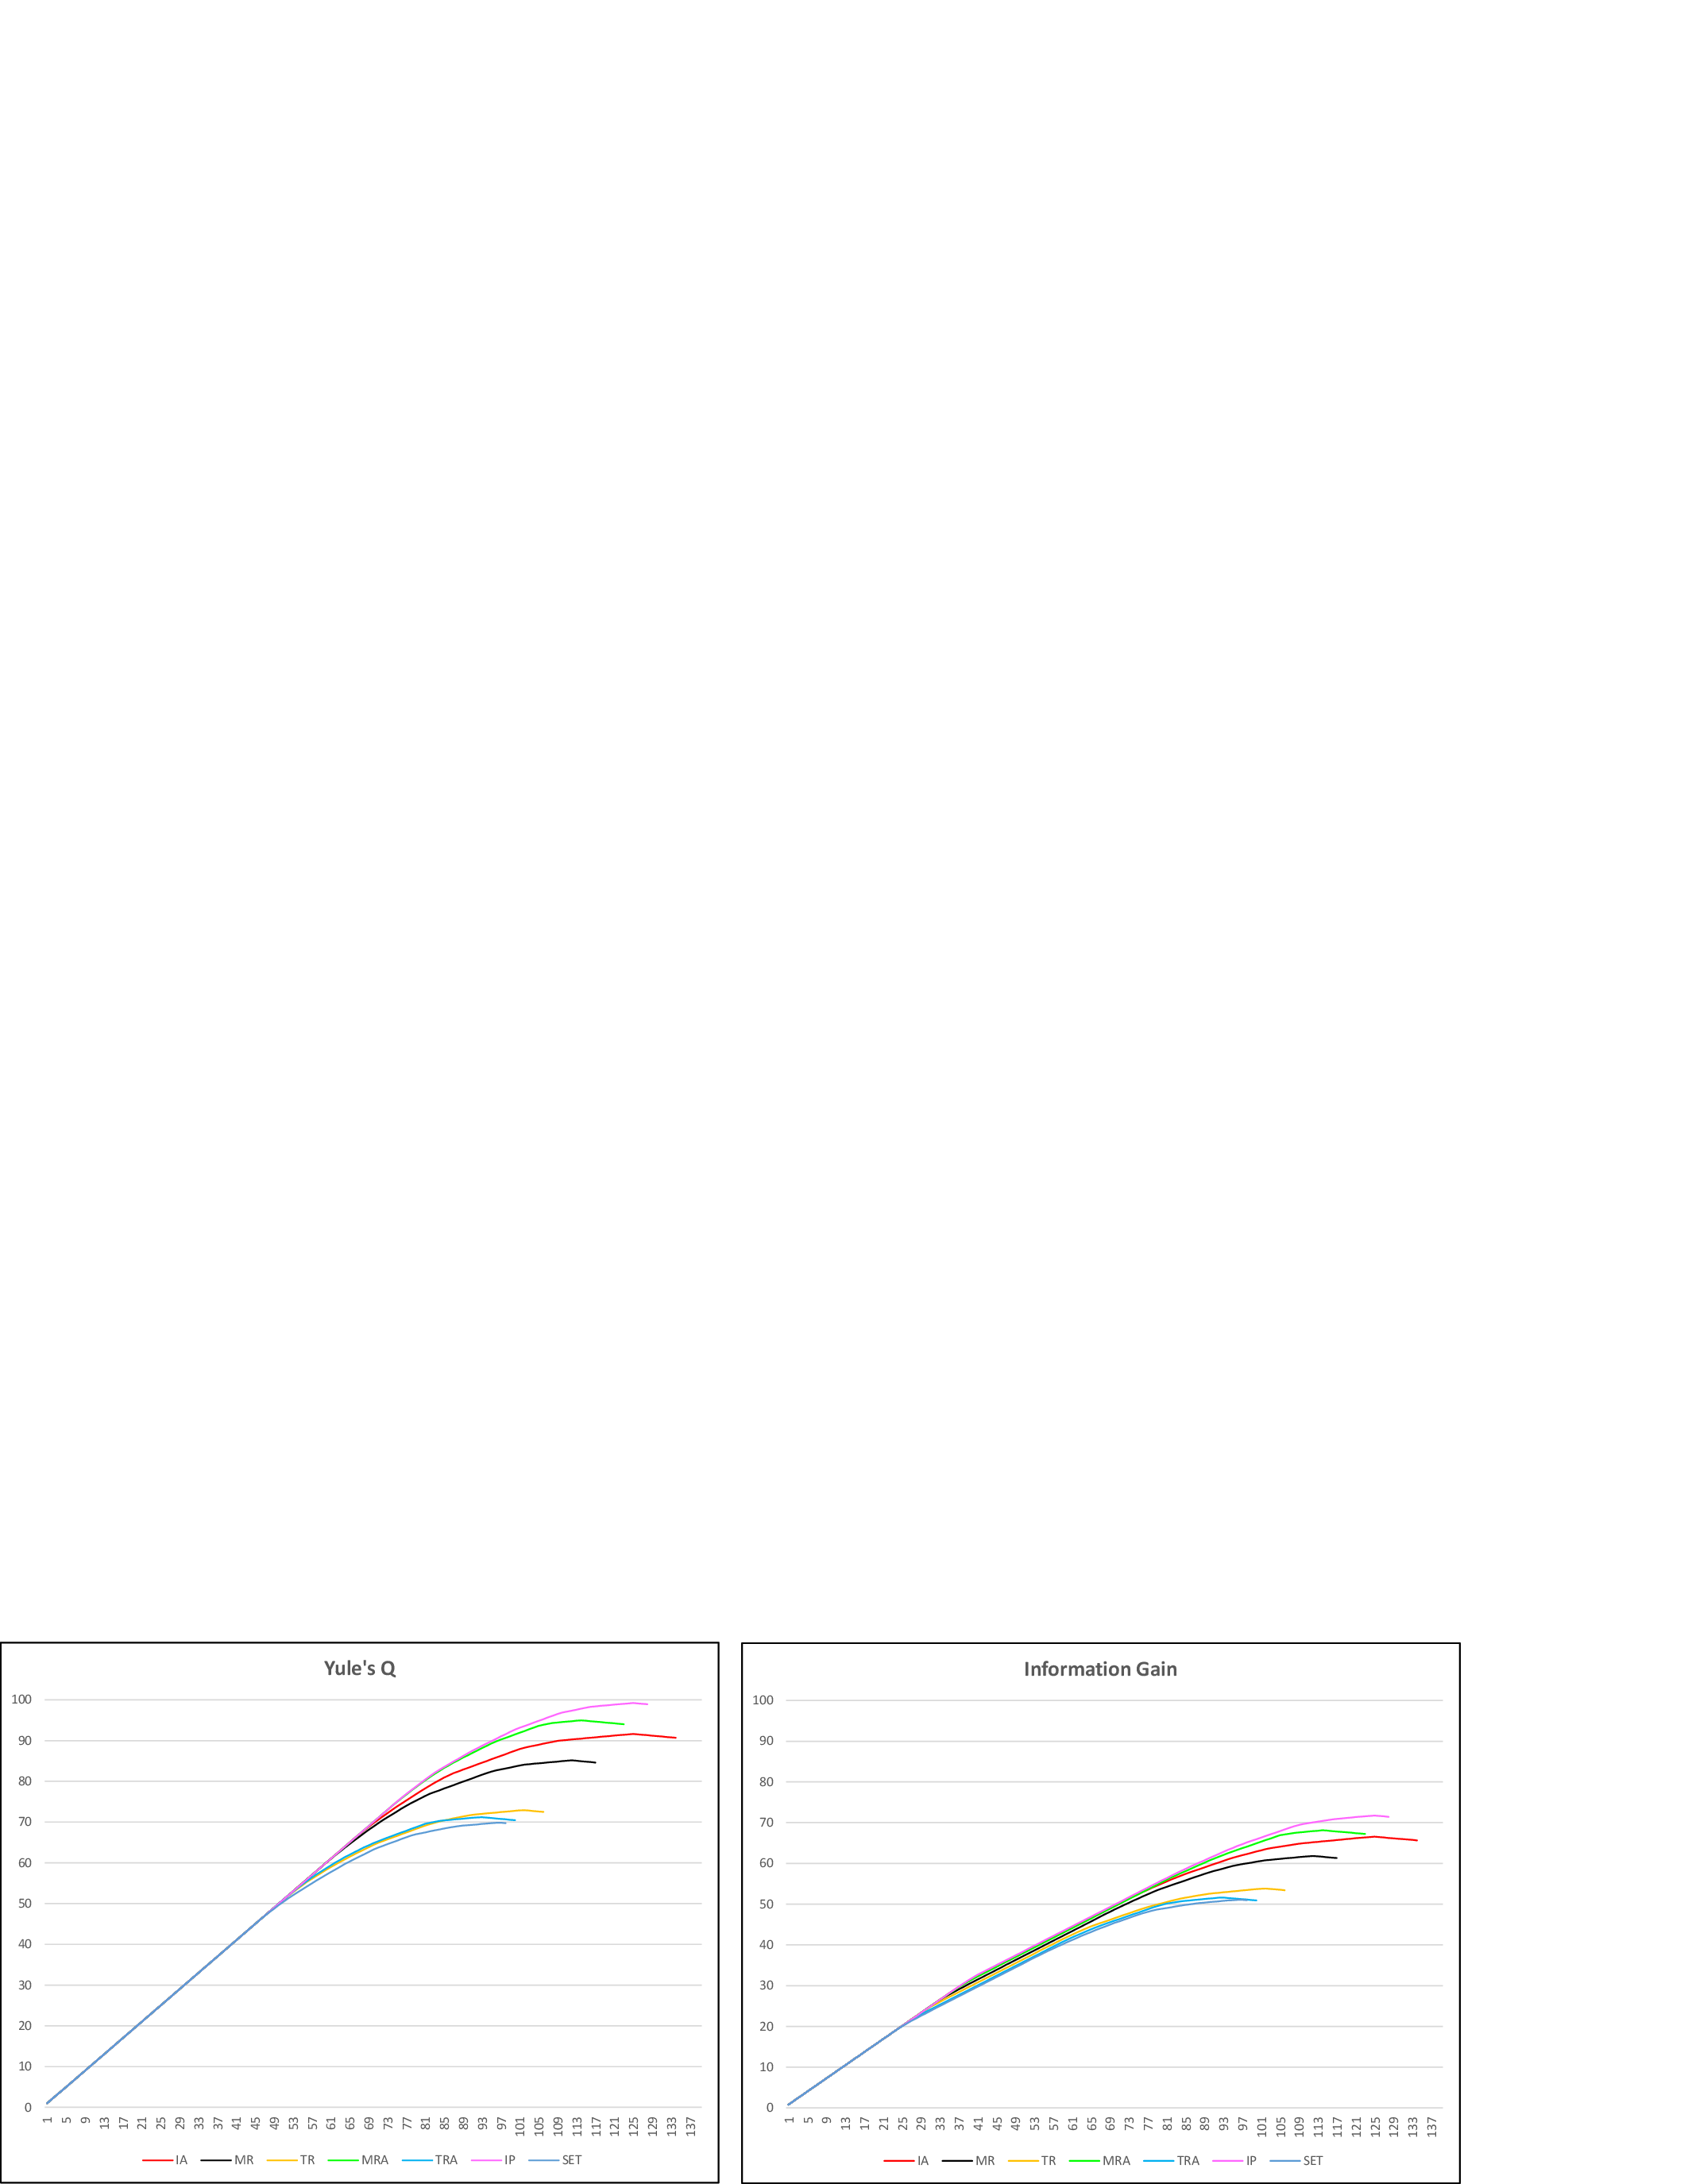}}
	\caption{Hospital1 dataset - Yule's Q and Information Gain}
	\label{fig:hospital1-interest4}
\end{figure}
\FloatBarrier

\clearpage
\subsection{Hospital2 Dataset}

\FloatBarrier
\begin{figure}[!htb]
	\centering
	{\includegraphics[width=\textwidth]{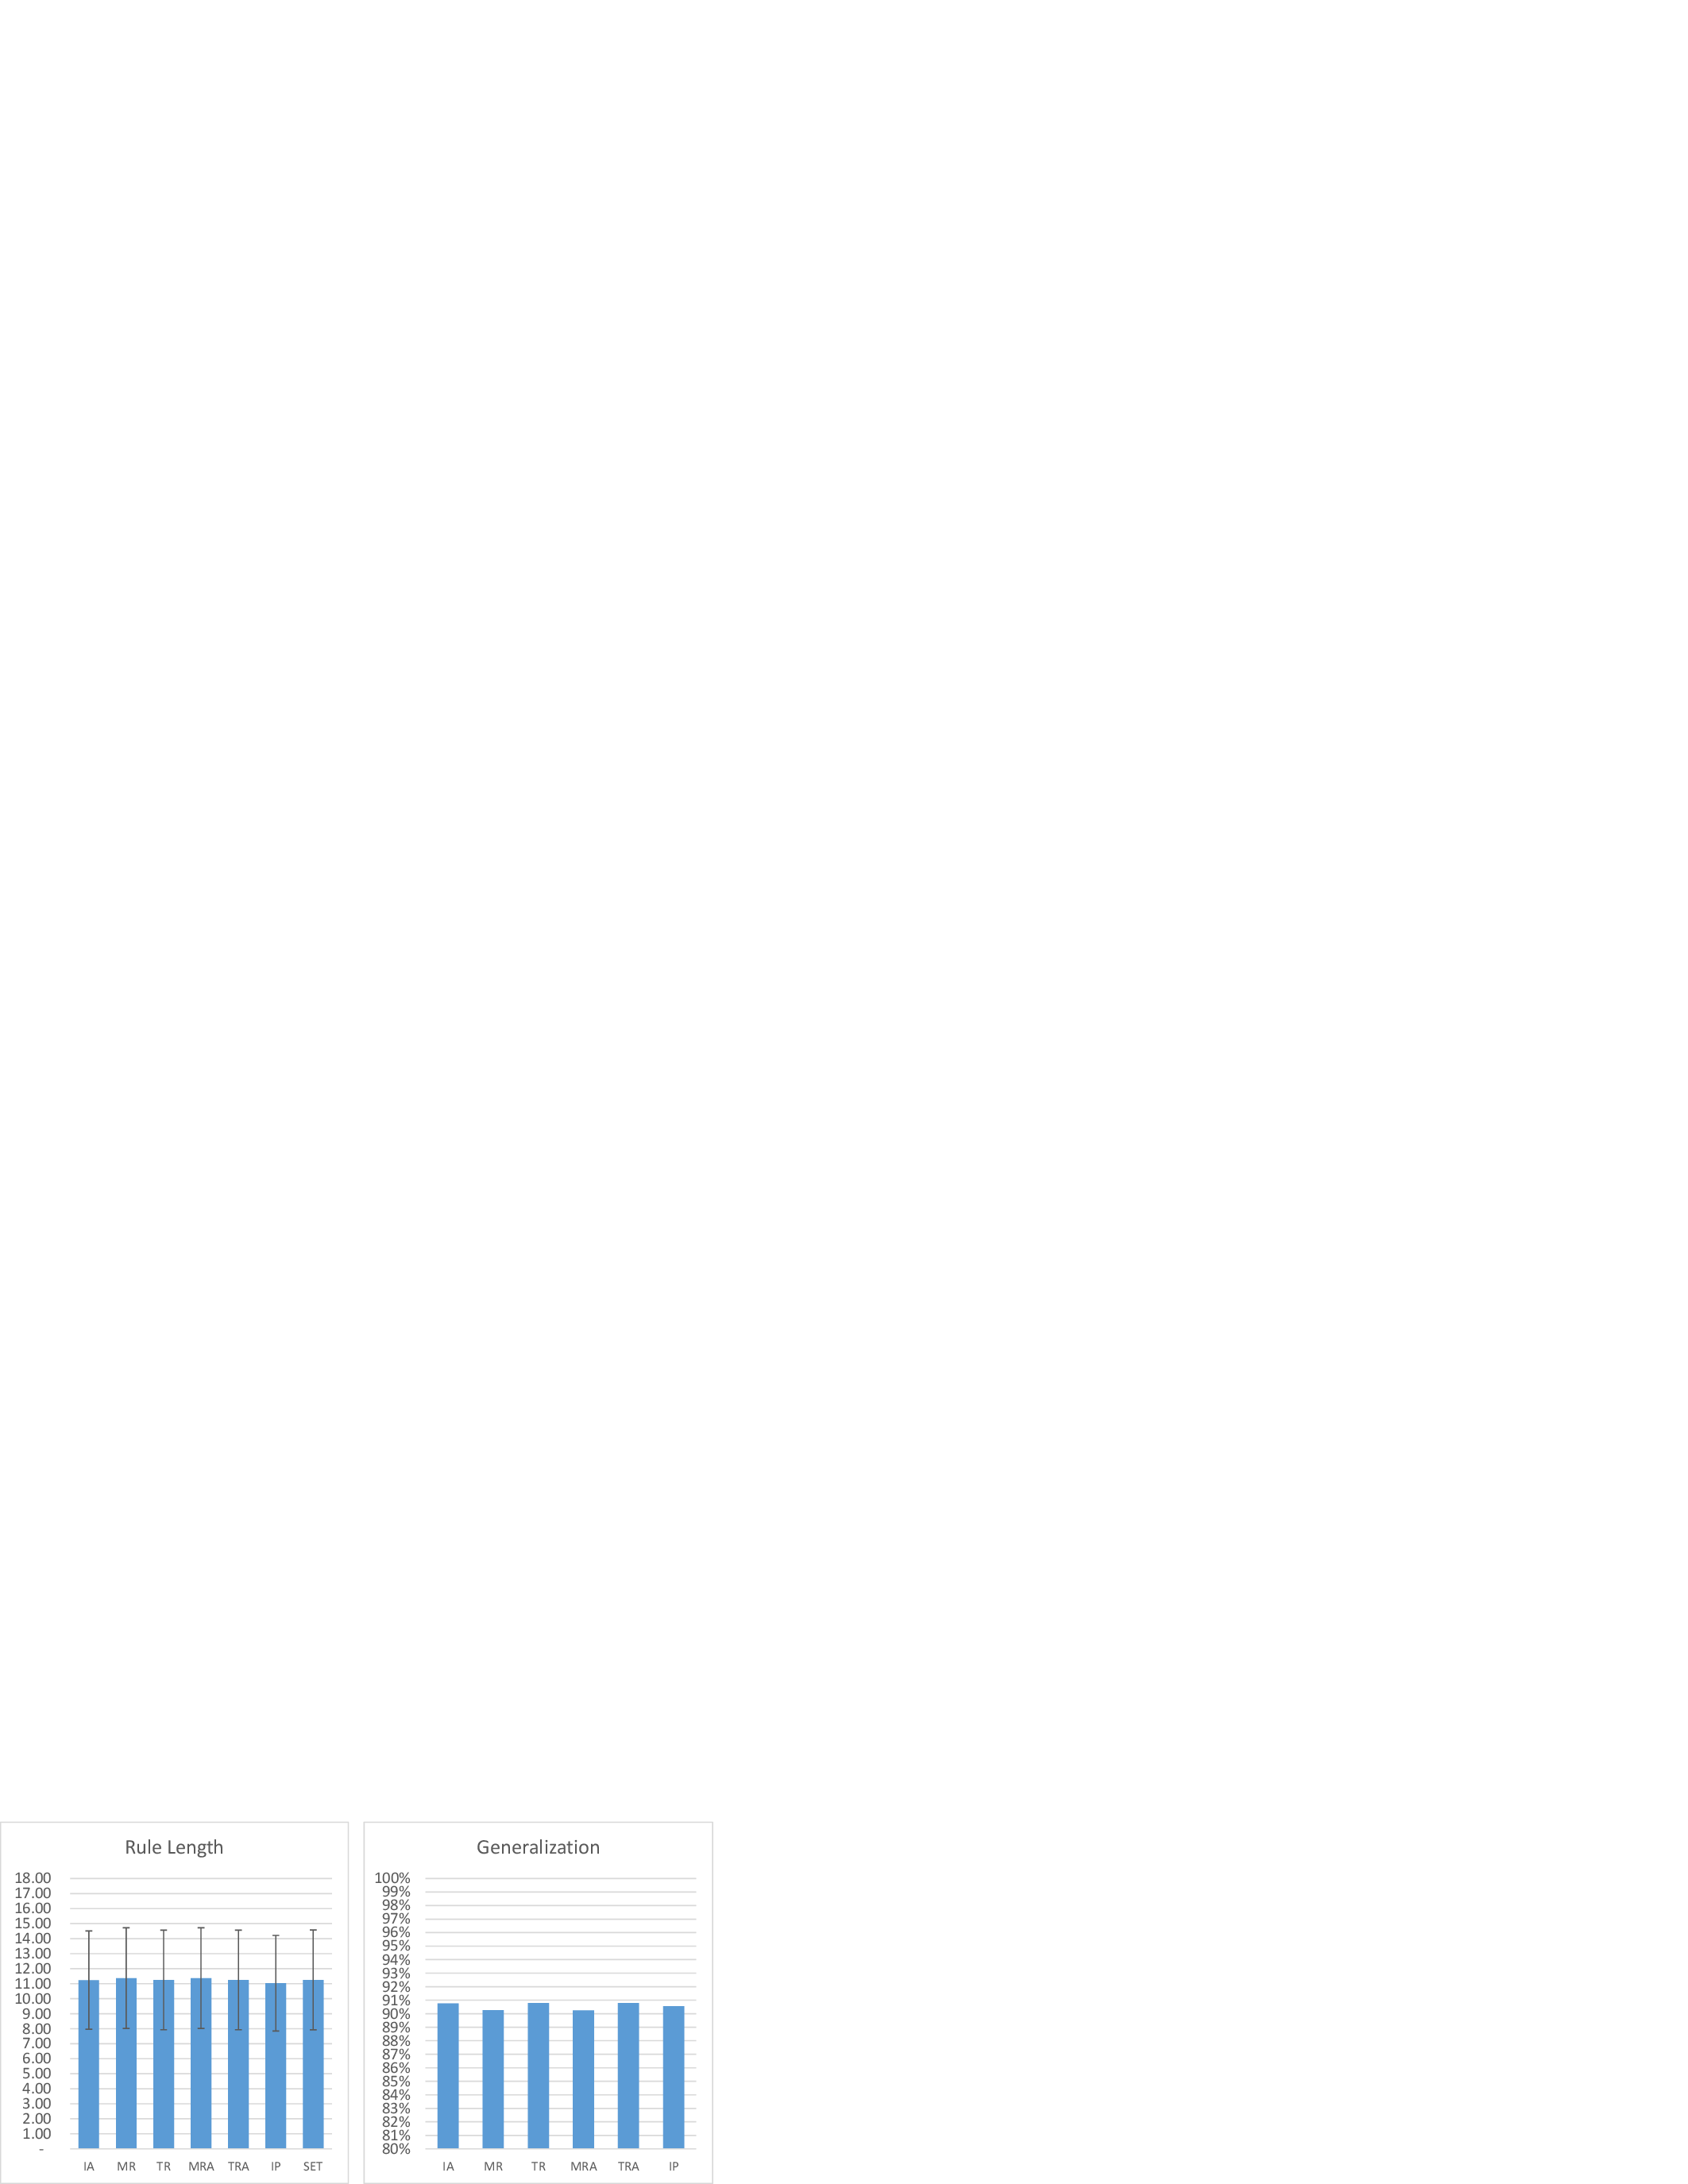}}
	\caption{Hospital2 dataset - Rule Length \& \%Generalization}
	\label{fig:hospital2-interest5}
\end{figure}
	
\begin{figure}[!htb]	
	{\includegraphics[width=\textwidth]{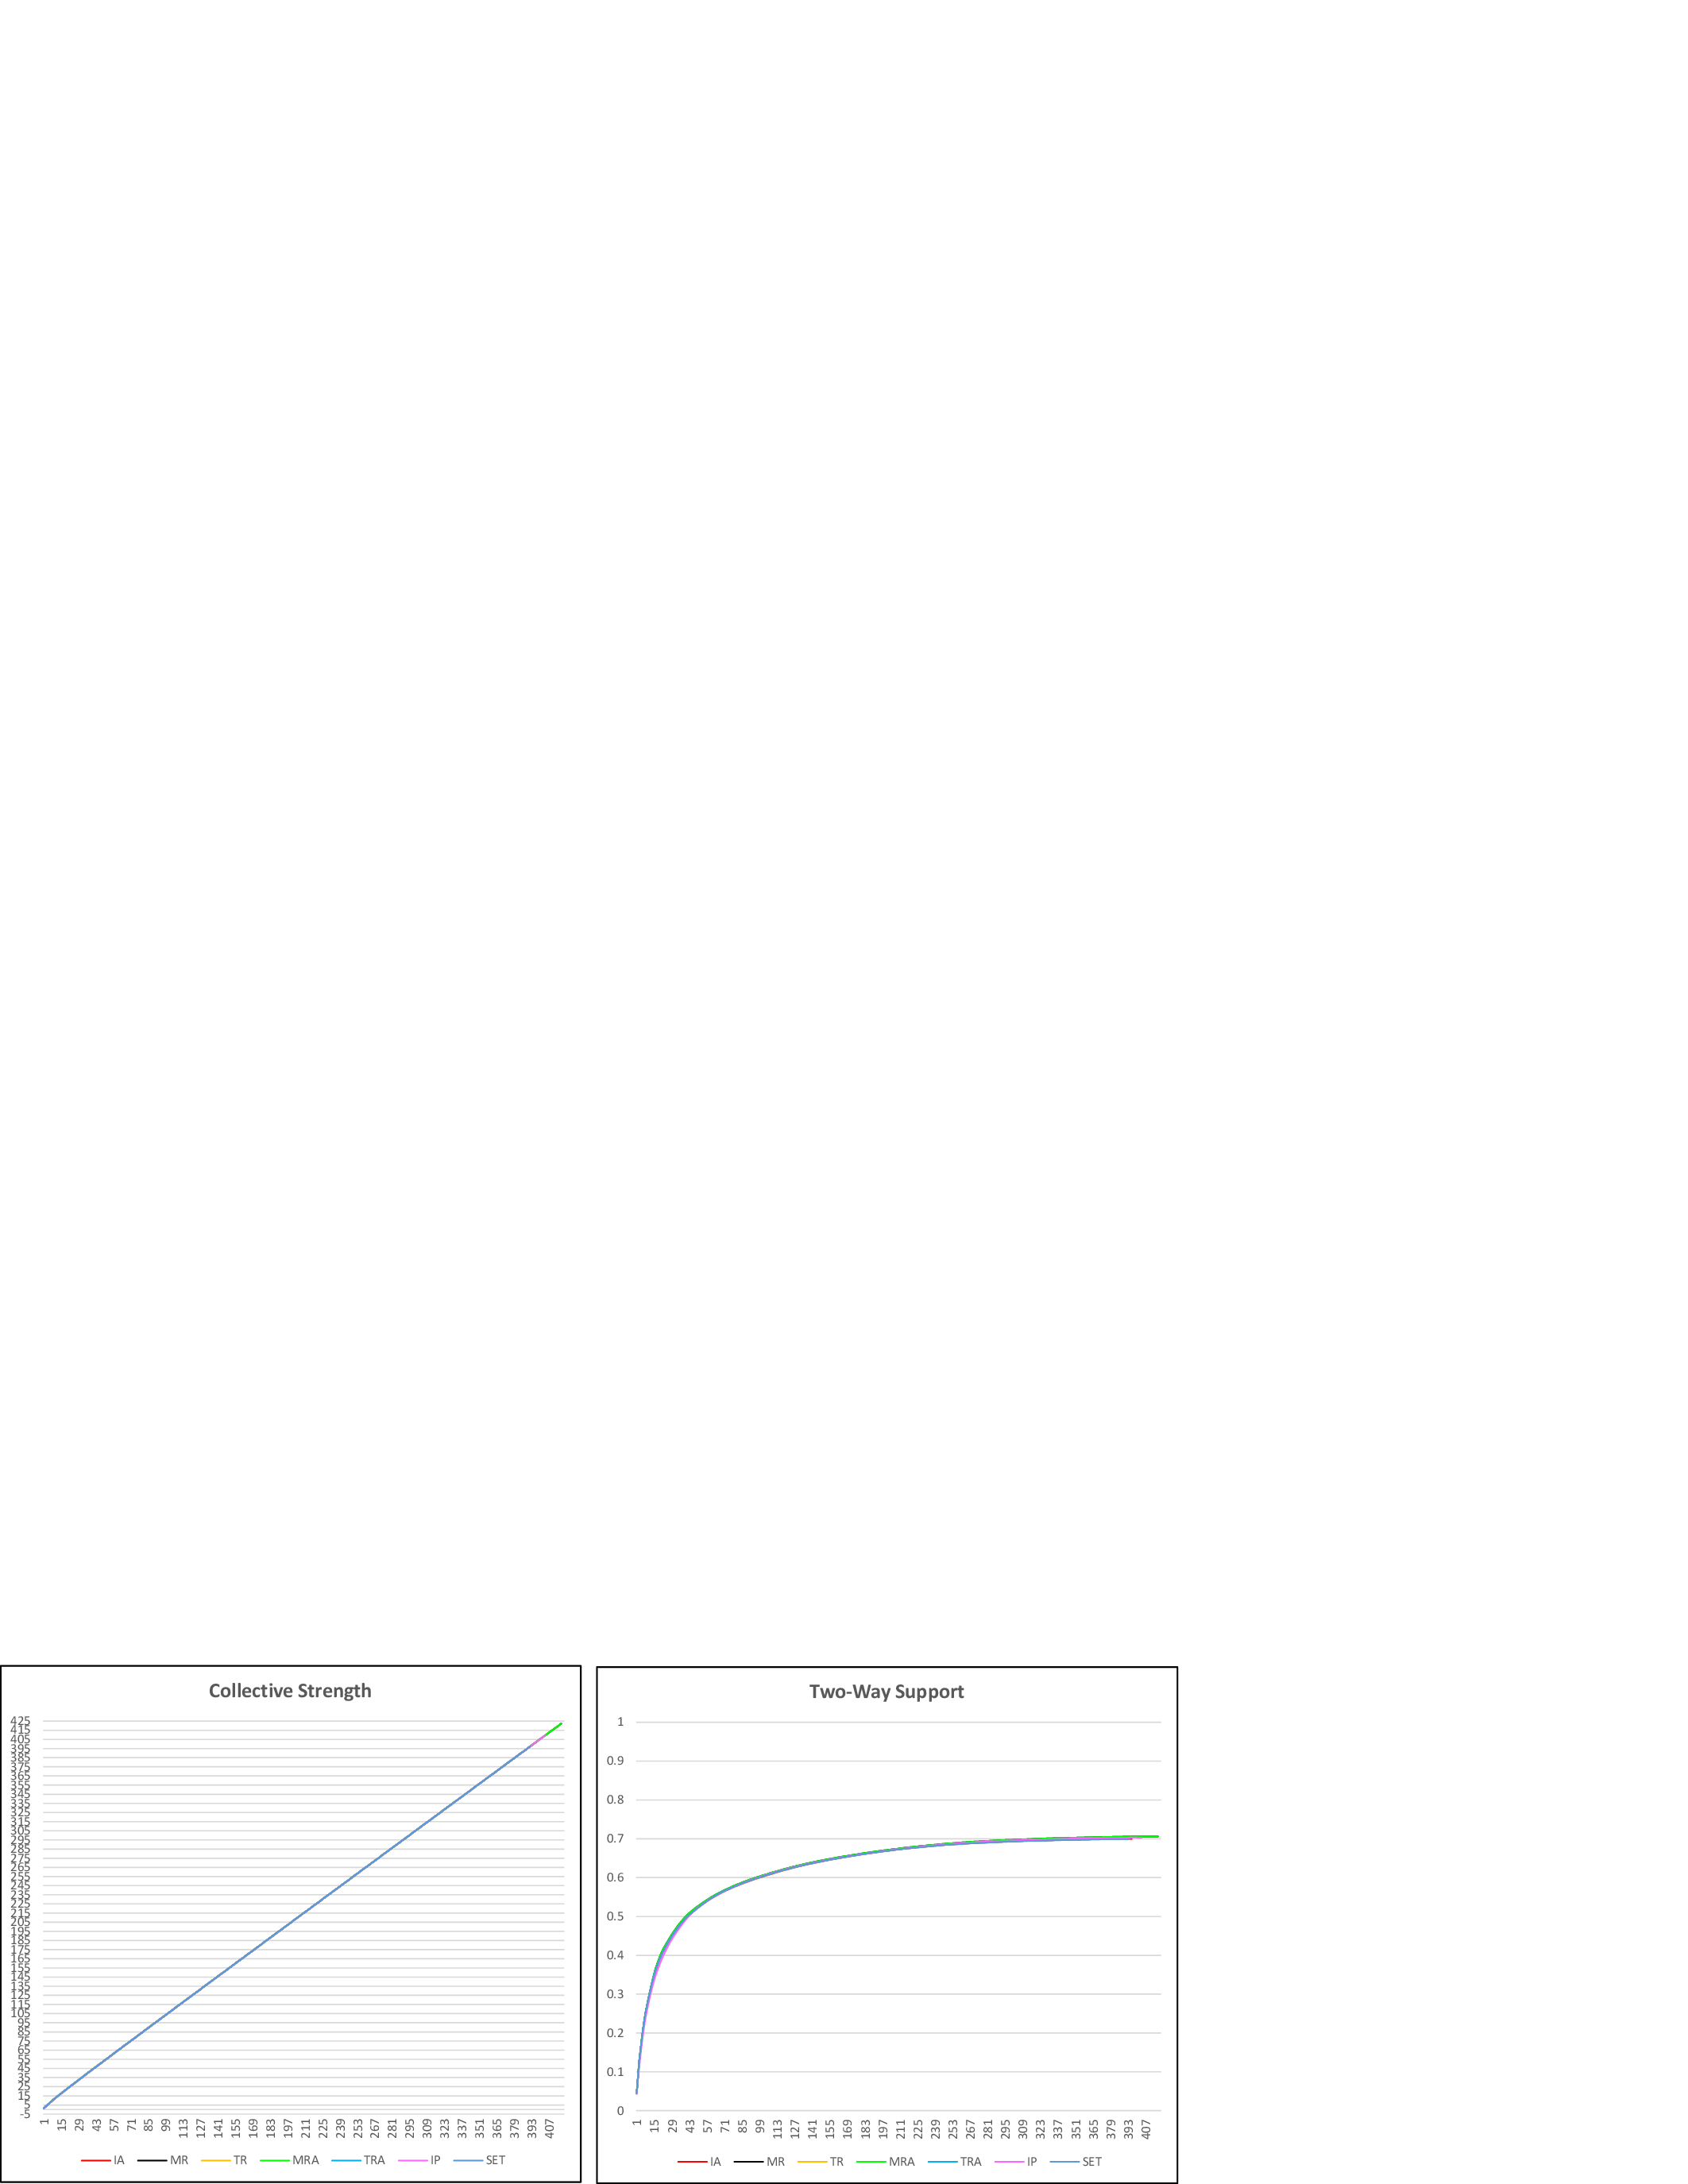}}
	\caption{Hospital2 dataset - Collective Strength and Two-Way Support}
	\label{fig:hospital2-interest2}	
\end{figure}

\begin{figure}[!htb]
	\centering
	
	{\includegraphics[width=\textwidth]{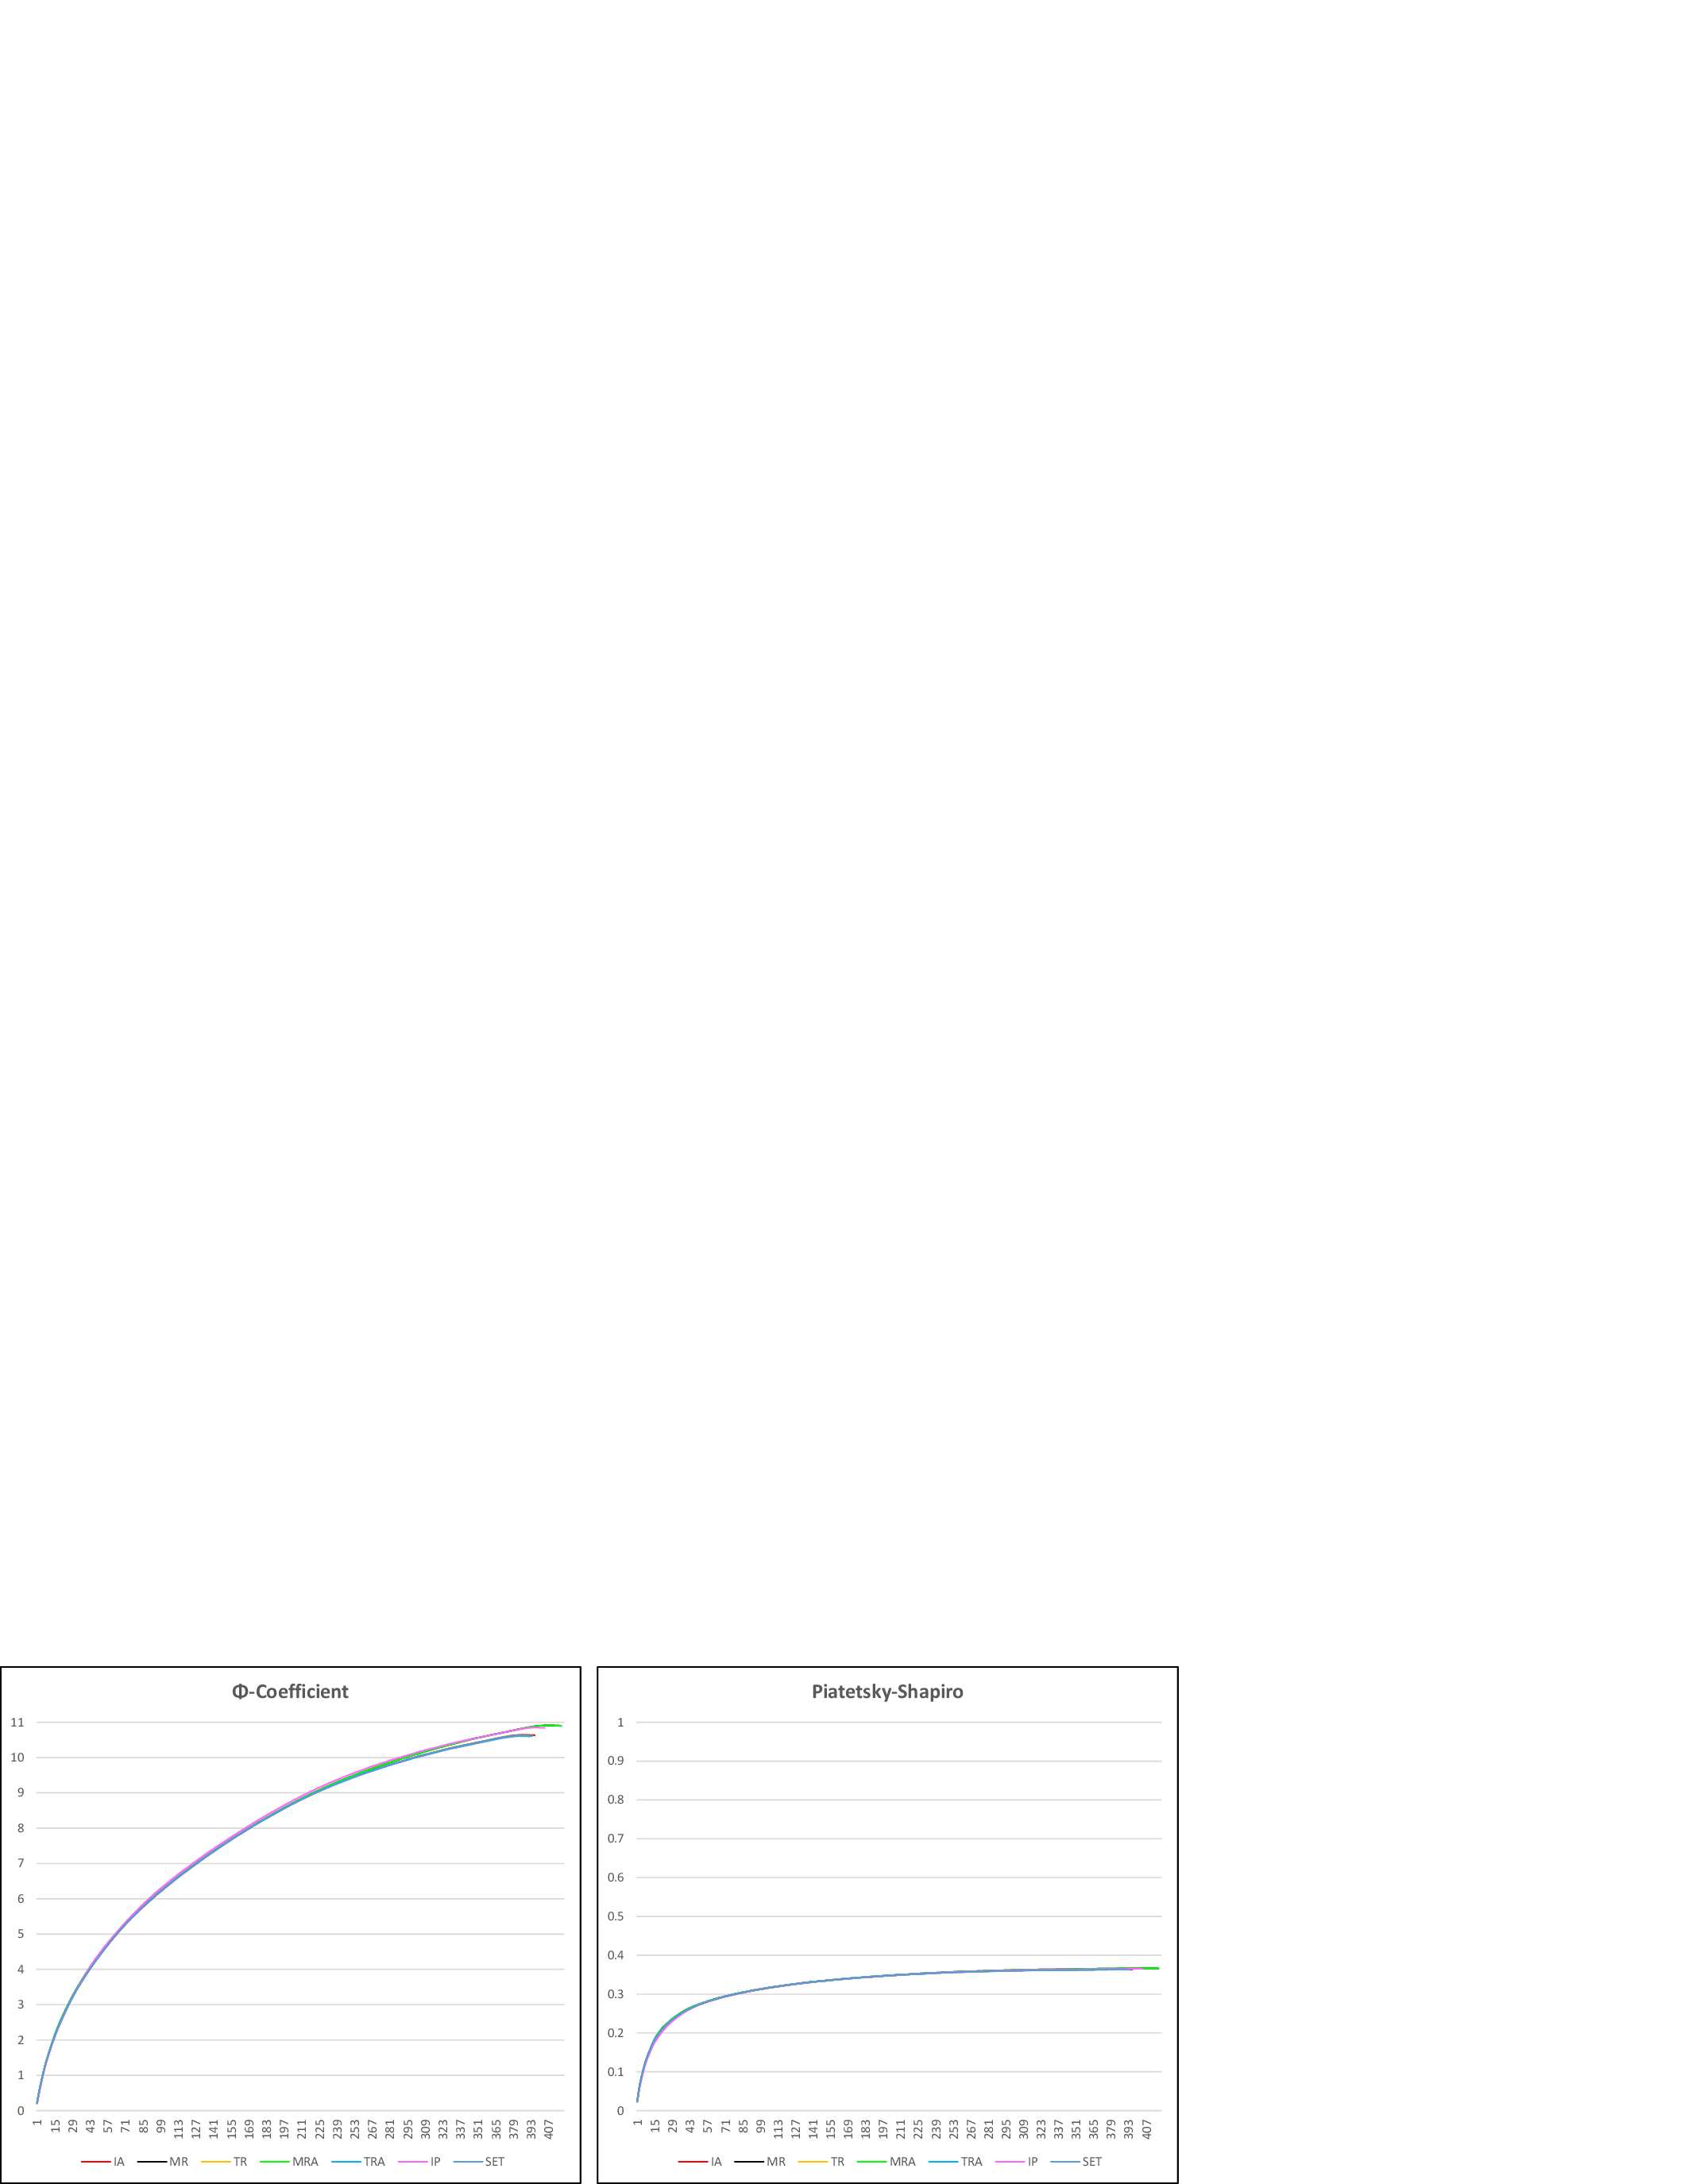}}
	\caption{Hospital2 dataset - \(\phi\)-Coefficient and Piatetsky-Shapiro}
	\label{fig:hospital2-interest3}
\end{figure}	
		
\begin{figure}[!htb]
	{\includegraphics[width=\textwidth]{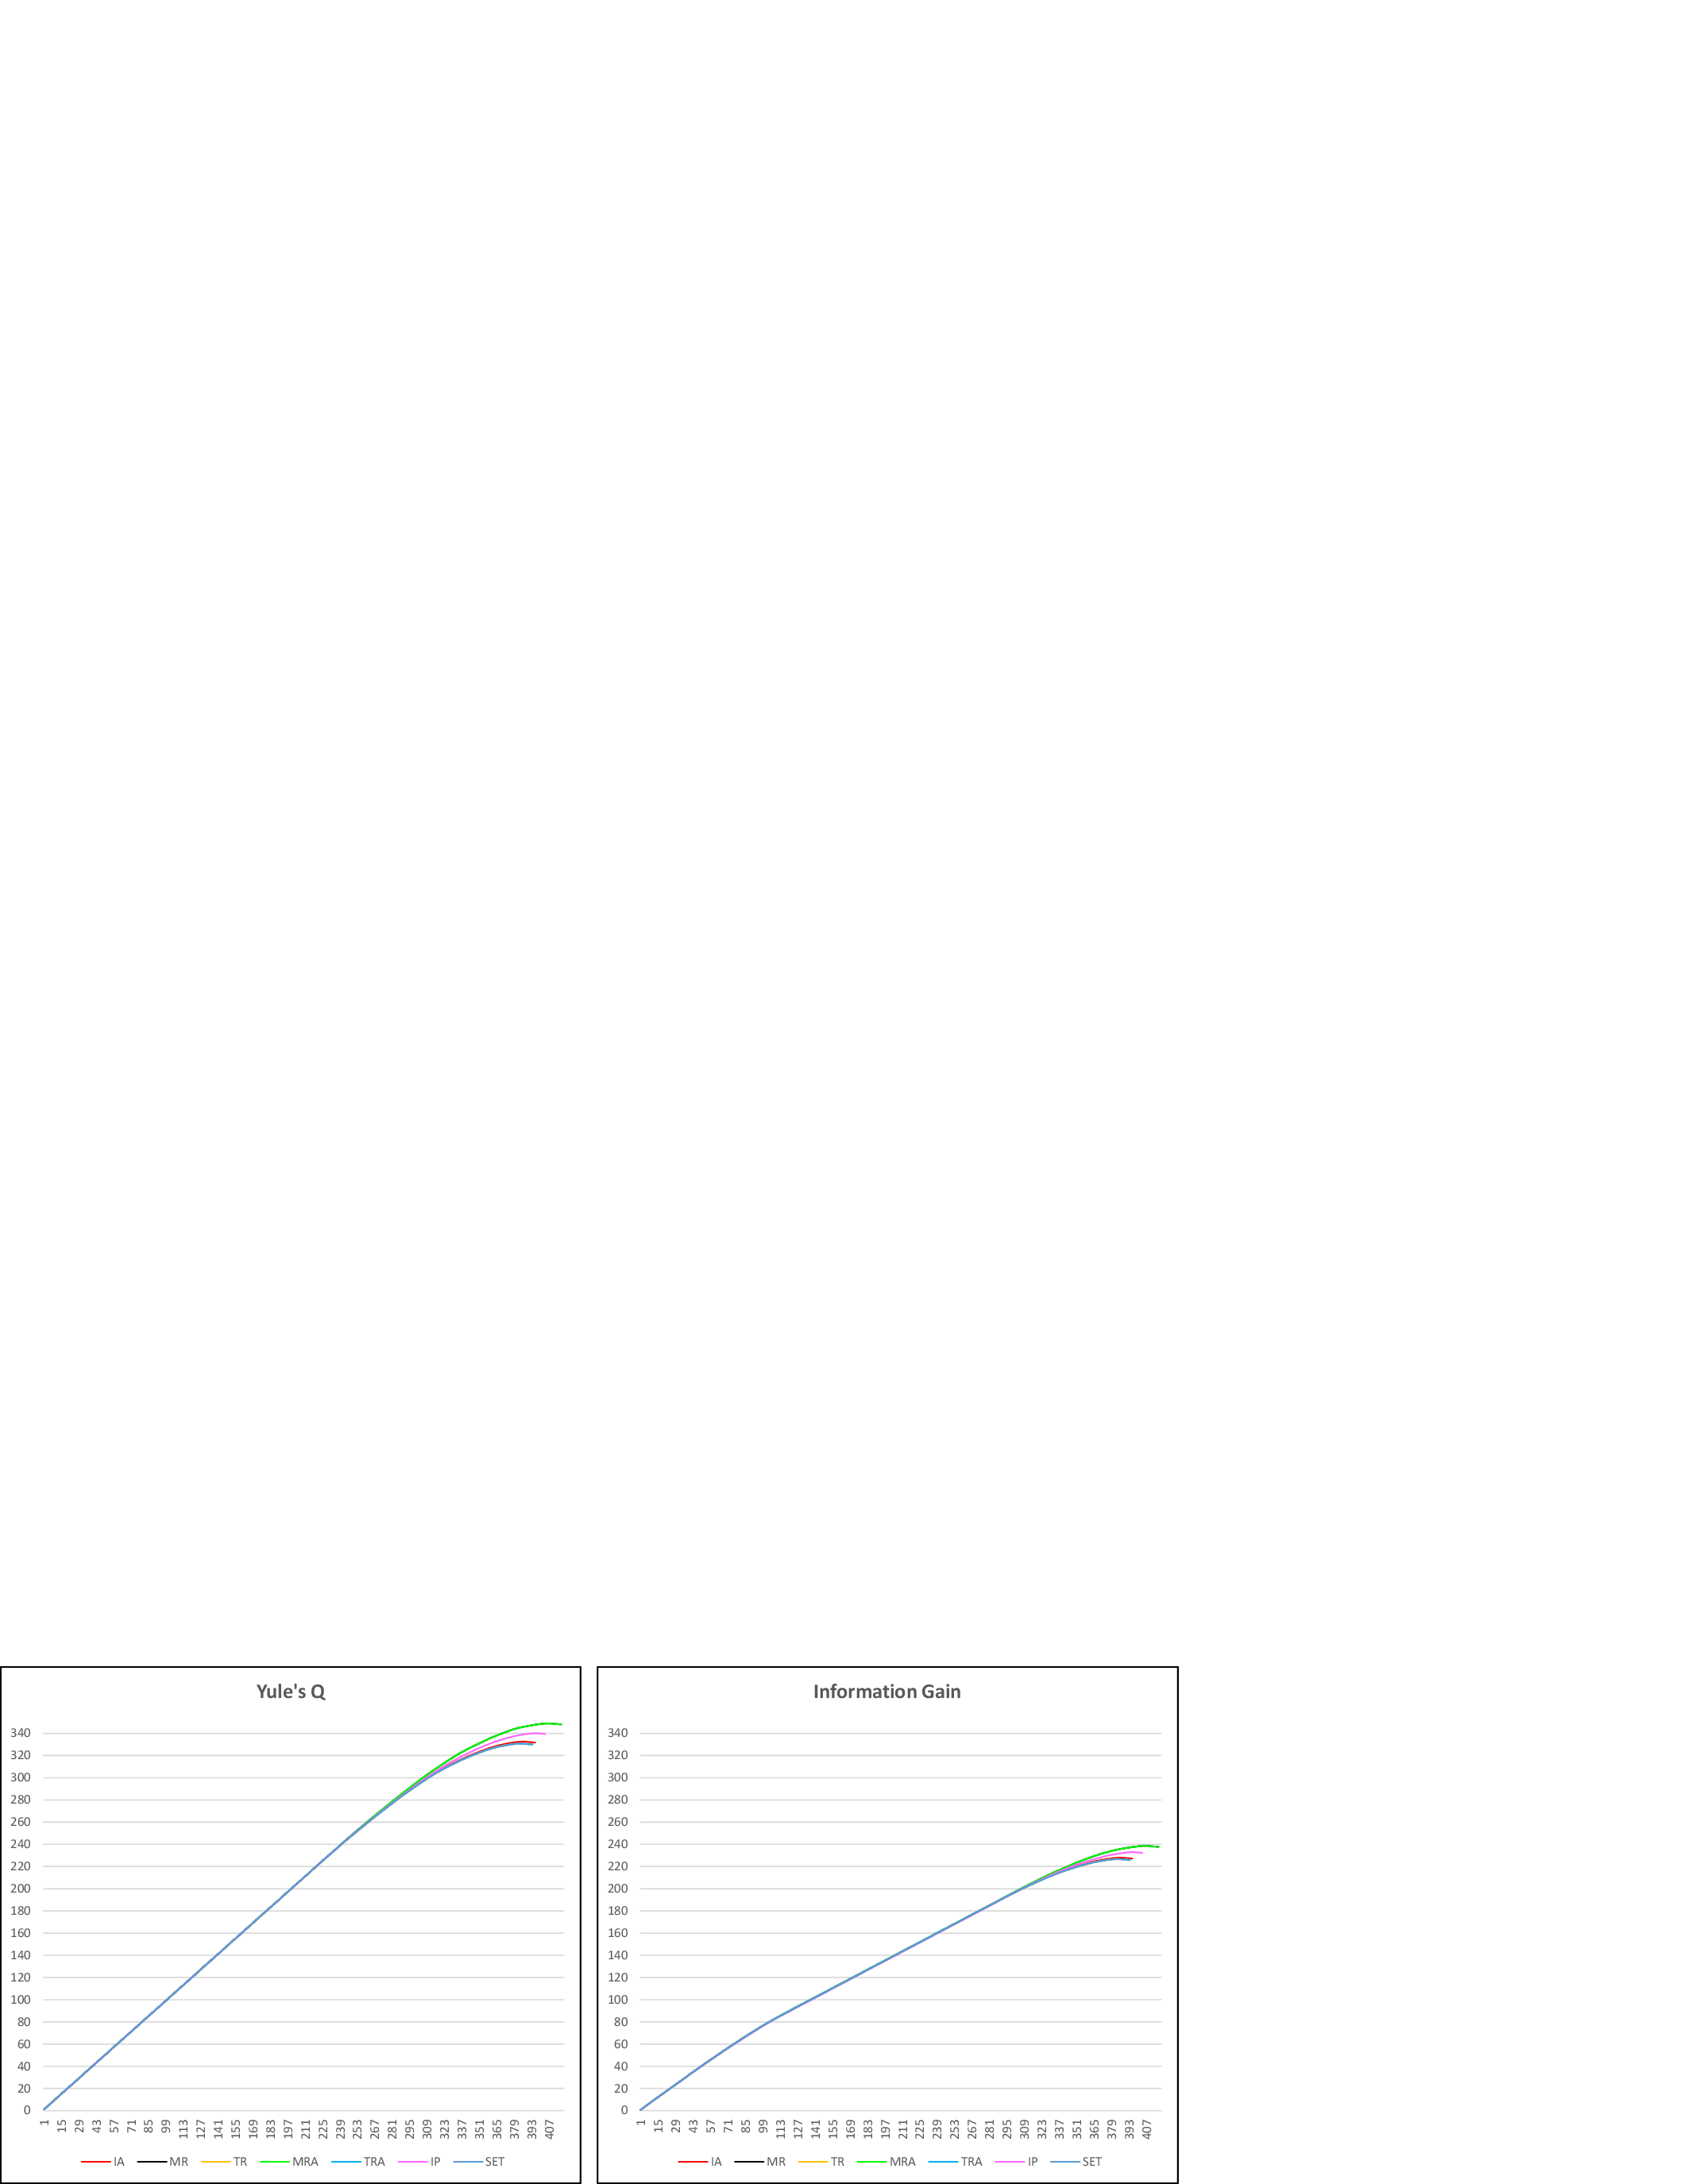}}
	\caption{Hospital2 dataset - Yule's Q and Information Gain}
	\label{fig:hospital2-interest4}
\end{figure}

\FloatBarrier

\clearpage
\subsection{Insurance1 Dataset}

\FloatBarrier
\begin{figure}[!htb]	
	\centering
	
	{\includegraphics[width=\textwidth]{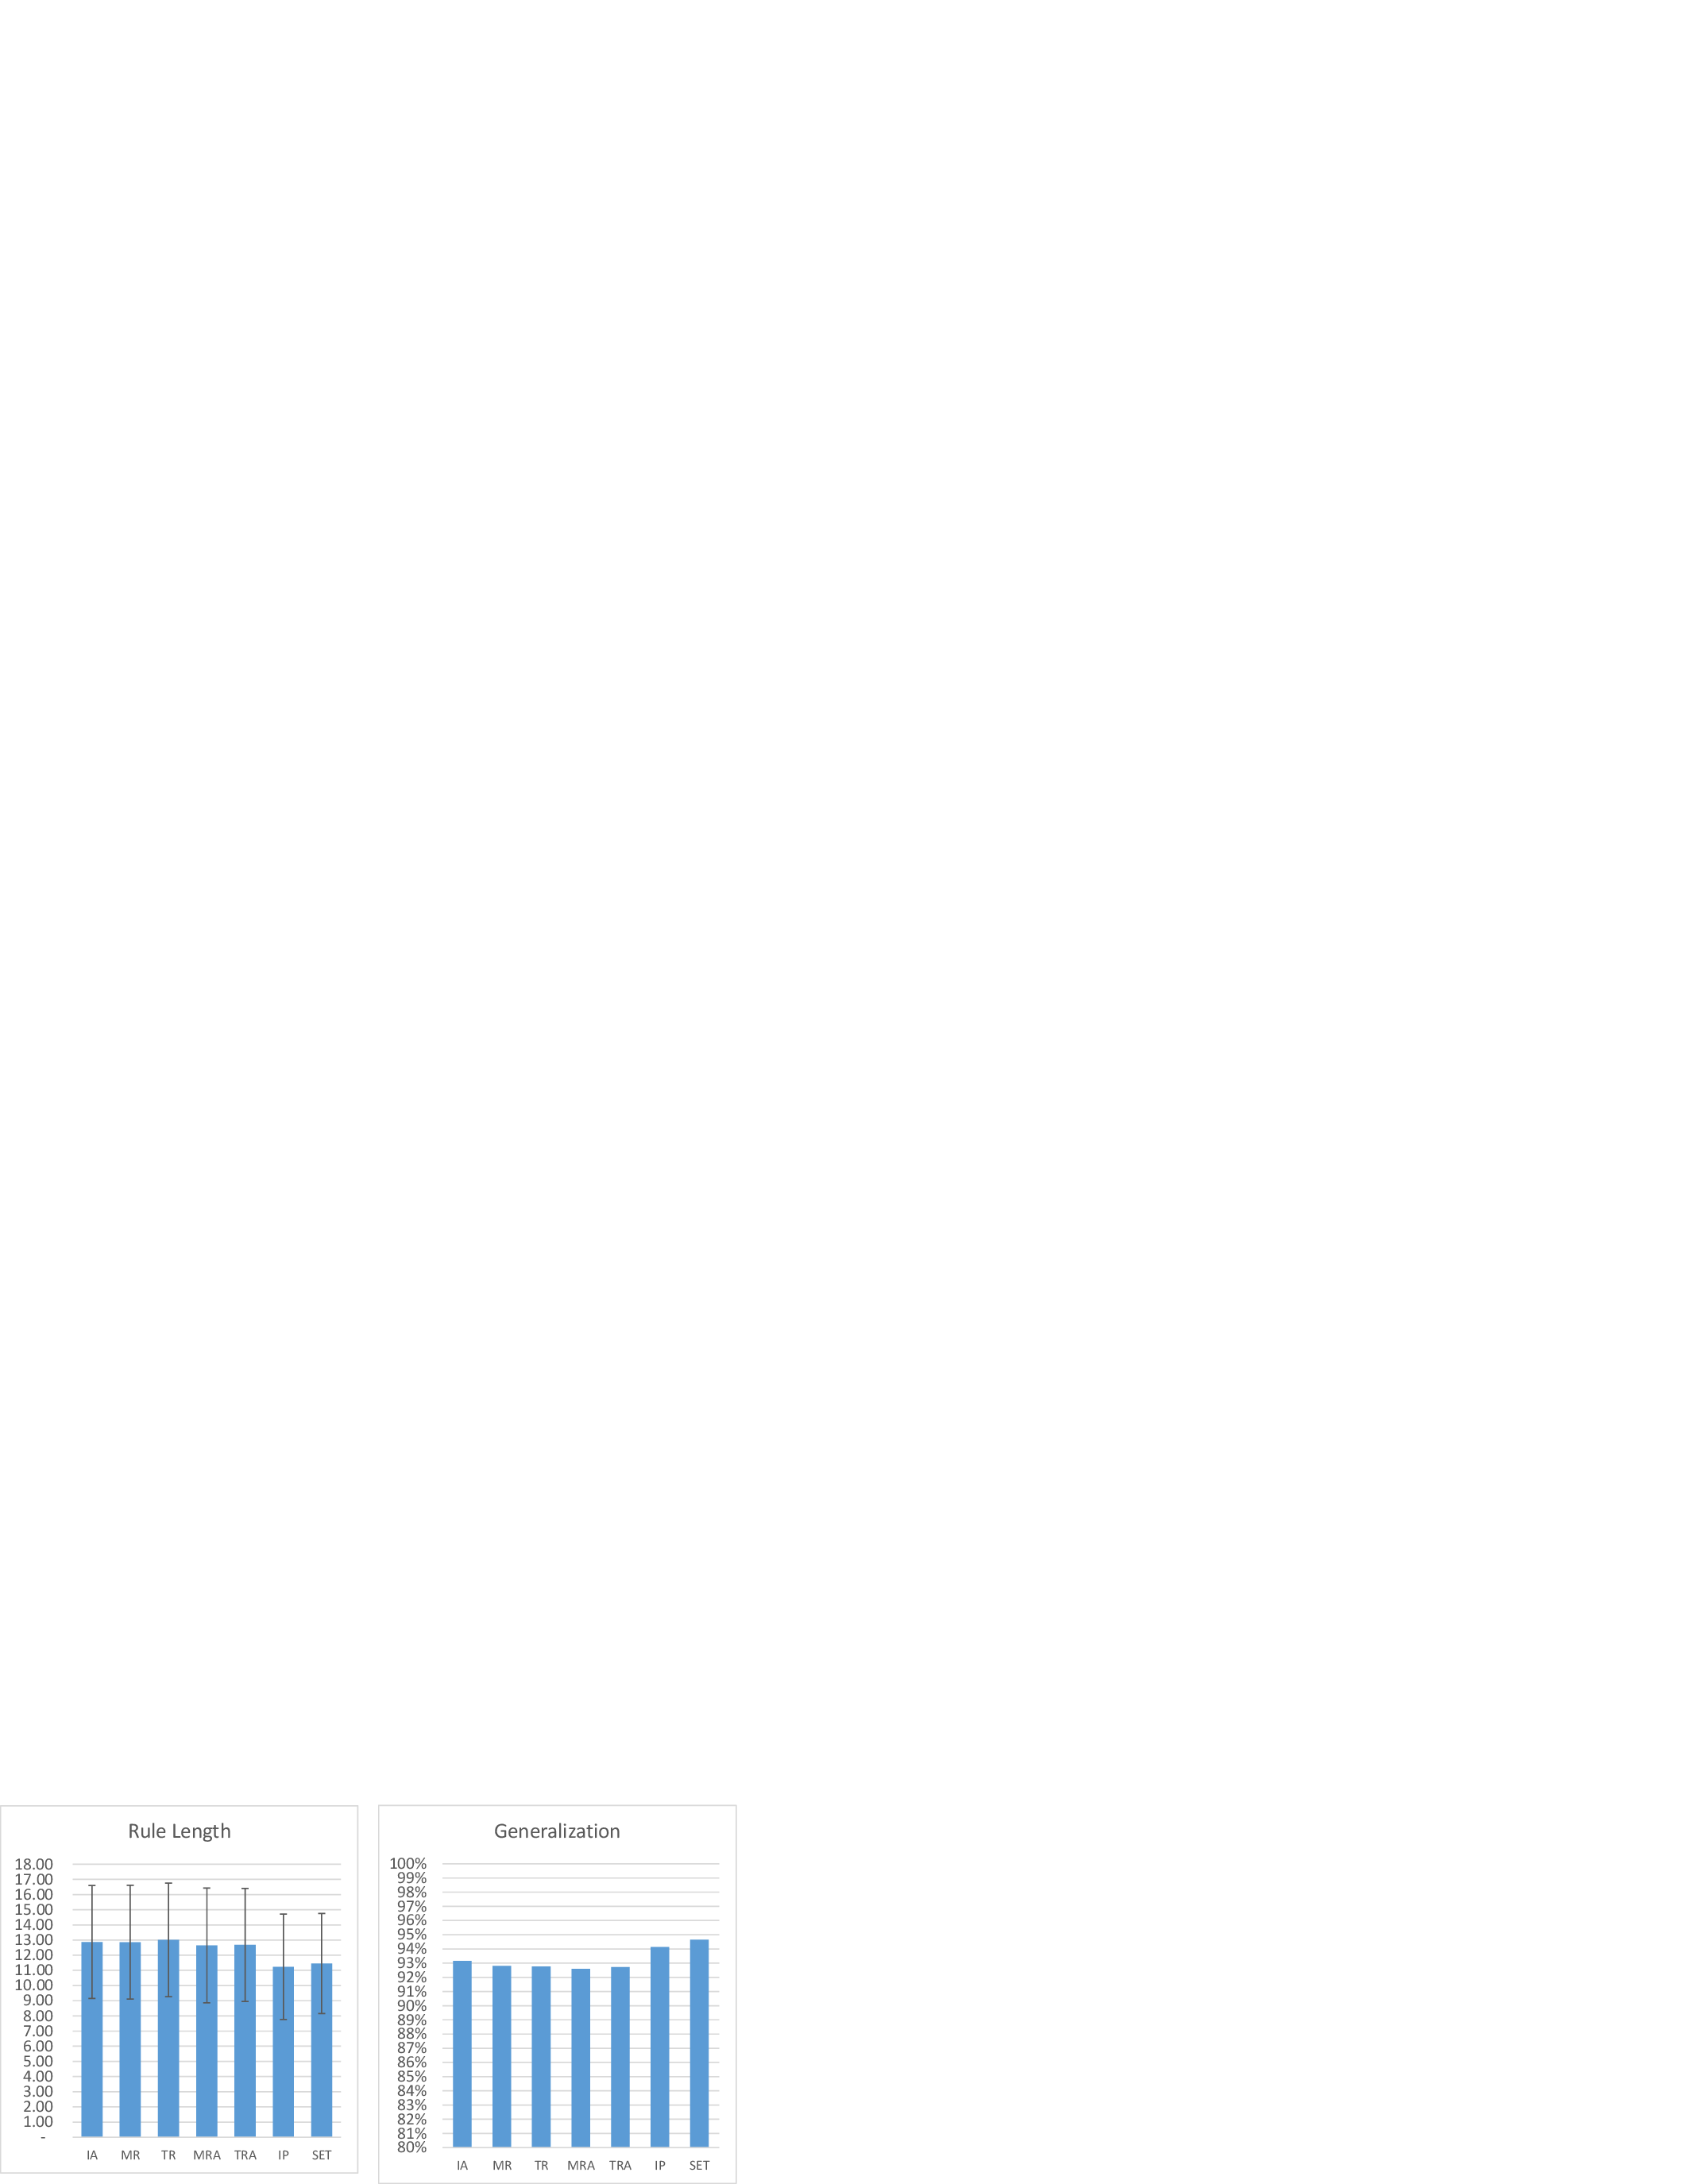}}
	\caption{Insurance1 dataset - Rule Length \& \%Generalization}
	\label{fig:insurance1-interest5}
\end{figure}
	
\begin{figure}[!htb]		
	{\includegraphics[width=\textwidth]{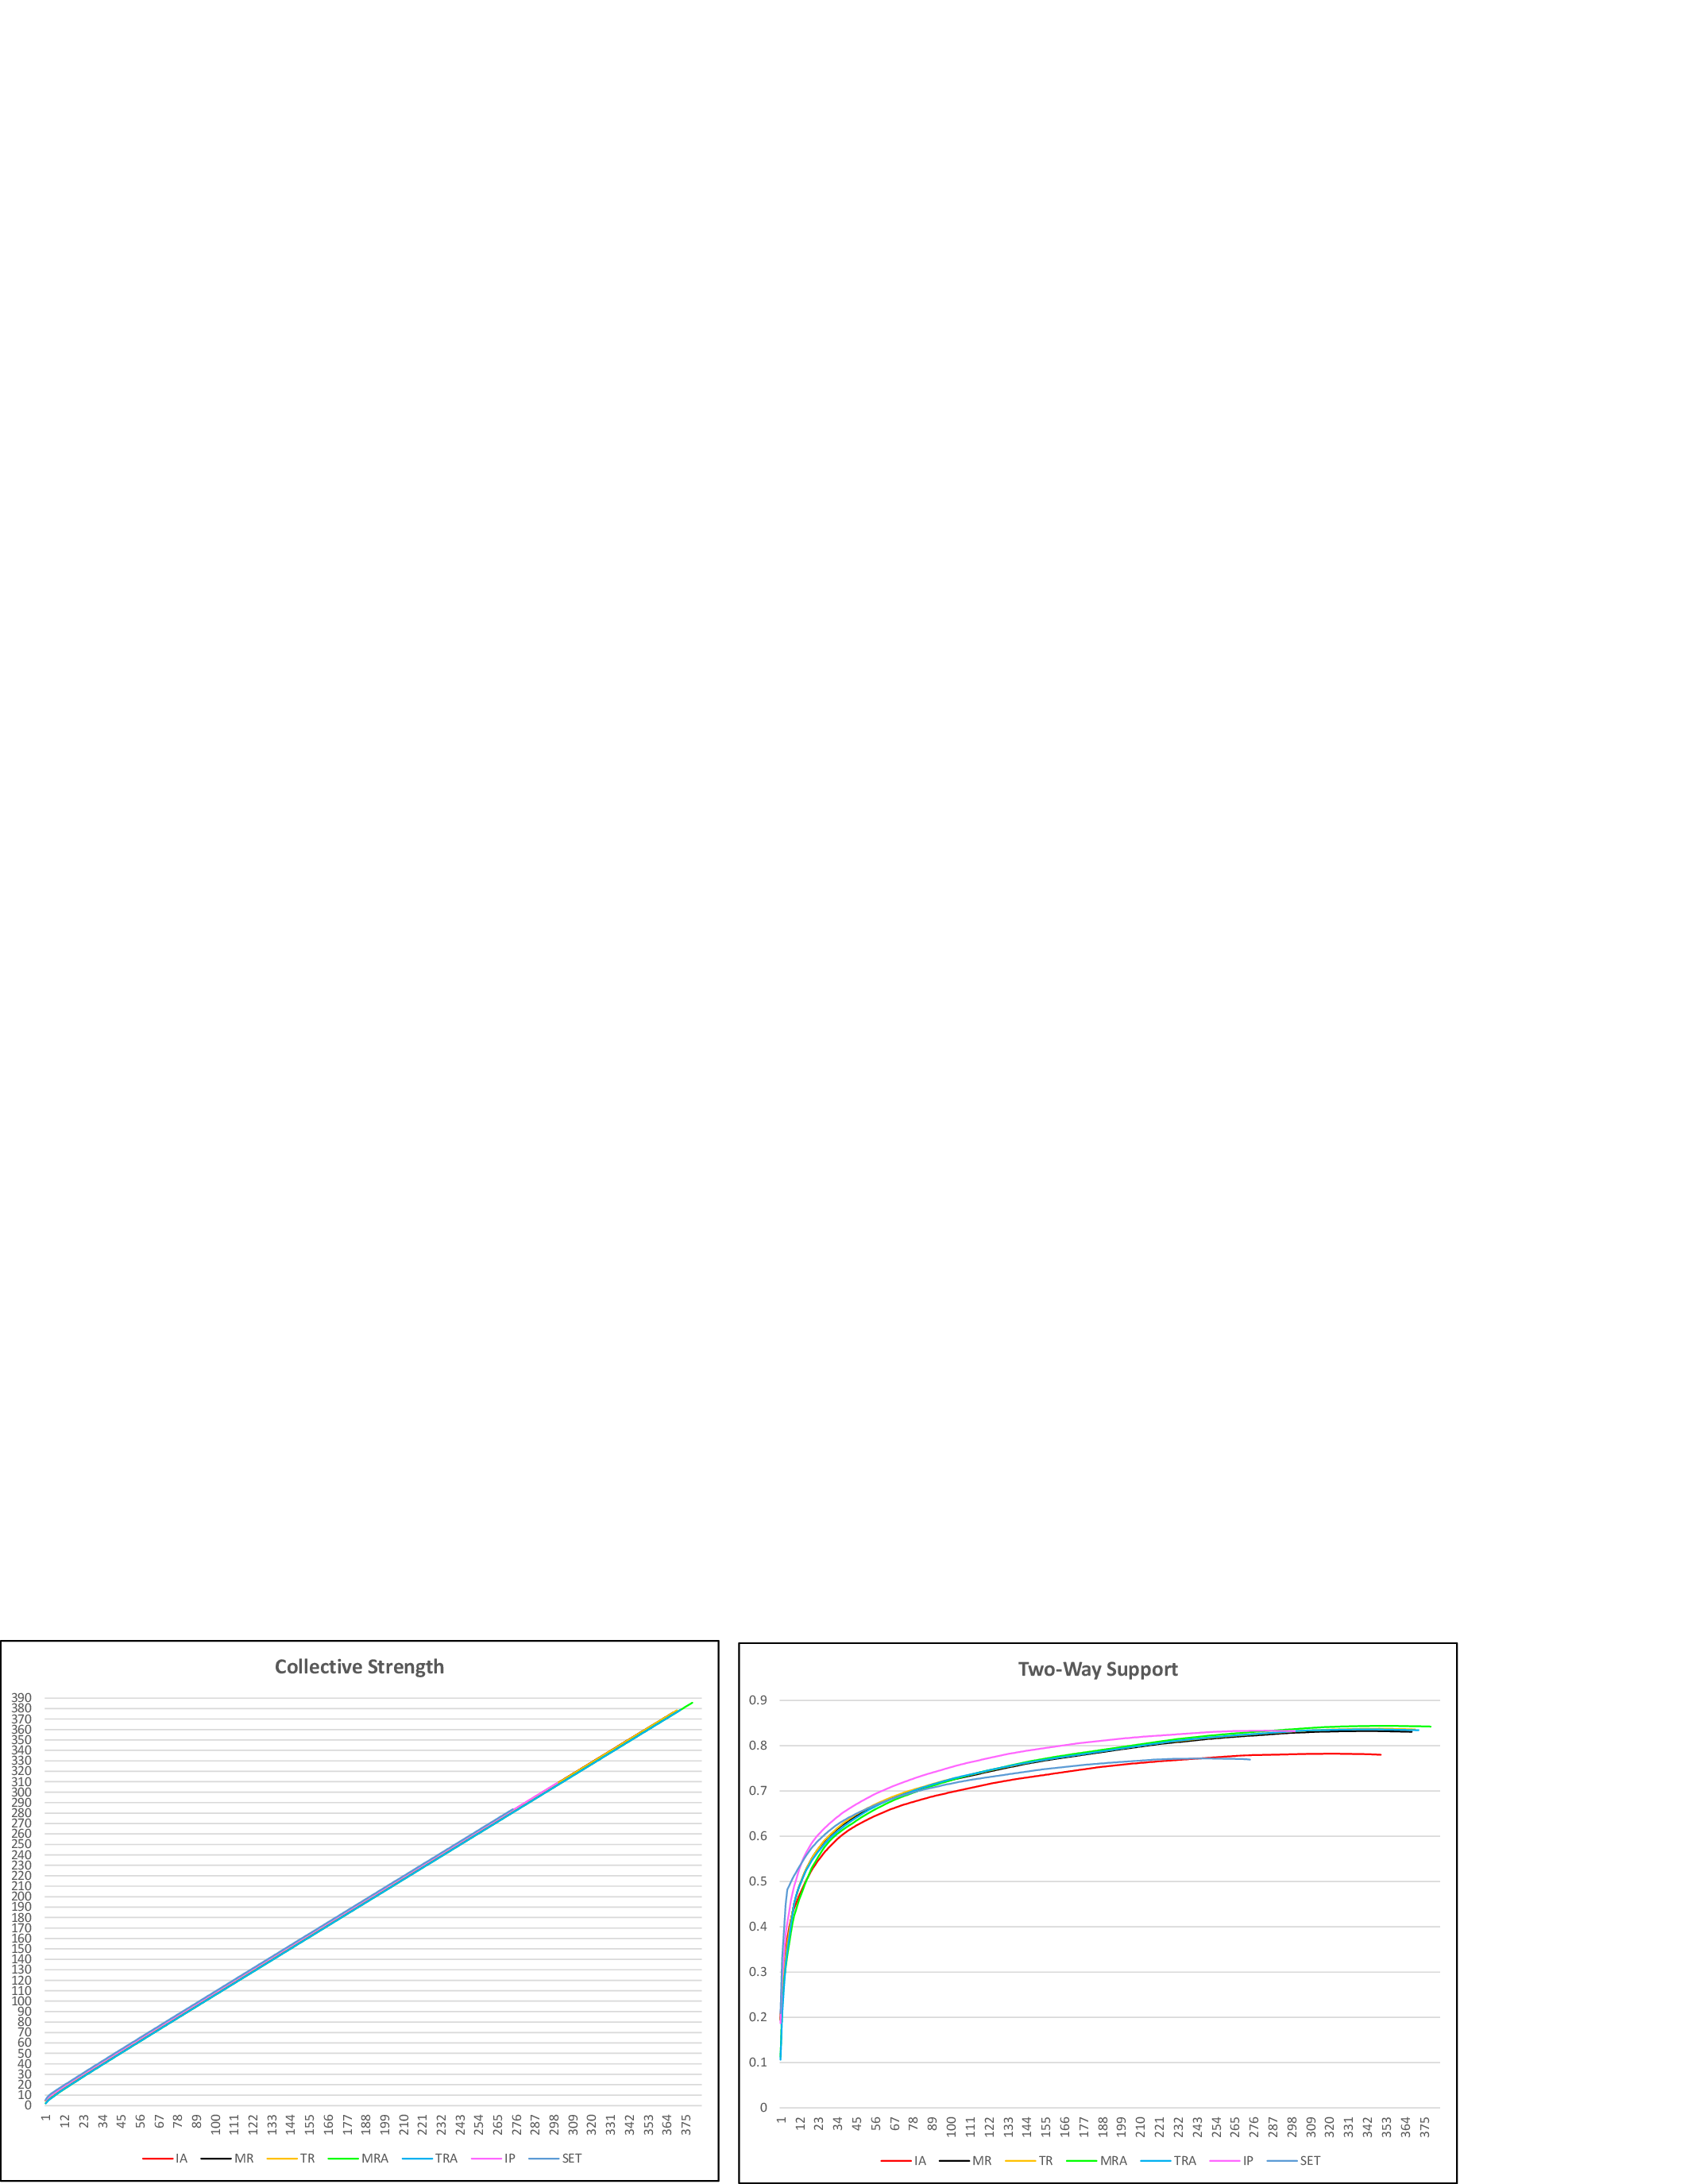}}
	\caption{Insurance1 dataset - Collective Strength and Two-Way Support}
	\label{fig:insurance1-interest2}
\end{figure}

\begin{figure}[!htb]
	\centering
	{\includegraphics[width=\textwidth]{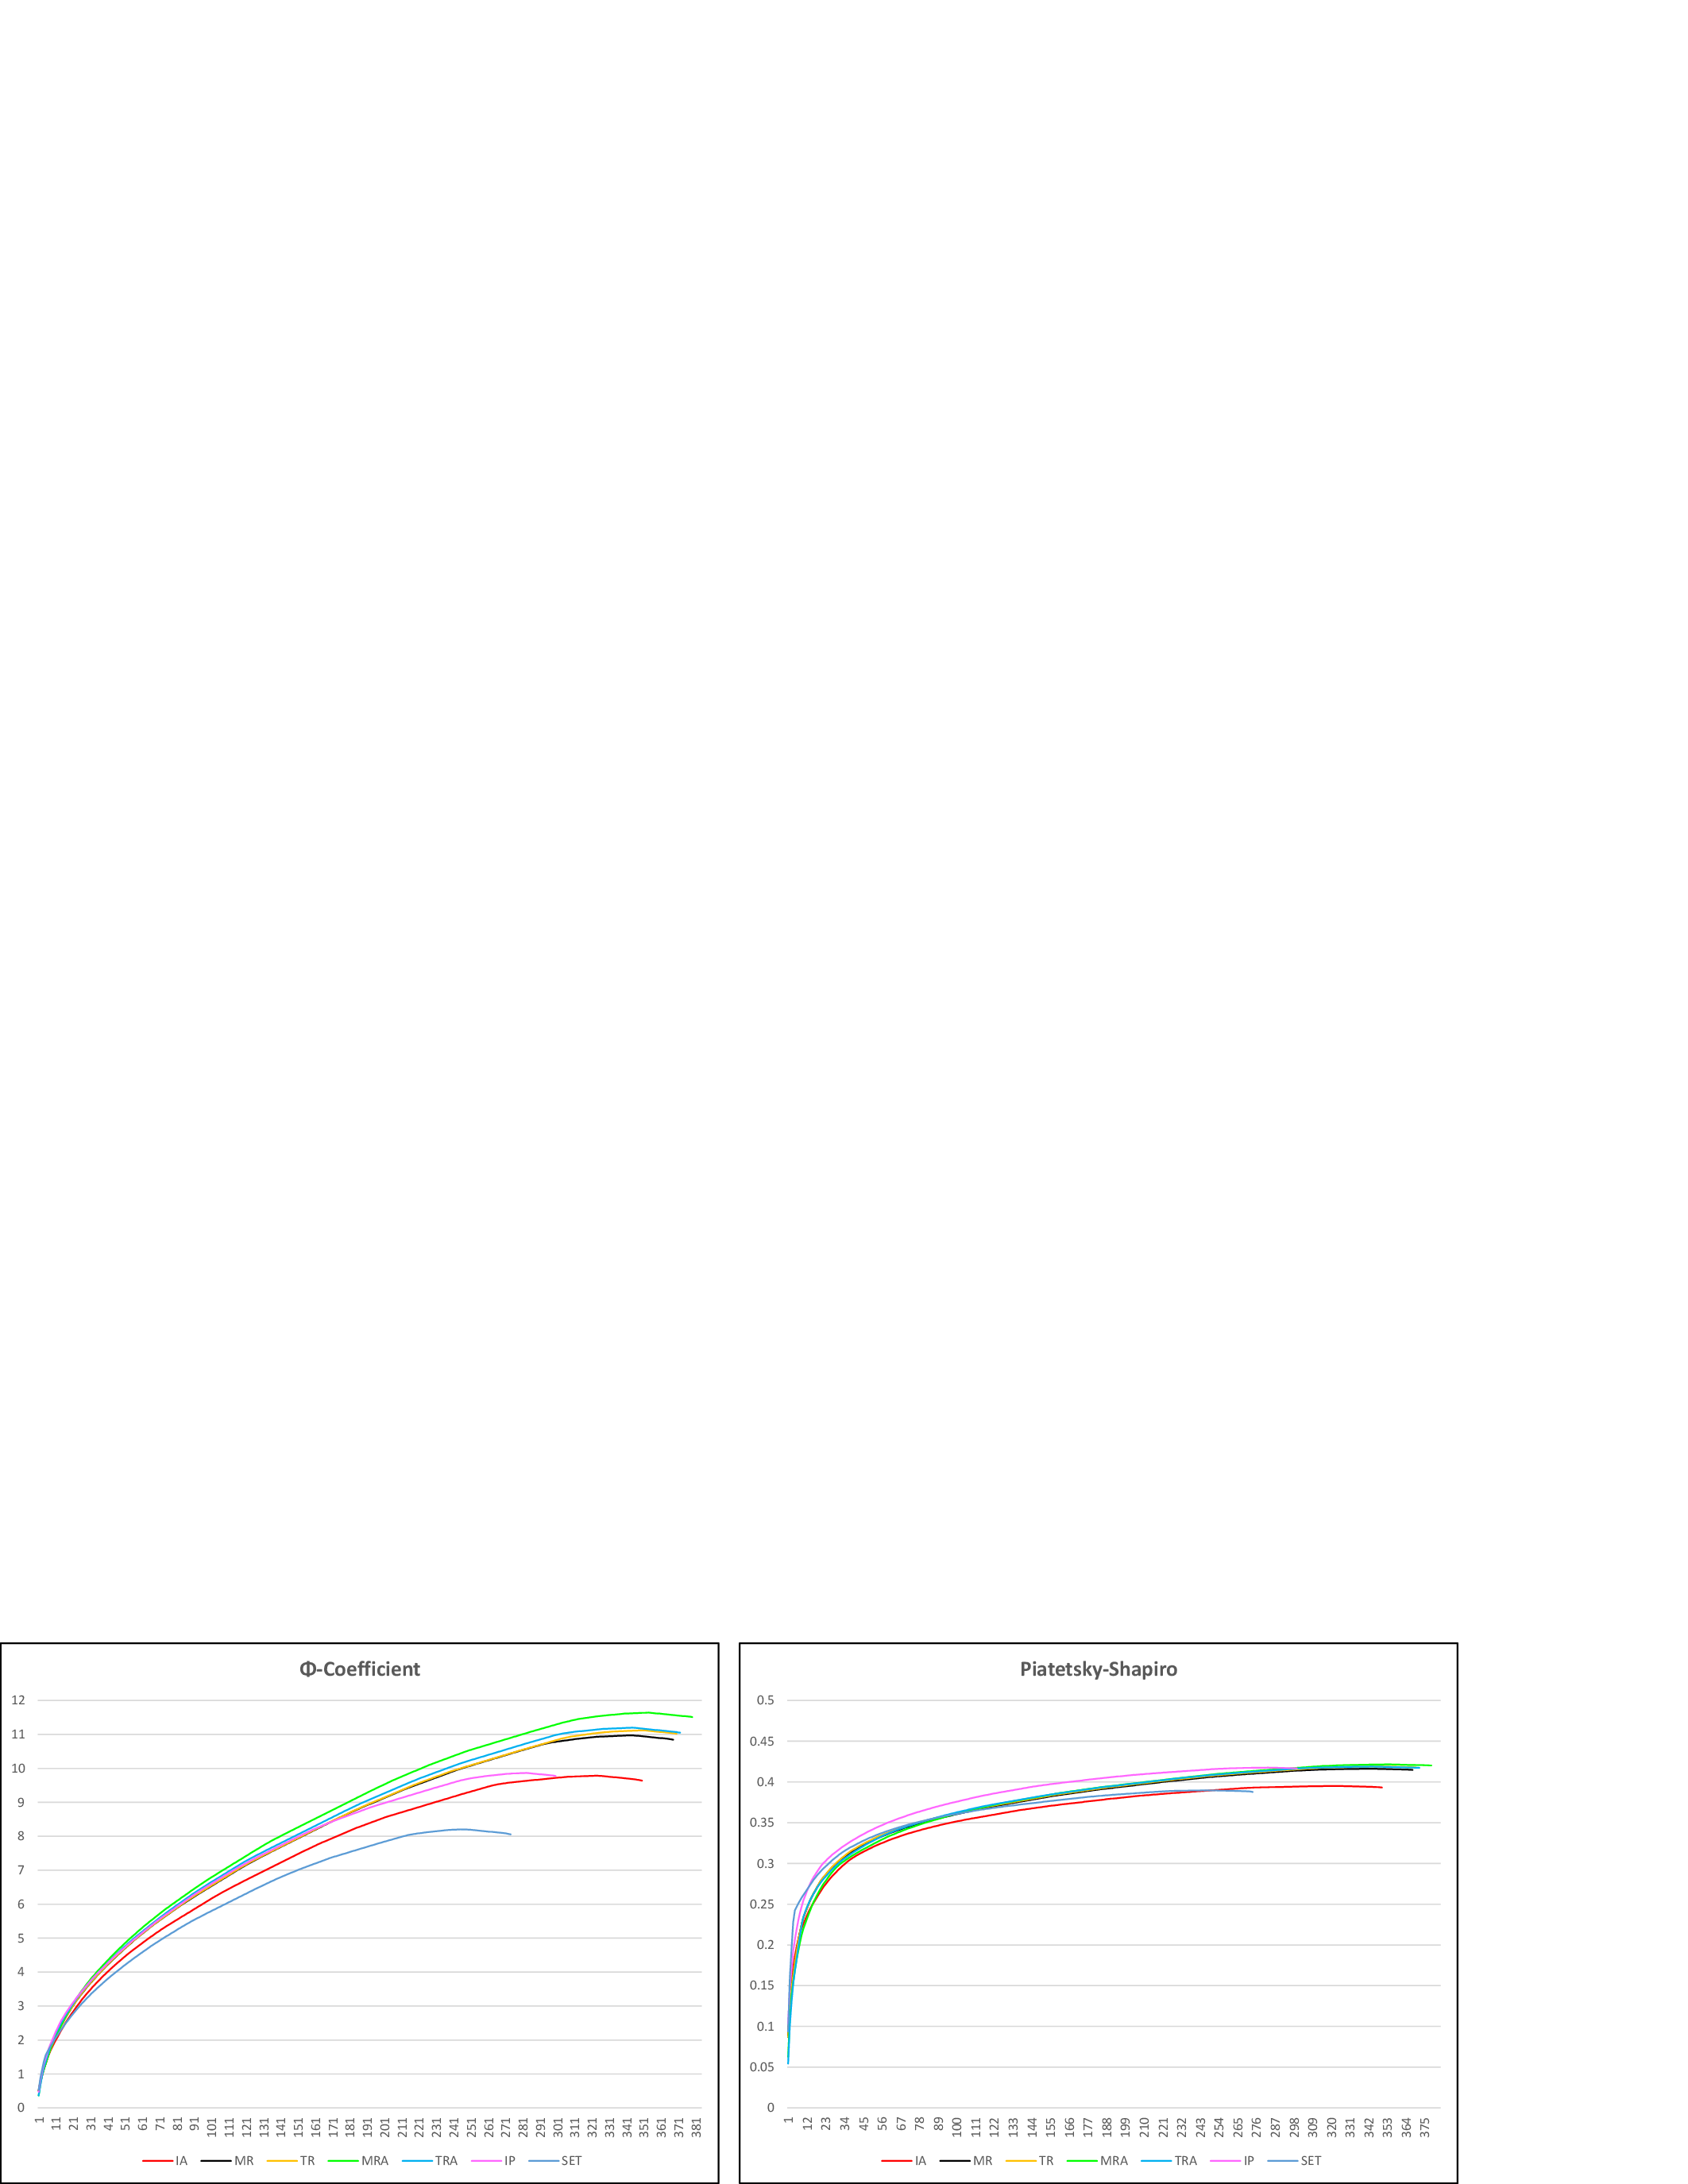}}
	\caption{Insurance1 dataset - \(\phi\)-Coefficient and Piatetsky-Shapiro}
	\label{fig:insurance1-interest3}
\end{figure}
	
\begin{figure}[!htb]	
	{\includegraphics[width=\textwidth]{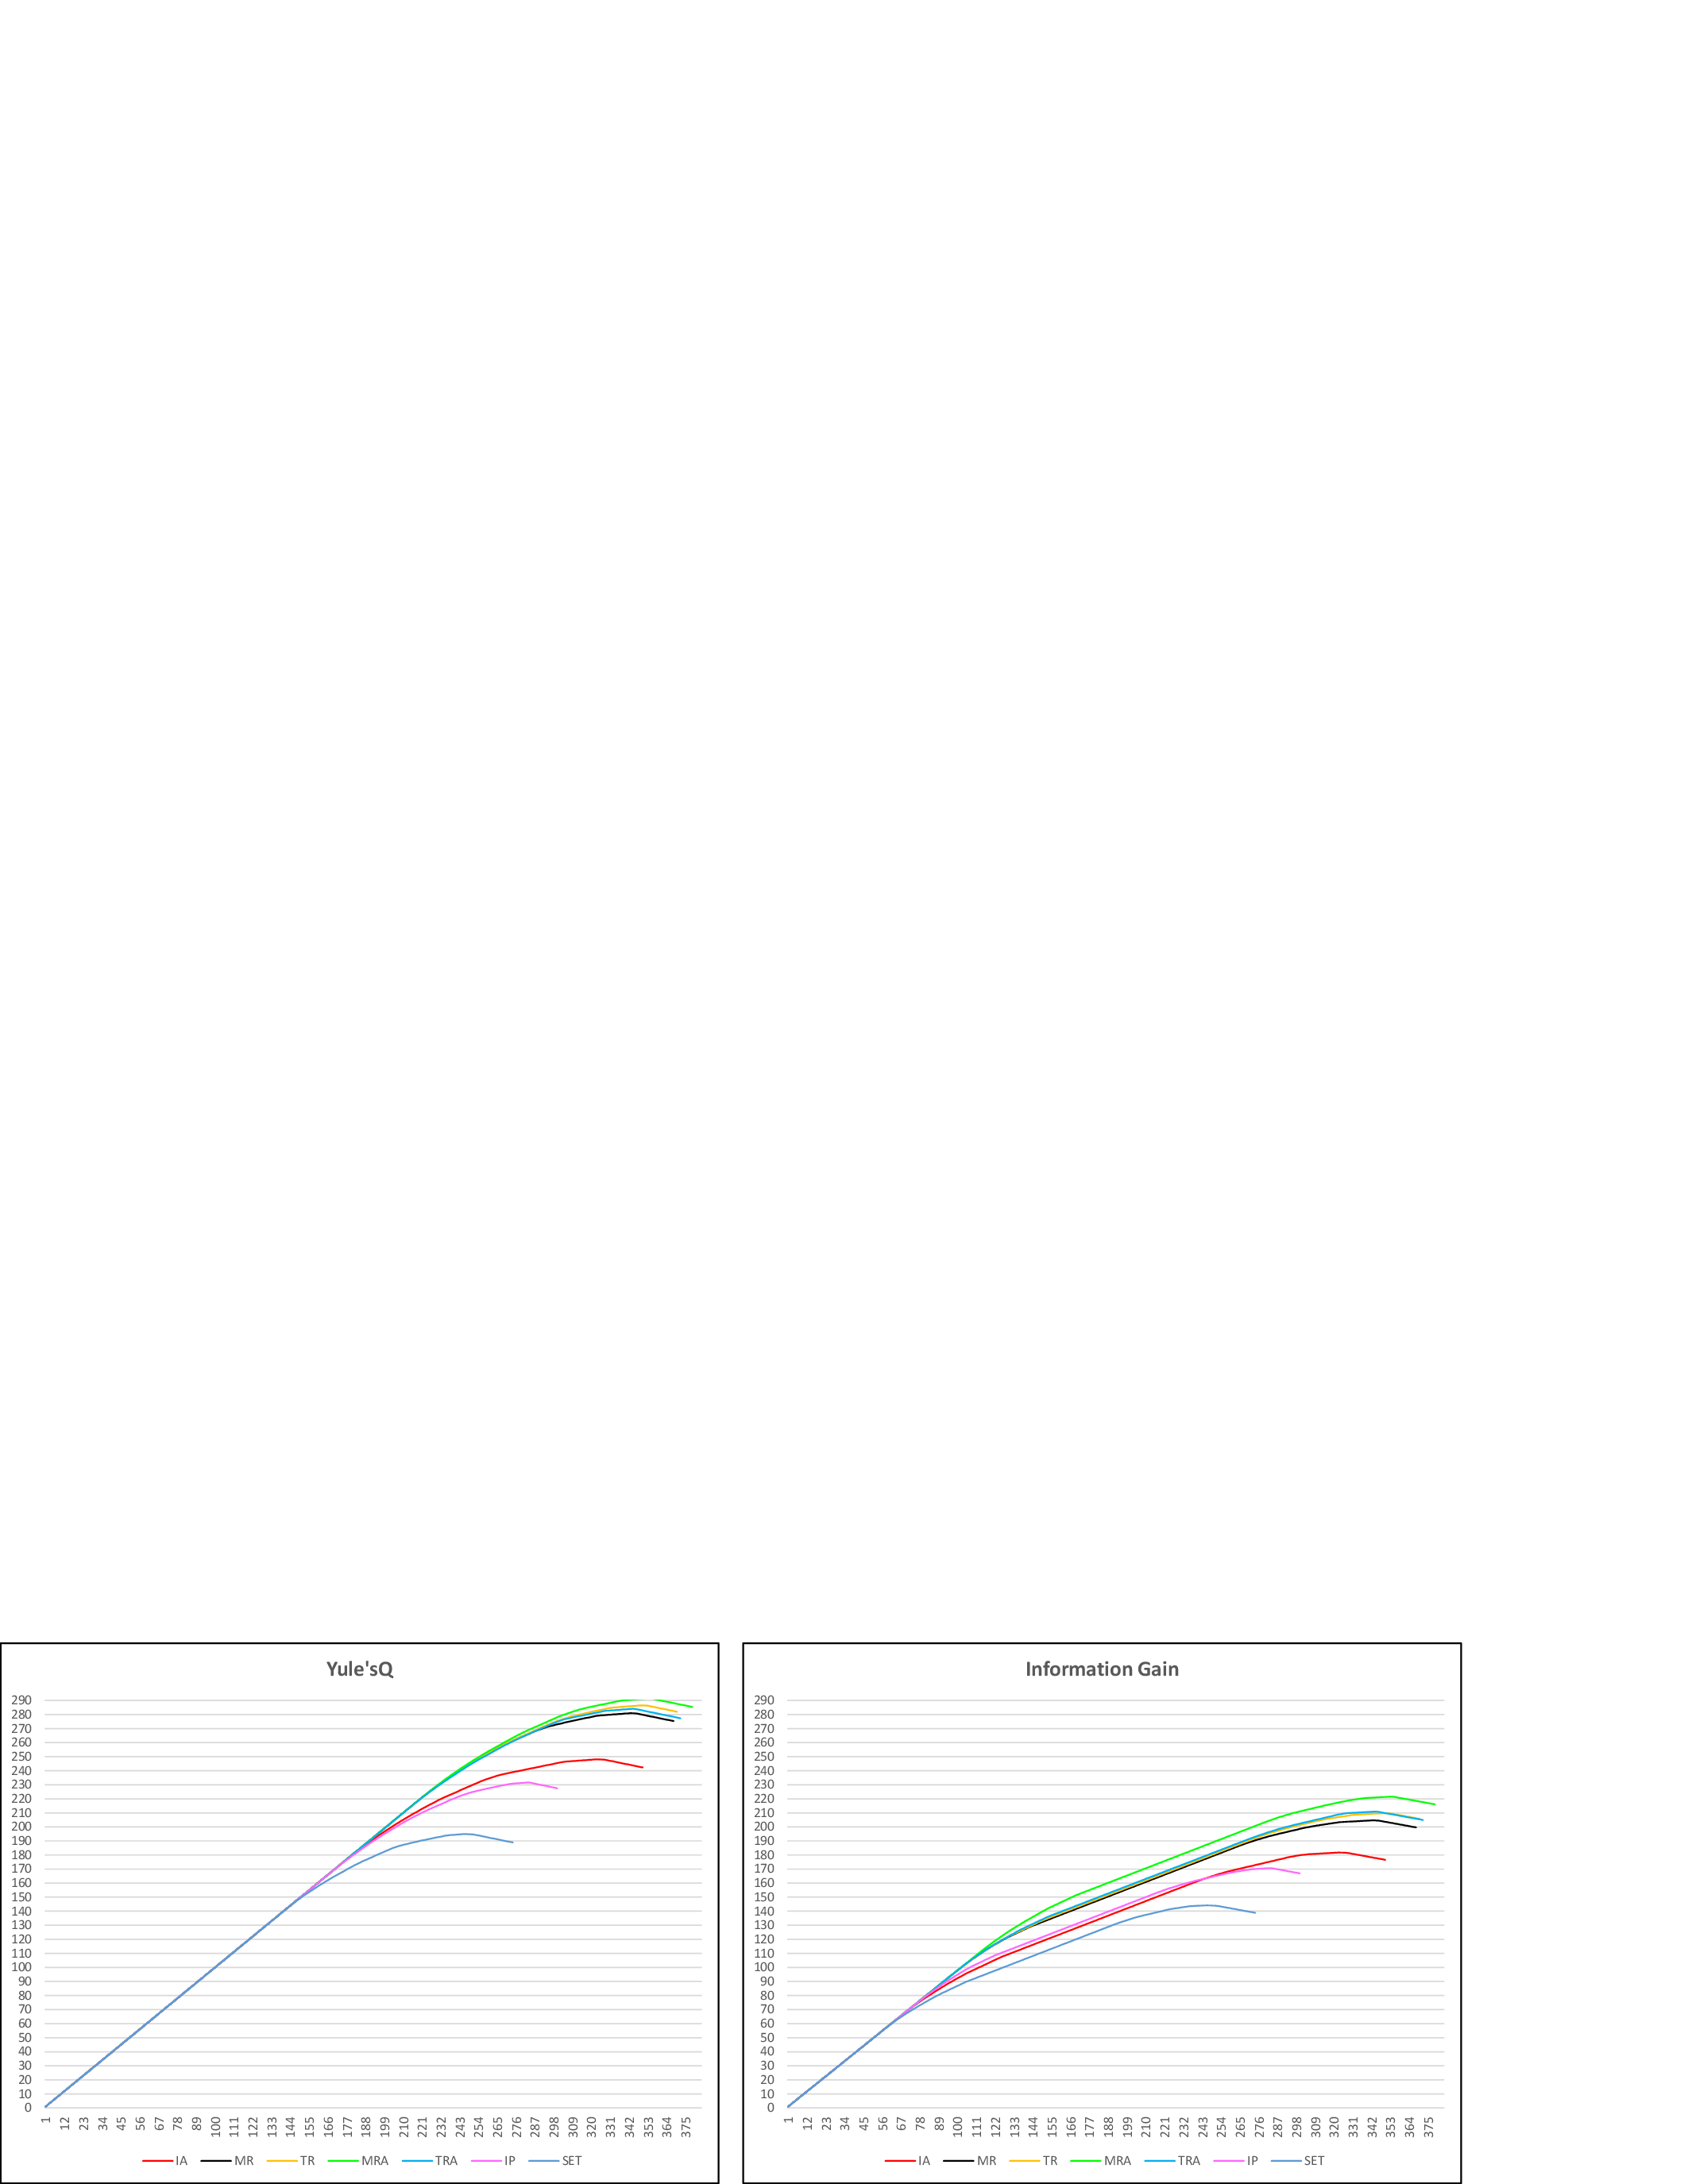}}
	\caption{Insurance1 dataset - Yule's Q and Information Gain}
	\label{fig:insurance1-interest4}
\end{figure}
\FloatBarrier

\clearpage
\subsection{Insurance2 Dataset}

\FloatBarrier
\begin{figure}[!htb]
	\centering
	
	{\includegraphics[width=\textwidth]{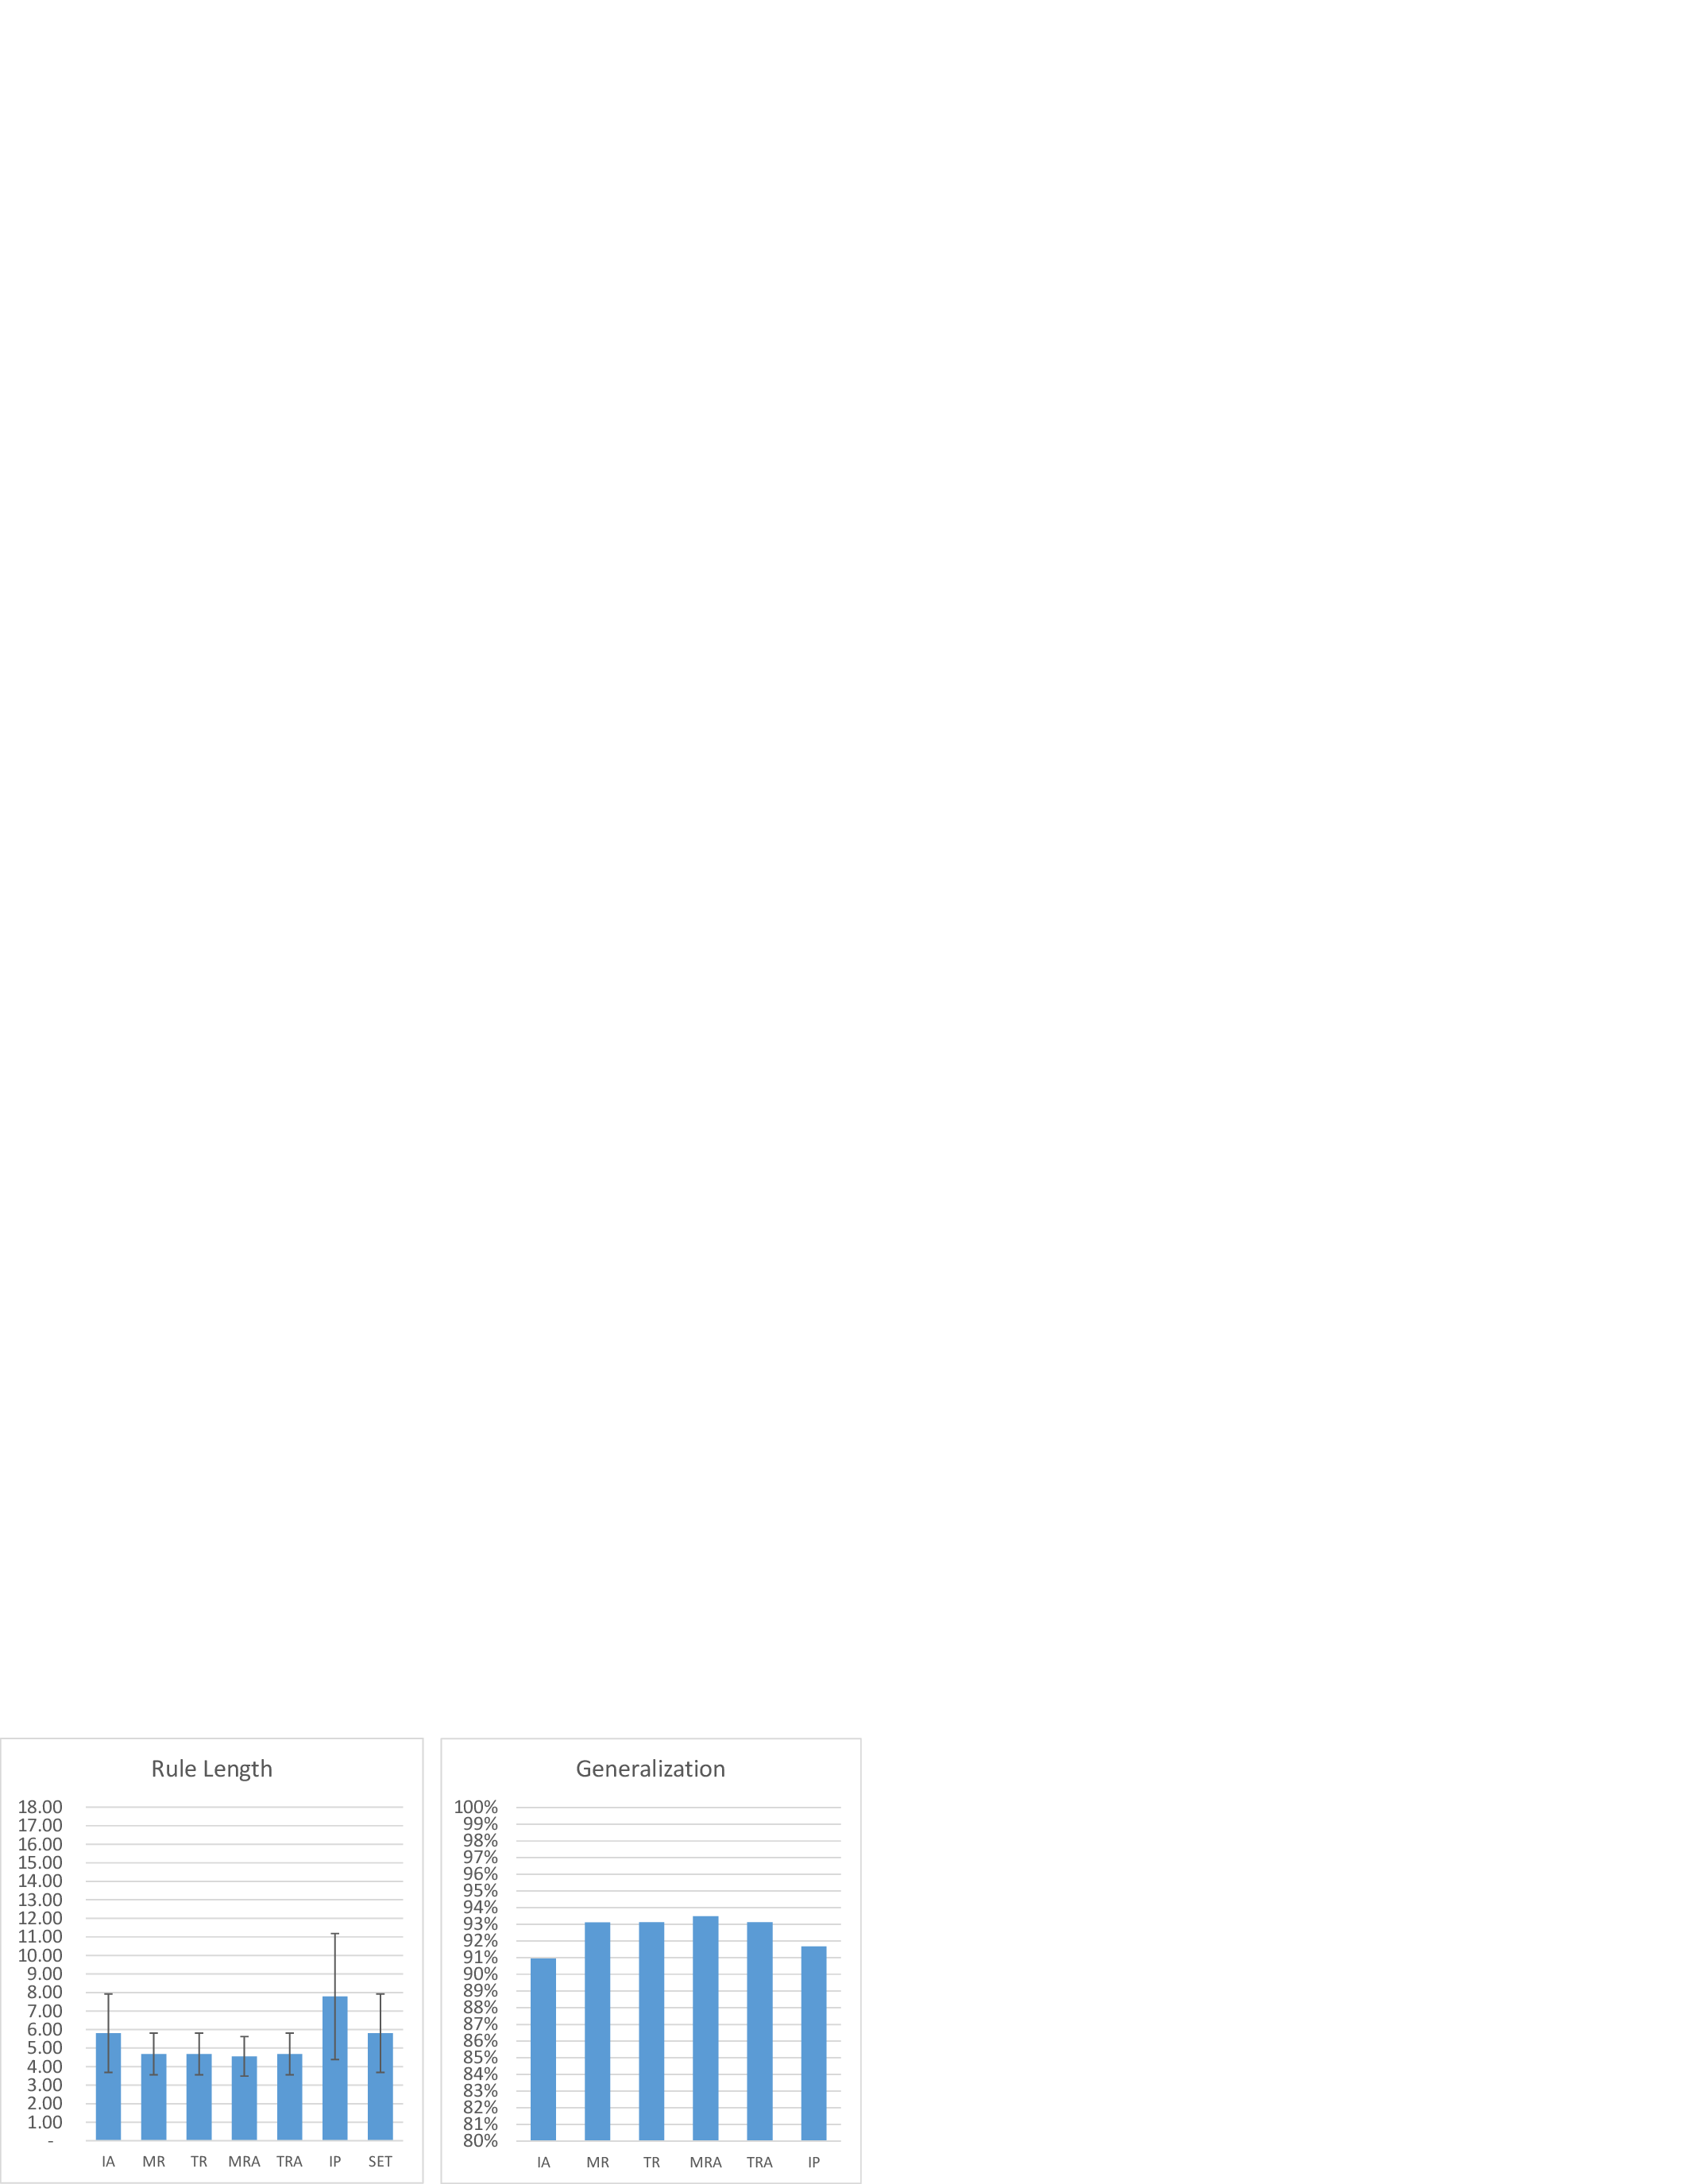}}
	\caption{Insurance2 dataset - Rule Length \& \%Generalization}
	\label{fig:insurance2-interest5}
\end{figure}
	
\begin{figure}[!htb]
	{\includegraphics[width=\textwidth]{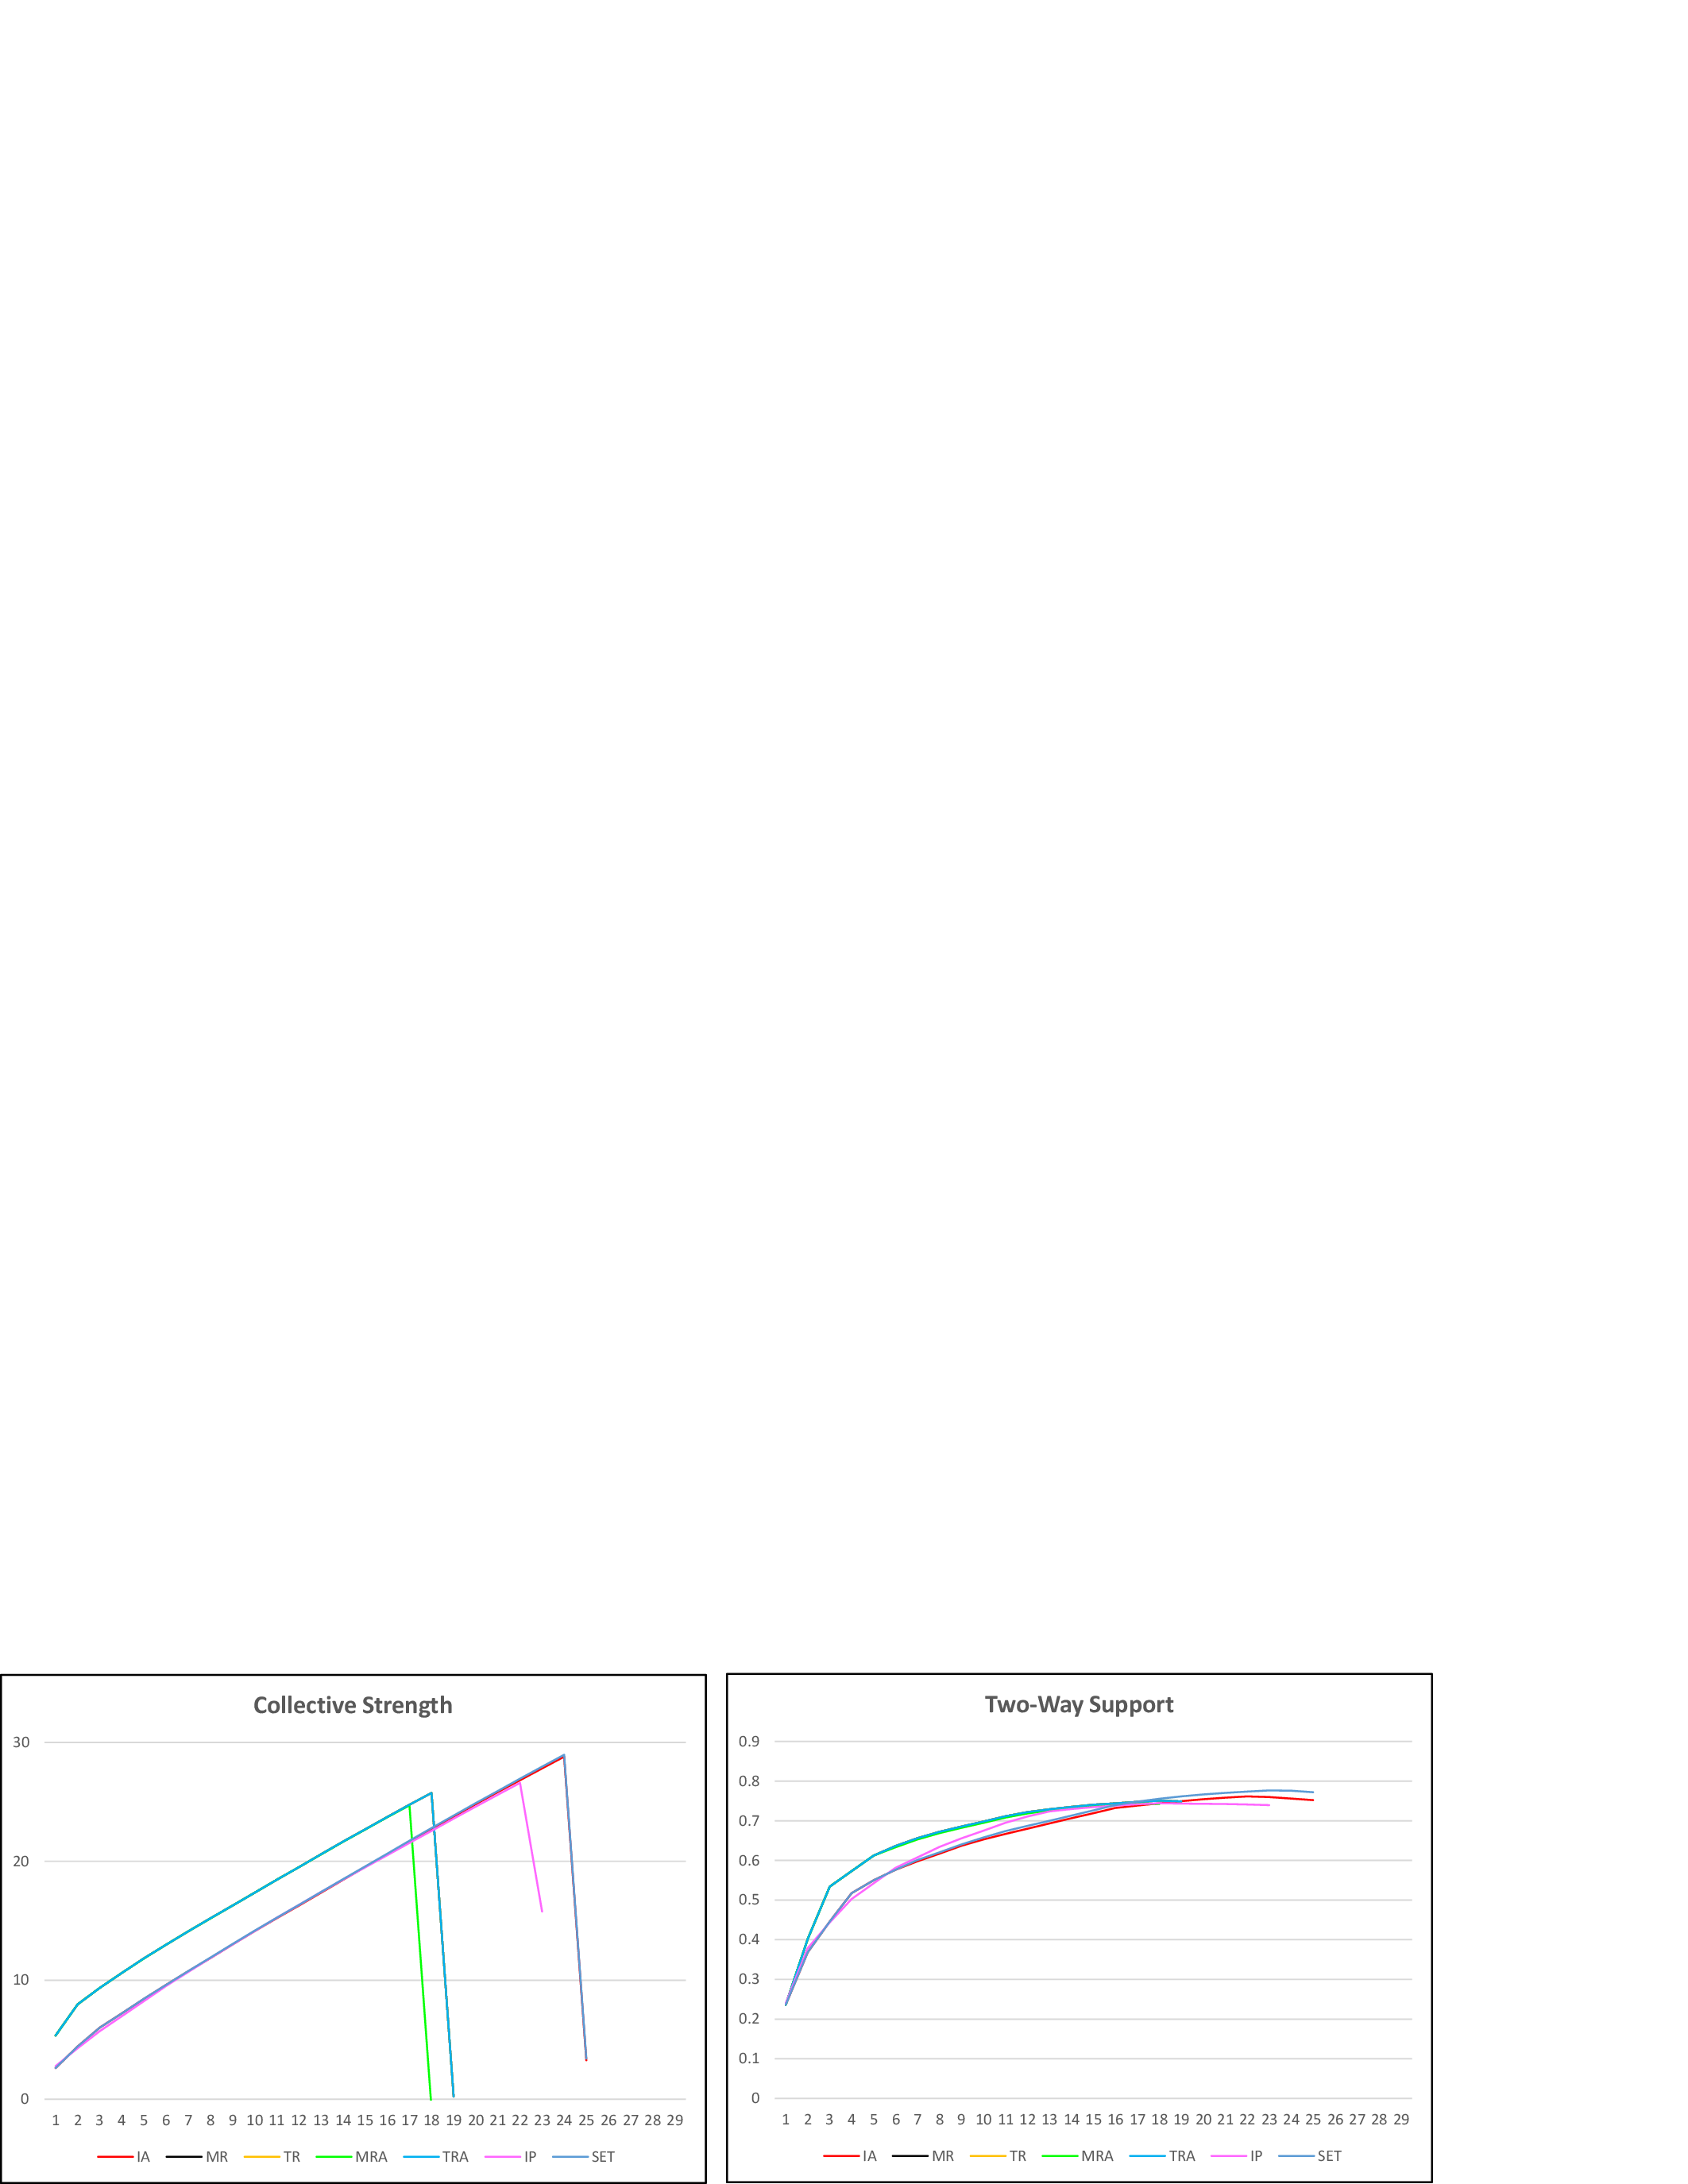}}
	\caption{Insurance2 dataset - Collective Strength and Two-Way Support}
	\label{fig:insurance2-interest2}
\end{figure}

\begin{figure}[!htb]
	\centering
	{\includegraphics[width=\textwidth]{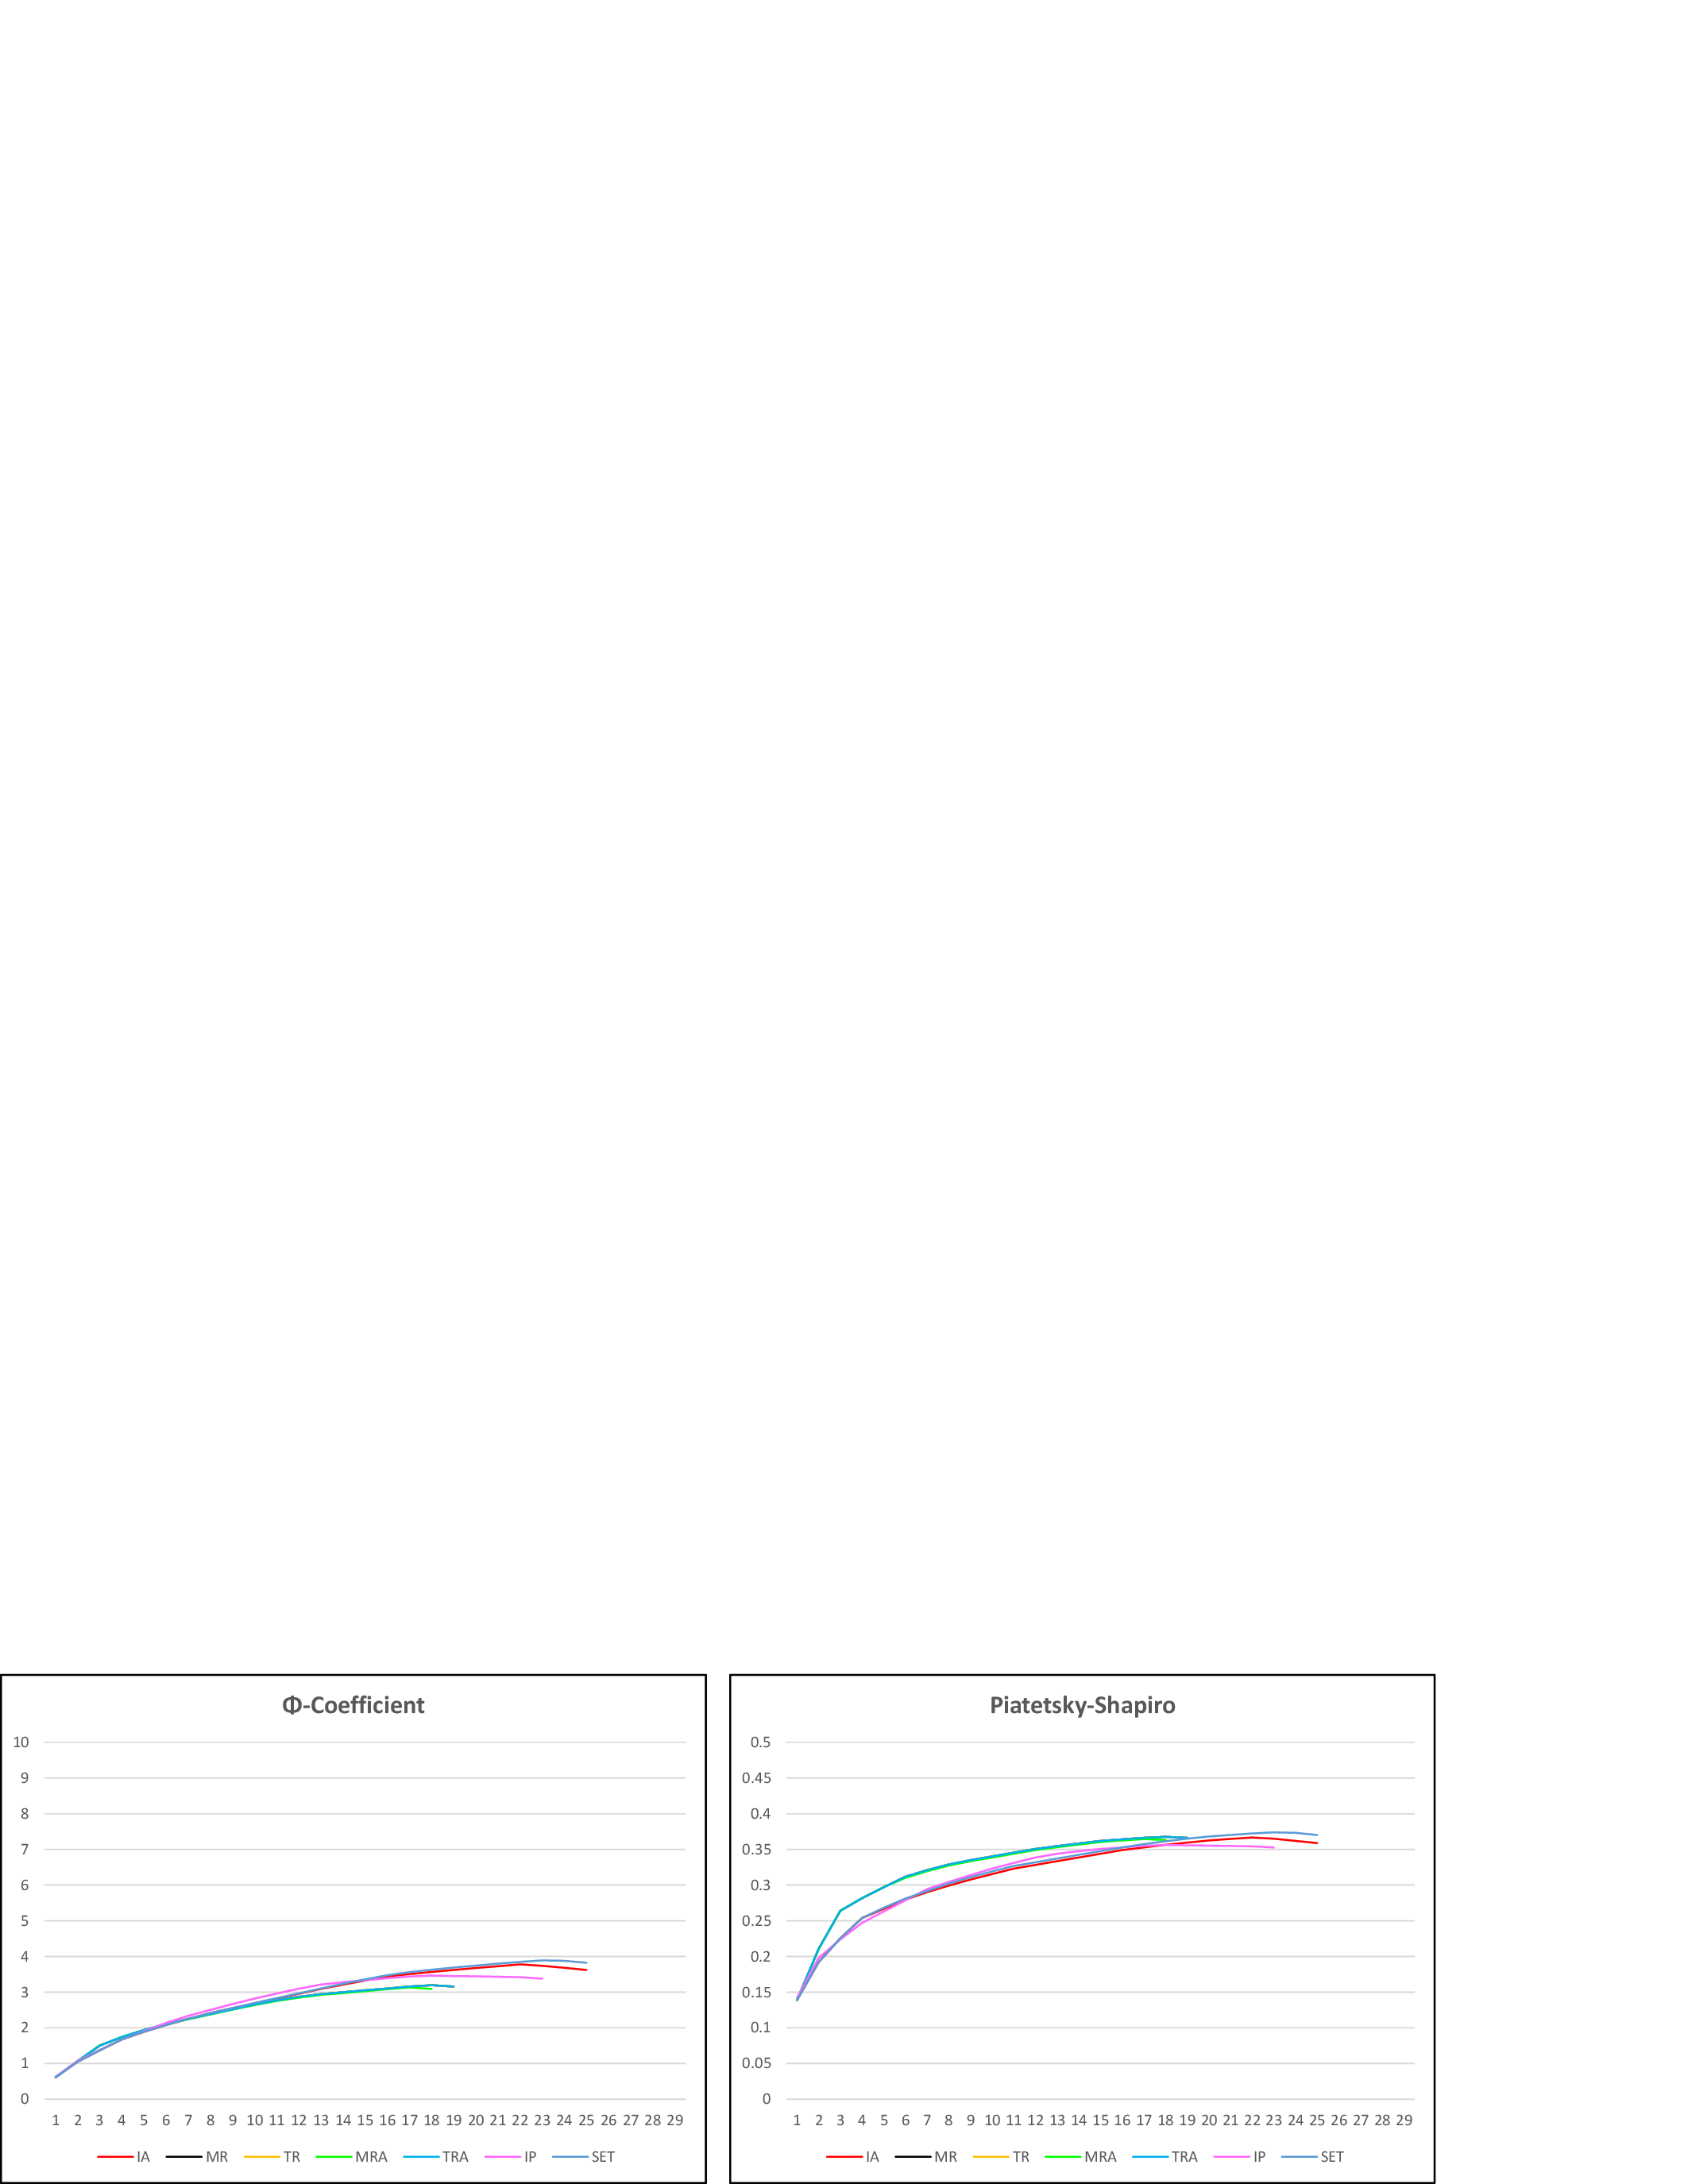}}
	\caption{Insurance2 dataset - \(\phi\)-Coefficient and Piatetsky-Shapiro}
	\label{fig:insurance2-interest3}
\end{figure}
	
\begin{figure}[!htb]	
	{\includegraphics[width=\textwidth]{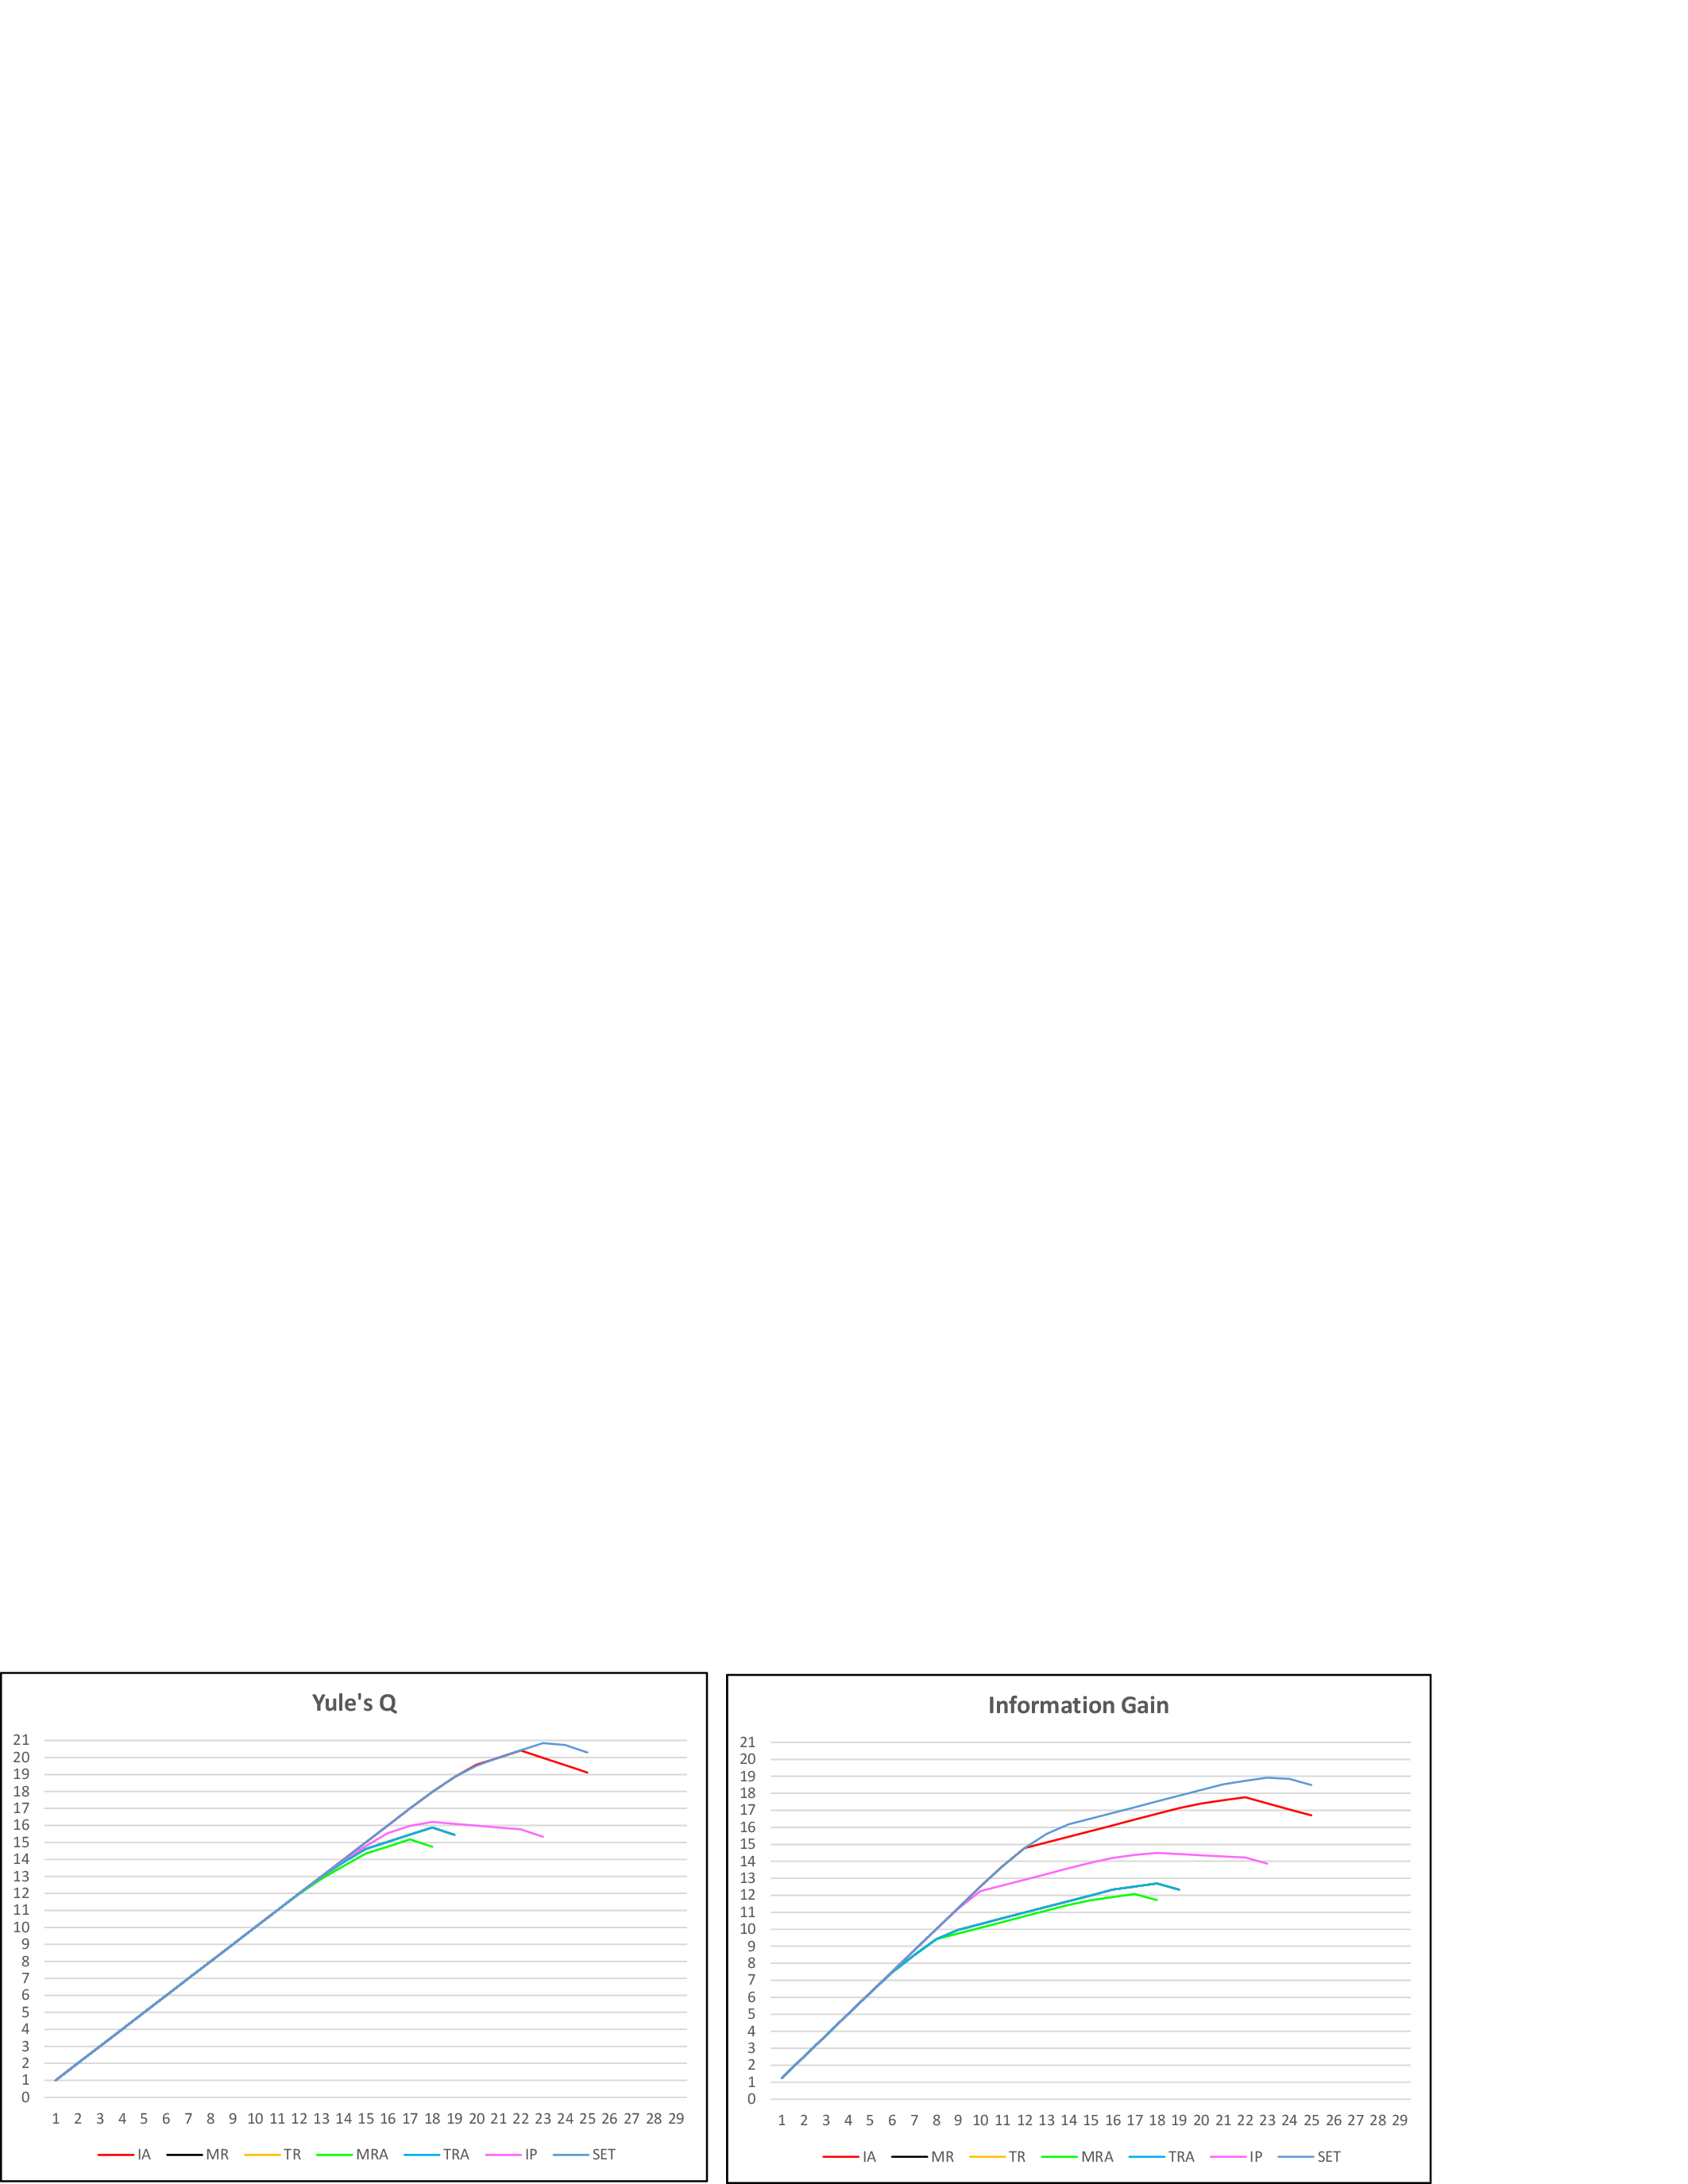}}
	\caption{Insurance2 dataset - Yule's Q and Information Gain}
	\label{fig:insurance2-interest4}
\end{figure}
\FloatBarrier
